# Supplementary material for: Accurate absolute core-electron binding energies of molecules, solids and surfaces from first-principles calculations
Source: arXiv:1904.04823 ancillary file (2019-04-09)
Supplement: Supplementary file 1 [file Supplementary_information_for_SCAN_BE_paper.pdf]

# Supplementary Information for "Accurate absolute core-electron binding energies of molecules, solids, and surfaces from first-principles calculations"

J. Matthias Kahk† and Johannes Lischner‡

†*Department of Materials, Imperial College London, London SW7 2AZ, United Kingdom*

‡*Department of Physics and Department of Materials, and the Thomas Young Centre for Theory and Simulation of Materials, Imperial College London, London SW7 2AZ, United Kingdom*

E-mail: j.lischner@imperial.ac.uk

## Contents

Core electron binding energies in free molecules – full details.....2
Comparison with the molecular dataset from PRL 118, 026401 (2017).....9
Basis sets used in the molecular calculations.....10
Numerical basis sets with additional core functions.....10
Standard numerical basis sets.....20
u-pcJ-3 basis sets.....35
A comparison of the results obtained using different basis sets.....47
The geometries of the clusters used for calculating core electron binding energies of adsorbates and solids.....48
Basis sets used in the cluster calculations.....74
Relaxed lattice parameters of bulk Be and Mg obtained using the SCAN functional and numerical "tight" basis sets.....83

# Core electron binding energies in free molecules – full details

Supplementary Table 1: a dataset of 103 experimental and calculated core electron binding energies from free molecules.

Most of the experimental values are taken from the compilation of binding energies from gas phase photoelectron spectra by Jolly et al. (At. Data Nucl. Data Tables **31**, 433 (1984)). The references to the original experimental measurements are given in the table below. In addition, some B 1s binding energies from reference [25] have been included that are not contained in the compilation, and furthermore, all of the "weighted average" core electron binding energies from reference [28] have been used "as is".

Amongst the 2p binding energies, the weighted average of the spin-orbit doublet has been used for Si 2p, as most experimental results only report this average value. For P 2p, S 2p and Cl 2p, the $2p_{3/2}$ binding energy is used.

* Denotes that the value has been obtained by subtracting 1/3 of the 2p spin-orbit splitting from the published binding energy that refers to an average of the 2p spin-orbit doublet. The subtracted values are 0.29 eV for P 2p, 0.39 eV for S 2p, and 0.53 eV for Cl 2p.

When two experimental references are given for one binding energy, it means that a published value from the second one has been used for calibrating the binding energy scale in the first.

All values are given in eV.

| Core level | Expt. $E_B$ | Reference | Average Expt $E_B$ | Calculated $E_B$ | Error (Theory - Expt) | Abs. Error \|Theory - Expt\| |
|---|---|---|---|---|---|---|
| $Si(CH_3)_4$ Si 2p | 105.96 | [1] | 105.97 | 105.76 | -0.21 | 0.21 |
| | 106.02 | [2] | | | | |
| | 105.94 | [3] | | | | |
| $Si(CH_3)_3CH_2Cl$ Si 2p | 106.31 | [4] | 106.27 | 106.28 | 0.01 | 0.01 |
| | 106.23 | [3] | | | | |
| $(Si(CH_3)_3)_2O$ Si 2p | 106.50 | [4] | 106.54 | 106.67 | 0.13 | 0.13 |
| | 106.56 | [5] | | | | |
| | 106.57 | [6] | | | | |
| $SiH_3CH_3$ Si 2p | 106.82 | [1] | 106.89 | 106.81 | -0.08 | 0.08 |
| | 106.95 | [2] | | | | |
| $Si(CH_3)_3Cl$ Si 2p | 106.95 | [4] | 107.00 | 107.07 | 0.07 | 0.07 |
| | 107.06 | [3] | | | | |
| $SiH_4$ Si 2p | 107.31 | [2] | 107.30 | 107.25 | -0.05 | 0.05 |
| | 107.28 | [1] | | | | |
| $Si(CH_3)_2Cl_2$ Si 2p | 108.09 | [4] | 108.10 | 108.27 | 0.17 | 0.17 |
| | 108.10 | [3] | | | | |
| $SiCl_3CH_3$ Si 2p | 109.16 | [4] | 109.19 | 109.40 | 0.21 | 0.21 |
| | 109.25 | [7] | | | | |
| | 109.15 | [3] | | | | |
| $SiCl_4$ Si 2p | 110.39 | [1] | 110.24 | 110.44 | 0.20 | 0.20 |
| | 110.17 | [3] | | | | |
| | 110.17 | [4] | | | | |
| $SiF_4$ Si 2p | 111.79 | [1] | 111.75 | 111.00 | -0.75 | 0.75 |
| | 111.70 | [3] | | | | |

| Core level | Expt. $E_B$ | Reference | Average Expt $E_B$ | Calculated $E_B$ | Error (Theory - Expt) | Abs. Error \|Theory - Expt\| |
|---|---|---|---|---|---|---|
| $P(CH_3)_3$ P $2p_{3/2}$ | 135.93 | [8] | 135.96 | 135.69 | -0.27 | 0.27 |
| | 136.00 | [9,10] | | | | |
| | 135.96* | [11] | | | | |
| $PH_3$ P $2p_{3/2}$ | 137.02 | [8] | 137.04 | 136.95 | -0.09 | 0.09 |
| | 137.01* | [12] | | | | |
| | 137.06* | [13,11] | | | | |
| | 137.08 | [9,10] | | | | |
| $P(OCH_3)_3$ P $2p_{3/2}$ | 138.32 | [14] | 138.29 | 137.92 | -0.37 | 0.37 |
| | 138.25* | [11] | | | | |
| $P(CF_3)_3$ P $2p_{3/2}$ | 138.85 | [14] | 138.81 | 138.13 | -0.68 | 0.68 |
| | 138.76* | [11] | | | | |
| $PCl_3$ P $2p_{3/2}$ | 139.75 | [10] | 139.81 | 139.79 | -0.02 | 0.02 |
| | 139.86* | [13,11] | | | | |
| $PSCl_3$ P $2p_{3/2}$ | 140.60 | [8] | 140.7 | 140.56 | -0.14 | 0.14 |
| | 140.86* | [13] | | | | |
| | 140.63* | [11] | | | | |
| $POCl_3$ P $2p_{3/2}$ | 141.02 | [10] | 141.04 | 140.92 | -0.12 | 0.12 |
| | 141.06* | [13,11] | | | | |
| $PF_3$ P $2p_{3/2}$ | 141.78 | [10] | 141.77 | 141.14 | -0.63 | 0.63 |
| | 141.76* | [13,11] | | | | |
| $POF_3$ P $2p_{3/2}$ | 143.00 | [10] | 142.98 | 142.37 | -0.61 | 0.61 |
| | 142.96 | [13,11] | | | | |
| $PSCl_3$ S $2p_{3/2}$ | 168.87 | [8] | 168.84 | 169.10 | 0.26 | 0.26 |
| | 168.81* | [15] | | | | |
| $S(CH_3)_2$ S $2p_{3/2}$ | 169.09 | [7] | 169.06 | 169.02 | -0.04 | 0.04 |
| | 169.02 | [9,16] | | | | |
| $CH_3SH$ S $2p_{3/2}$ | 169.28 | [6] | 169.4 | 169.55 | 0.15 | 0.15 |
| | 169.51 | [9,16] | | | | |
| $CS_2$ S $2p_{3/2}$ | 169.80 | [16] | 169.92 | 170.01 | 0.09 | 0.09 |
| | 170.03 | [17] | | | | |
| $C_4H_4S$ (thiophene) S $2p_{3/2}$ | 169.90 | [18] | 169.97 | 169.93 | -0.04 | 0.04 |
| | 170.04 | [19] | | | | |
| $H_2S$ S $2p_{3/2}$ | 170.20 | [16] | 170.32 | 170.28 | -0.04 | 0.04 |
| | 170.44 | [17] | | | | |
| OCS S $2p_{3/2}$ | 170.60 | [20] | 170.69 | 170.75 | 0.06 | 0.06 |
| | 170.77 | [17] | | | | |
| $SO_2$ S $2p_{3/2}$ | 174.80 | [16] | 174.82 | 174.75 | -0.07 | 0.07 |
| | 174.81 | [5] | | | | |
| | 174.84 | [17] | | | | |

| Core level | Expt. $E_B$ | Reference | Average Expt $E_B$ | Calculated $E_B$ | Error (Theory - Expt) | Abs. Error \|Theory - Expt\| |
|---|---|---|---|---|---|---|
| | 180.28 | [17] | | | | |
| $SF_6$ S $2p_{3/2}$ | 180.40 | [16] | 180.29 | 179.45 | -0.84 | 0.84 |
| | 180.20 | [21] | | | | |
| $BH_3CO$ B 1s | 195.20 | [22,23] | 195.15 | 194.96 | -0.19 | 0.19 |
| | 195.10 | [24] | | | | |
| $B_2H_6$ B 1s | 196.50 | [23] | 196.50 | 196.40 | -0.10 | 0.10 |
| | 196.50 | [22,23] | | | | |
| $BI_3$ B 1s | 197.80 | [23] | 197.86 | 197.68 | -0.18 | 0.18 |
| | 197.92 | [25] | | | | |
| BBr3 B 1s | 199.00 | [23] | 198.90 | 198.64 | -0.26 | 0.26 |
| | 198.80 | [25] | | | | |
| BCl3 B 1s | 199.80 | [23] | 199.89 | 199.92 | 0.03 | 0.03 |
| | 199.98 | [25] | | | | |
| $BF_3$ B 1s | 202.80 | [23] | 202.83 | 201.79 | -1.04 | 1.04 |
| | 202.85 | [25] | | | | |
| $CH_3CH_2Cl$ Cl $2p_{3/2}$ | 205.92 | [26] | 205.96 | 205.73 | -0.23 | 0.23 |
| | 206.00 | [27] | | | | |
| $PCl_3$ Cl $2p_{3/2}$ | 206.42 | [10] | 206.24 | 206.32 | 0.08 | 0.08 |
| | 206.07* | [15] | | | | |
| $CH_3Cl$ Cl $2p_{3/2}$ | 206.24 | [1] | 206.25 | 206.17 | -0.08 | 0.08 |
| | 206.26 | [26] | | | | |
| $SiCl_3CH_3$ Cl $2p_{3/2}$ | 206.33 | [7] | 206.39 | 206.22 | -0.17 | 0.17 |
| | 206.44 | [4] | | | | |
| $CH_2Cl_2$ Cl $2p_{3/2}$ | 206.62 | [26] | 206.66 | 206.46 | -0.20 | 0.20 |
| | 206.70 | [27] | | | | |
| $CHCl_3$ Cl $2p_{3/2}$ | 206.86 | [26] | 206.83 | 206.68 | -0.15 | 0.15 |
| | 206.80 | [27] | | | | |
| $SiCl_4$ Cl $2p_{3/2}$ | 206.90 | [4] | 206.92 | 206.66 | -0.26 | 0.26 |
| | 206.94 | [1] | | | | |
| | 207.31 | [10] | | | | |
| $POCl_3$ Cl $2p_{3/2}$ | 207.33 | [8] | 207.17 | 207.12 | -0.05 | 0.05 |
| | 206.87* | [15] | | | | |
| HCl Cl $2p_{3/2}$ | 207.39 | [1] | 207.39 | 207.26 | -0.13 | 0.13 |
| | 207.38 | [26] | | | | |
| $Cl_2$ Cl $2p_{3/2}$ | 207.81 | [1] | 207.82 | 207.65 | -0.17 | 0.17 |
| | 207.82 | [26] | | | | |
| $Si(CH_3)_4$ C 1s | 289.78 | [1] | 289.78 | 289.65 | -0.13 | 0.13 |
| | 289.78 | [2,4] | | | | |

| Core level | Expt. $E_B$ | Reference | Average Expt $E_B$ | Calculated $E_B$ | Error (Theory - Expt) | Abs. Error \|Theory - Expt\| |
|---|---|---|---|---|---|---|
| $C_4H_5N$ (pyrrole) C 1s (C2) | 289.80<br>289.96 | [18]<br>[19] | 289.88 | 289.75 | -0.13 | 0.13 |
| $C_6H_6$ C 1s | Weighted average, | [28] | 290.39 | 290.14 | -0.25 | 0.25 |
| $C_2H_6$ C 1s | Weighted average, | [28] | 290.72 | 290.61 | -0.11 | 0.11 |
| $C_2H_4$ C 1s | 290.70<br>290.88 | [29]<br>[30] | 290.79 | 290.69 | -0.10 | 0.10 |
| $C_4H_5N$ (pyrrole) C 1s (C1) | 290.80<br>290.77 | [18]<br>[19] | 290.79 | 290.63 | -0.16 | 0.16 |
| $CH_4$ C 1s | Weighted average, | [28] | 290.84 | 290.76 | -0.08 | 0.08 |
| $CH_3COCH_3$ C 1s (methyl) | 291.15<br>291.23 | [31]<br>[5] | 291.19 | 291.08 | -0.11 | 0.11 |
| $CH_3COOH$ C 1s (methyl) | 291.55<br>291.60 | [31]<br>[16] | 291.58 | 291.52 | -0.06 | 0.06 |
| $CH_3OCH_3$ C 1s | 292.17<br>292.30<br>292.55 | [6]<br>[1]<br>[17] | 292.34 | 292.19 | -0.15 | 0.15 |
| $CH_3Cl$ C 1s | 292.40<br>292.48 | [32]<br>[1] | 292.44 | 292.48 | 0.04 | 0.04 |
| $CH_3OH$ C 1s | 292.30<br>292.42<br>292.80 | [16]<br>[6]<br>[33] | 292.51 | 292.42 | -0.09 | 0.09 |
| $CH_3F$ C 1s | 293.60<br>293.70 | [32]<br>[34,35] | 293.65 | 293.45 | -0.20 | 0.20 |
| $CH_3COCH_3$ C 1s (carbonyl) | 293.71<br>293.88 | [31]<br>[36] | 293.80 | 293.56 | -0.24 | 0.24 |
| $CHCl_3$ C 1s | 295.10<br>295.10 | [32]<br>[27] | 295.10 | 295.30 | 0.20 | 0.20 |
| $CH_3COOH$ C 1s (carboxyl) | 295.38<br>295.60 | [31]<br>[16] | 295.49 | 295.21 | -0.28 | 0.28 |
| HCOOH C 1s | 295.80<br>295.90 | [31]<br>[33,35] | 295.85 | 295.67 | -0.18 | 0.18 |
| CO C 1s | Weighted average, | [28] | 296.21 | 296.28 | 0.07 | 0.07 |
| $CCl_4$ C 1s | Weighted average, | [28] | 296.36 | 296.57 | 0.21 | 0.21 |
| $CH_2F_2$ C 1s | 296.36<br>296.44 | [35]<br>[37,35] | 296.40 | 296.15 | -0.25 | 0.25 |
| $CO_2$ C 1s | Weighted average, | [28] | 297.69 | 297.57 | -0.12 | 0.12 |
| $CF_4$ C1s | Weighted average, | [28] | 301.89 | 301.44 | -0.45 | 0.45 |
| $NH(C_2H_5)_2$ N 1s | 404.57<br>404.58 | [9,35]<br>[38] | 404.58 | 404.51 | -0.07 | 0.07 |

| Core level | Expt. $E_B$ | Reference | Average Expt $E_B$ | Calculated $E_B$ | Error (Theory - Expt) | Abs. Error \|Theory - Expt\| |
|---|---|---|---|---|---|---|
| $N(CH_3)_3$ N 1s | 404.80 | [8] | 404.81 | 404.81 | 0.00 | 0.00 |
| | 404.82 | [9,35] | | | | |
| $C_5H_5N$ (pyridine) N 1s | 404.82 | [38] | 404.88 | 404.66 | -0.22 | 0.22 |
| | 404.94 | [39,40] | | | | |
| $NH(CH_3)_2$ N 1s | 404.90 | [35] | 404.92 | 404.95 | 0.03 | 0.03 |
| | 404.93 | [9,35] | | | | |
| $NH_2CH_2CH_3$ N 1s | 404.93 | [38] | 404.96 | 404.99 | 0.03 | 0.03 |
| | 404.98 | [9,35] | | | | |
| $CH_3NH_2$ N 1s | 405.10 | [41,35] | 405.14 | 405.23 | 0.09 | 0.09 |
| | 405.15 | [17] | | | | |
| | 405.17 | [9,35] | | | | |
| $C_6H_5NH_2$ N 1s | Weighted average, [28] | | 405.40 | 405.29 | -0.11 | 0.11 |
| $NH_3$ N 1s | 405.52 | [9,35] | 405.57 | 405.7 | 0.13 | 0.13 |
| | 405.60 | [35] | | | | |
| | 405.60 | [8] | | | | |
| $CH_3CN$ N 1s | Weighted average, [28] | | 405.64 | 405.41 | -0.23 | 0.23 |
| $C_4H_5N$ (pyrrole) N 1s | 406.10 | [18] | 406.14 | 406.16 | 0.02 | 0.02 |
| | 406.18 | [38] | | | | |
| | 406.15 | [19] | | | | |
| $N_2O$ N 1s (terminal N) | Weighted average, [28] | | 408.71 | 408.73 | 0.02 | 0.02 |
| $N_2$ N 1s | Weighted average, [28] | | 409.98 | 409.96 | -0.02 | 0.02 |
| $N_2O$ N 1s (centre N) | Weighted average, [28] | | 412.59 | 412.62 | 0.03 | 0.03 |
| $CH_3COCH_3$ O 1s | 537.92 | [42] | 537.99 | 537.73 | -0.26 | 0.26 |
| | 538.05 | [36] | | | | |
| $POCl_3$ O 1s | 537.97 | [43] | 538.04 | 538.03 | -0.01 | 0.01 |
| | 538.10 | [15] | | | | |
| $CH_3COOH$ O 1s (C=O) | 538.29 | [31] | 538.33 | 538.14 | -0.19 | 0.19 |
| | 538.36 | [9] | | | | |
| $CH_3CHO$ O 1s | 538.50 | [36] | 538.59 | 538.39 | -0.20 | 0.20 |
| | 538.62 | [42] | | | | |
| | 538.64 | [9,16] | | | | |
| $CH_3OCH_3$ O 1s | 538.59 | [17] | 538.74 | 538.81 | 0.07 | 0.07 |
| | 538.61 | [9,16] | | | | |
| | 539.03 | [1] | | | | |
| HCOOH O 1s (C=O) | Weighted average, [28] | | 538.97 | 538.83 | -0.14 | 0.14 |
| $CH_3OH$ O 1s | Weighted average, [28] | | 539.11 | 539.11 | 0.00 | 0.00 |
| HCHO O 1s | 539.42 | [42] | 539.48 | 539.38 | -0.10 | 0.10 |
| | 539.44 | [44] | | | | |
| | 539.58 | [9,16] | | | | |

| Core level | Expt. $E_B$ | | Reference | Average Expt $E_B$ | Calculated $E_B$ | Error (Theory - Expt) |
|---|---|---|---|---|---|---|
| $H_2O$ O 1s | Weighted average, [28] | | 539.90 | 539.88 | -0.02 | 0.02 |
| $CH_3COOH$ OH O 1s | 540.09 | [31] | 540.12 | 540.17 | 0.05 | 0.05 |
| | 540.15 | [9,16] | | | | |
| HCOOH O 1s (-OH) | Weighted average, [28] | | 540.63 | 540.78 | 0.15 | 0.15 |
| $CO_2$ O 1s | Weighted average, [28] | | 541.28 | 541.36 | 0.08 | 0.08 |
| $N_2O$ O 1s | 541.40 | [16] | 541.41 | 541.64 | 0.23 | 0.23 |
| | 541.42 | [33,35] | | | | |
| CO O 1s | Weighted average, [28] | | 542.55 | 542.59 | 0.04 | 0.04 |
| $O_2$ O 1s (strong line) | 543.10 | [16] | 543.28 | 543.52 | 0.24 | 0.24 |
| | 543.35 | [33] | | | | |
| | 543.39 | [7] | | | | |
| $O_2$ O 1s (weak line) | 544.20 | [16] | 544.38 | 544.38 | 0.00 | 0.00 |
| | 544.47 | [7] | | | | |
| | 544.47 | [33] | | | | |
| $C_6H_5F$ F 1s | Weighted average, [28] | | 692.92 | 693.02 | 0.10 | 0.10 |
| $PF_3$ F 1s | 694.09 | [10] | 694.14 | 694.17 | 0.03 | 0.03 |
| | 694.20 | [15] | | | | |
| $PF_5$ F 1s (axial) | 694.10 | [45] | 694.15 | 694.14 | -0.01 | 0.01 |
| | 694.20 | [15] | | | | |
| HF F 1s | Weighted average, [28] | | 694.23 | 694.28 | 0.05 | 0.05 |
| $CF_3CCCF_3$ F 1s | 694.36 | [46] | 694.45 | 694.71 | 0.26 | 0.26 |
| | 694.54 | [47] | | | | |
| $PF_5$ F 1s (equatorial) | 695.30 | [45] | 695.35 | 695.31 | -0.04 | 0.04 |
| | 695.40 | [15] | | | | |
| $CF_4$ F 1s | Weighted average, [28] | | 695.56 | 695.41 | -0.15 | 0.15 |
| $F_2$ F 1s | 696.66 | [48] | 696.69 | 696.65 | -0.04 | 0.04 |
| | 696.71 | [49] | | | | |
| Mean error: -0.09 eV | | | | | | |
| Mean unsigned error: 0.16 eV | | | | | | |


1. W.B. Perry et al., Inorg. Chem. 13, 1211 (1974)
2. J.E. Drake et al., Inorg. Chem. 17, 2333 (1978)
3. P. Kelfve et al., Phys. Scripta 21, 75 (1980)
4. J.E. Drake et al., Can. J. Chem. 53, 3602 (1975)
5. W.L. Jolly et al., marked as unpublished data in At. Data Nucl. Data Tables 31, 433 (1984)
6. J.E. Drake et al., Can. J. Chem. 55, 2957 (1977)
7. W.L. Jolly et al., marked as unpublished data in At. Data Nucl. Data Tables 31, 433 (1984)
8. W.B. Perry et al., J. Am. Chem. Soc. 97, 4899 (1975)
9. B.E. Mills, J. Am. Chem. Soc. 98, 2380 (1976)
10. S.C. Avanzino et al., Inorg. Chem. 16, 2046 (1977)
11. R.N. Sodhi et al., J. Electron Spectrosc. Relat. Phenom. 32, 283 (1983)
12. A.J. Ashe III et al., J. Am. Chem. Soc. 101, 1764 (1979)

13. R.G. Cavell et al., J. Electron Spectrosc. Relat. Phenom. 15, 145 (1979)
14. T.H. Lee, et al., J. Am. Chem. Soc. 102, 2631 (1980)
15. R.G. Cavell, Inorg. Chem. 14, 2828 (1975)
16. K. Siegbahn et al., "ESCA Applied to Free Molecules", North-Holland Publishing Co., Amsterdam, (1969)
17. J.S. Jen et al., J. Electron Spectrosc. Relat. Phenom. 4, 43 (1974)
18. U. Gelius et al., Phys. Scripta 3, 237 (1971)
19. S.A. Chambers et al., J. Chem. Phys. 67, 2596 (1977)
20. C.J. Allan et al., J. Electron Spectrosc. Relat. Phenom. 1, 131 (1972)
21. L. Pettersson et al., J. Electron Spectrosc. Relat. Phenom. 27, 29 (1982)
22. P. Finn et al., J. Am. Chem. Soc. 94, 1540 (1972)
23. D.A. Allison et al., J. Electron Spectrosc. Relat. Phenom. 1, 269 (1972)
24. D.B. Beach et al., J. Am. Chem. Soc. 106, 536 (1984)
25. D.B. Beach, "A Photoelectron Spectroscopic Study of Bonding in Inorganic and Organometallic Compounds", Ph. D Thesis, University of California, Berkeley (1985)
26. E.J. Aitken et al., J. Am. Chem. Soc. 102, 4873 (1980)
27. T. Ohta et al., Bull. Chem. Soc. Jpn. 49, 2939 (1976)
28. G. Cavigliasso et al., J. Chem. Phys. 111, 9485 (1999), and G. Cavigliasso, M.Sc. Thesis, University of British Columbia, Vancouver (1999)
29. T.D. Thomas, J. Chem. Phys. 52, 1373 (1970)
30. A. Berndtsson et al., Phys. Scripta 12, 235 (1975)
31. S.R. Smith et al., J. Am. Chem. Soc. 100, 5459 (1978)
32. T.D. Thomas et al., J. Am. Chem. Soc. 92, 4184 (1970)
33. D.W. Davis et al., J. Chem. Phys. 52, 3295 (1970)
34. D.W. Davis et al., "Electron Spectroscopy", North-Holland Publishing Co., Amsterdam, (1972)
35. T.D. Thomas et al., J. Electron Spectrosc. Relat. Phenom. 5, 1081 (1974)
36. W.L. Jolly et al., J. Am. Chem. Soc. 98, 3178 (1976)
37. D.W. Davis, Ph.D Thesis, University of California, Berkeley, (1973)
38. R.G. Cavell et al., J. Am. Chem. Soc. 99, 4203 (1977)
39. R.S. Brown et al., J. Am. Chem. Soc. 102, 1174 (1980)
40. R.S. Brown et al., Can. J. Chem. 59, 694 (1980)
41. P. Finn et al., Inorg. Chem. 10, 378 (1971)
42. T.X. Carroll et al., J. Am. Chem. Soc. 97, 659 (1975)
43. S.C. Avanzino et al., Inorg. Chem. 14, 1595 (1975)
44. T.X. Carroll et al., J. Electron Spectrosc. Relat. Phenom. 10, 215 (1977)
45. R.W. Shaw Jr. et al., J. Am. Chem. Soc. 95, 5870 (1973)
46. P. Brant et al., J. Electron Spectrosc. Relat. Phenom. 22, 119 (1981)
47. R.G. Cavell et al., J. Electron Spectrosc. Relat. Phenom. 6, 281 (1975)
48. S.C. Avanzino, Ph.D. Thesis, University of California, Berkeley, (1978)
49. T.X. Carroll et al., J. Am. Chem. Soc. 96, 1989 (1974)

# Comparison with the molecular dataset from PRL 118, 026401 (2017)

The same experimental values are used as in the supplementary information of Ozaki et al., PRL 118, 026401 (2017). Note that some of them are different from the average experimental values used in the table above.

All values are given in eV.

| Core level | Expt. $E_B$ | Calculated $E_B$ (Ozaki et al.) | Calculated $E_B$ (This work) | Abs. Error (Ozaki et al.) | Abs. Error (This work) |
|---|---|---|---|---|---|
| CO C 1s | 296.19 | 295.87 | 296.28 | 0.32 | 0.09 |
| $C_2H_2$ C 1s | 291.17 | 291.24 | 291.20 | 0.07 | 0.03 |
| $CO_2$ C 1s | 297.66 | 296.89 | 297.57 | 0.77 | 0.09 |
| HCN C 1s | 293.50 | 293.35 | 293.46 | 0.15 | 0.04 |
| $C_2H_4$ C 1s | 290.79 | 290.50 | 290.69 | 0.29 | 0.10 |
| $H_2CO$ C 1s | 294.47 | 294.00 | 294.48 | 0.47 | 0.01 |
| $N_2$ N 1s | 409.83 | 409.89 | 409.96 | 0.06 | 0.13 |
| $NH_3$ N 1s | 405.60 | 404.70 | 405.70 | 0.90 | 0.10 |
| $N_2H_4$ N 1s | 406.10 | 404.82 | 405.95 | 1.28 | 0.15 |
| HCN N 1s | 406.36 | 406.16 | 406.73 | 0.20 | 0.37 |
| $N_2O$ (end N) N 1s | 408.66 | 408.24 | 408.73 | 0.42 | 0.07 |
| $N_2O$ (mid N) N 1s | 412.57 | 411.98 | 412.62 | 0.59 | 0.05 |
| NO (S=0) N 1s | 411.6 | 410.62 | 411.23 | 0.98 | 0.37 |
| NO (S=1) N 1s | 410.2 | 410.1 | 410.51 | 0.10 | 0.31 |
| CO O 1s | 542.4 | 542.5 | 542.59 | 0.10 | 0.19 |
| $CO_2$ O 1s | 541.20 | 541.08 | 541.36 | 0.12 | 0.16 |
| $O_2$ (S=1/2) O 1s | 544.2 | 543.15 | 544.38 | 1.05 | 0.18 |
| $O_2$ (S=3/2) O 1s | 543.1 | 542.64 | 543.52 | 0.46 | 0.42 |
| $H_2O$ O 1s | 539.9 | 539.18 | 539.88 | 0.72 | 0.02 |
| $SiH_4$ Si 2p | 107.3 | 106.56 | 107.25 | 0.74 | 0.05 |
| $Si_2H_6$ Si 2p | 106.86 | 106.21 | 107.27 | 0.65 | 0.41 |
| $SiF_4$ Si 2p | 111.7 | 111.02 | 111.00 | 0.68 | 0.70 |
| $SiCl_4$ Si 2p | 110.2 | 109.32 | 110.44 | 0.88 | 0.24 |
| Mean Absolute Error | | | | 0.52 | 0.19 |
| Maximum Absolute Error | | | | 1.28 | 0.70 |

# Basis sets used in the molecular calculations

## Numerical basis sets with additional core functions

Constructed by adding additional core functions to the FHI-aims “tight” default basis sets (Blum et al., Comput. Phys. Commun. 180, 2175 (2009)). Given in FHI-aims format, together with a definition of other numerical parameters. These basis sets were only used for the atom whose core electron is removed. The same basis set is always used for the ground state and the final state.

### Boron

```
# core-hole
  species        B
#     global species definitions
    nucleus             5
    mass                10.811
#
    l_hartree           6
#
    cut_pot             4.0  2.0  1.0
    basis_dep_cutoff    1e-4
#
    radial_base         32 7.0
    radial_multiplier   2
    angular_grids       specified
      division   0.3742  110
      division   0.5197  194
      division   0.5753  302
      division   0.7664  434
#      division   0.8392  770
#      division   1.6522  974
#      outer_grid   974
      outer_grid  434

#     valence basis states
    valence      2  s   2.
    valence      2  p   1.
#     ion occupancy
    ion_occ      2  s   1.

#  "First tier" - improvements: -710.52 meV to -92.39 meV
     hydro 2 p 1.4
     hydro 3 d 4.8
     hydro 2 s 4
#  "Second tier" - improvements: -33.88 meV to -2.20 meV
     hydro 4 f 7.8
     hydro 3 p 4.2
     hydro 3 s 3.3
     hydro 5 g 11.2
     hydro 3 d 5.4
#  "Third tier" - improvements: -1.28 meV to -0.36 meV
     hydro 2 p 4.7
     hydro 2 s 8.4
     hydro 4 d 5.8
#  "Fourth tier" - improvements: -0.25 meV to -0.12 meV
#     hydro 3 p 2.2
#     hydro 3 s 3
#     hydro 4 f 9.8
```

```
#     hydro 5 g 12.8
#     hydro 4 d 10
#  Further functions
#     hydro 4 f 14
#     hydro 3 p 12.4

## Additional basis functions for core hole
hydro 1 s 9.0
hydro 1 s 7.0
hydro 1 s 3.0
hydro 2 s 5.0
hydro 2 p 6.0
```

## Carbon

```
# core-hole
  species        C
#     global species definitions
    nucleus             6
    mass                12.0107
#
    l_hartree           6
#
    cut_pot             4.0  2.0  1.0
    basis_dep_cutoff    1e-4
#
    radial_base         34 7.0
    radial_multiplier   2
    angular_grids specified
      division   0.2187   50
      division   0.4416  110
      division   0.6335  194
      division   0.7727  302
      division   0.8772  434
#      division   0.9334  590
#      division   0.9924  770
#      division   1.0230  974
#      division   1.5020 1202
#     outer_grid  974
      outer_grid  434

#     valence basis states
    valence      2  s   2.
    valence      2  p   2.
#     ion occupancy
    ion_occ      2  s   1.
    ion_occ      2  p   1.

#  "First tier" - improvements: -1214.57 meV to -155.61 meV
     hydro 2 p 1.7
     hydro 3 d 6
     hydro 2 s 4.9
#  "Second tier" - improvements: -67.75 meV to -5.23 meV
     hydro 4 f 9.8
     hydro 3 p 5.2
     hydro 3 s 4.3
     hydro 5 g 14.4
     hydro 3 d 6.2
#  "Third tier" - improvements: -2.43 meV to -0.60 meV
     hydro 2 p 5.6
     hydro 2 s 1.4
```

```
     hydro 3 d 4.9
     hydro 4 f 11.2
#  "Fourth tier" - improvements: -0.39 meV to -0.18 meV
#     hydro 2 p 2.1
#     hydro 5 g 16.4
#     hydro 4 d 13.2
#     hydro 3 s 13.6
#     hydro 4 f 17.6
#  Further basis functions - improvements: -0.08 meV and below
#     hydro 3 s 2
#     hydro 3 p 6
#     hydro 4 d 20

# Additional basis functions for an atom with a core hole
     hydro 1 s 10.0
     hydro 1 s 8.0
     hydro 1 s 4.0
     hydro 2 s 6.0
```

## Nitrogen

```
# core-hole
  species        N
#     global species definitions
    nucleus             7
    mass                14.0067
#
    l_hartree           6
#
    cut_pot             4.0  2.0  1.0
    basis_dep_cutoff    1e-4
#
    radial_base         35 7.0
    radial_multiplier   2
    angular_grids       specified
      division   0.1841   50
      division   0.3514  110
      division   0.5126  194
      division   0.6292  302
      division   0.6939  434
#      division   0.7396  590
#      division   0.7632  770
#      division   0.8122  974
#      division   1.1604 1202
#      outer_grid  974
      outer_grid  434

#     valence basis states
    valence      2  s   2.
    valence      2  p   3.
#     ion occupancy
    ion_occ      2  s   1.
    ion_occ      2  p   2.

#  "First tier" - improvements: -1193.42 meV to -220.60 meV
     hydro 2 p 1.8
     hydro 3 d 6.8
#     hydro 3 s 5.8
#  "Second tier" - improvements: -80.21 meV to -6.86 meV
     hydro 4 f 10.8
#     hydro 3 p 5.8
```

```
     hydro 1 s 0.8
     hydro 5 g 16
     hydro 3 d 4.9
#  "Third tier" - improvements: -4.29 meV to -0.53 meV
     hydro 3 s 16
     ionic 2 p auto
     hydro 3 d 6.6
     hydro 4 f 11.6
#  "Fourth tier" - improvements: -0.75 meV to -0.25 meV
#     hydro 2 p 4.5
#     hydro 2 s 2.4
#     hydro 5 g 14.4
#     hydro 4 d 14.4
#     hydro 4 f 16.8
# Further basis functions - -0.21 meV and below
#     hydro 3 p 14.8
#     hydro 3 s 4.4
#     hydro 3 d 19.6
#     hydro 5 g 12.8

# additional basis functions for atom with a core hole
     hydro 1 s 11.0
     hydro 1 s 9.0
     hydro 1 s 5.0
     hydro 2 s 8.0
     hydro 2 s 10.0
     hydro 2 p 6.5
     hydro 3 s 6.2
     hydro 3 p 6.2
```

## Oxygen

```
# core-hole
  species        O
#     global species definitions
    nucleus             8
    mass                15.9994
#
    l_hartree           6
#
    cut_pot             4.0  2.0  1.0
    basis_dep_cutoff    1e-4
#
    radial_base         36 7.0
    radial_multiplier   2
     angular_grids specified
      division   0.1817   50
      division   0.3417  110
      division   0.4949  194
      division   0.6251  302
      division   0.8014  434
#      division   0.8507  590
#      division   0.8762  770
#      division   0.9023  974
#      division   1.2339 1202
#      outer_grid 974
      outer_grid  434

#     valence basis states
    valence      2  s   2.
    valence      2  p   4.
```

```
#     ion occupancy
    ion_occ      2  s   1.
    ion_occ      2  p   3.

#  "First tier" - improvements: -699.05 meV to -159.38 meV
     hydro 2 p 1.8
     hydro 3 d 7.6
     hydro 3 s 6.4
#  "Second tier" - improvements: -49.91 meV to -5.39 meV
     hydro 4 f 11.6
     hydro 3 p 6.2
     hydro 3 d 5.6
     hydro 5 g 17.6
     hydro 1 s 0.75
#  "Third tier" - improvements: -2.83 meV to -0.50 meV
     ionic 2 p auto
     hydro 4 f 10.8
     hydro 4 d 4.7
     hydro 2 s 6.8
#  "Fourth tier" - improvements: -0.40 meV to -0.12 meV
#     hydro 3 p 5
#     hydro 3 s 3.3
#     hydro 5 g 15.6
#     hydro 4 f 17.6
#     hydro 4 d 14
# Further basis functions - -0.08 meV and below
#     hydro 3 s 2.1
#     hydro 4 d 11.6
#     hydro 3 p 16
#     hydro 2 s 17.2

# additional basis functions for atom with a core hole
     hydro 1 s 12.0
     hydro 1 s 10.0
     hydro 1 s 6.0
     hydro 2 s 10.0
     hydro 2 p 8.0
     hydro 2 p 6.0
     hydro 3 d 8.0
```

## Fluorine

```
# core-hole
  species        F
#     global species definitions
    nucleus             9
    mass                18.9984032
#
    l_hartree           6
#
    cut_pot             4.0  2.0  1.0
    basis_dep_cutoff    1e-4
#
    radial_base         37 7.0
    radial_multiplier   2
    angular_grids specified
      division   0.4014  110
      division   0.5291  194
      division   0.6019  302
      division   0.6814  434
#      division   0.7989  590
```

```
#      division   0.8965  770
#      division   1.3427  974
#      outer_grid   974
     outer_grid  434

#     valence basis states
    valence      2  s   2.
    valence      2  p   5.
#     ion occupancy
    ion_occ      2  s   1.
    ion_occ      2  p   4.

#  "First tier" - improvements: -149.44 meV to -45.88 meV
     hydro 2 p 1.7
     hydro 3 d 7.4
     hydro 3 s 6.8
#  "Second tier" - improvements: -12.96 meV to -1.56 meV
     hydro 4 f 11.2
     ionic 2 p auto
     hydro 1 s 0.75
     hydro 4 d 8.8
     hydro 5 g 16.8
#  "Third tier" - improvements: -0.58 meV to -0.05 meV
     hydro 3 p 6.2
#     hydro 3 s 3.2
     hydro 4 f 9.6
     hydro 3 s 19.6
     hydro 4 d 8.6
     hydro 5 g 14.4
# Further basis functions: -0.05 meV and below
#     hydro 3 p 4.2

# additional basis functions for atom with a core hole
     hydro 1 s 13.0
     hydro 1 s 11.0
     hydro 1 s 7.0
     hydro 2 s 11.5
     hydro 2 s 9.5
     hydro 2 p 8.5
     hydro 2 p 6.5
     hydro 3 d 5.6
     hydro 3 p 4.2
```

## Silicon

```
# core-hole
  species        Si
#     global species definitions
    nucleus             14
    mass                28.0855
#
    l_hartree           6
#
    cut_pot             4.0          2.0  1.0
    basis_dep_cutoff    1e-4
#
    radial_base         42 7.0
    radial_multiplier   2
    angular_grids       specified
      division   0.4121   50
      division   0.7665  110
```

```
      division   1.0603  194
      division   1.2846  302
      division   1.4125  434
#      division   1.4810  590
#      division   1.5529  770
#      division   1.6284  974
#      division   2.6016 1202
#      outer_grid   974
      outer_grid  434

#     valence basis states
    valence      3  s   2.
    valence      3  p   2.
#     ion occupancy
    ion_occ      3  s   1.
    ion_occ      3  p   1.

#  "First tier" - improvements: -571.96 meV to -37.03 meV
     hydro 3 d 4.2
     hydro 2 p 1.4
     hydro 4 f 6.2
     ionic 3 s auto
#  "Second tier" - improvements: -16.76 meV to -3.03 meV
     hydro 3 d 9
     hydro 5 g 9.4
     hydro 4 p 4
     hydro 1 s 0.65
#  "Third tier" - improvements: -3.89 meV to -0.60 meV
     ionic 3 d auto
     hydro 3 s 2.6
     hydro 4 f 8.4
     hydro 3 d 3.4
     hydro 3 p 7.8
#  "Fourth tier" - improvements: -0.33 meV to -0.11 meV
#     hydro 2 p 1.6
#     hydro 5 g 10.8
#     hydro 5 f 11.2
#     hydro 3 d 1
#     hydro 4 s 4.5
#  Further basis functions that fell out of the optimization - noise
#  level... < -0.08 meV
#     hydro 4 d 6.6
#     hydro 5 g 16.4
#     hydro 4 d 9

# Additional basis functions for atoms with a core hole

     hydro 2 p 15.0
     hydro 2 p 12.0
     hydro 2 p 5.0
     hydro 2 s 14.0
     hydro 1 s 16.0
     hydro 1 s 9.0
```

## Phosphorus

```
# core-hole
  species        P
#     global species definitions
    nucleus             15
    mass                30.973762
```

```
#
    l_hartree           6
#
    cut_pot             4.0          2.0  1.0
    basis_dep_cutoff    1e-4
#
    radial_base         43 7.0
    radial_multiplier   2
    angular_grids       specified
      division   0.2995   50
      division   0.5998  110
      division   0.9240  194
      division   1.0921  302
      division   1.2863  434
#      division   1.3165  590
#      division   1.4113  770
#      division   1.5128  974
#      division   2.4980 1202
      outer_grid  434

#     valence basis states
    valence      3  s   2.
    valence      3  p   3.
#     ion occupancy
    ion_occ      3  s   1.
    ion_occ      3  p   2.

#  "First tier" - improvements: -726.20 meV to -35.91 meV
     ionic 3 d auto
     ionic 3 p auto
     hydro 4 f 6.2
     hydro 5 g 8.6
     ionic 3 s auto
#  "Second tier" - improvements: -16.02 meV to -1.71 meV
     hydro 4 d 6.2
     hydro 4 p 9.2
     hydro 5 f 9.8
     hydro 1 s 0.7
     hydro 5 g 13.2
#  "Third tier" - improvements: -1.82 meV to -0.20 meV
     hydro 3 p 2.5
     hydro 4 d 6.4
     hydro 5 f 11.2
     hydro 2 s 1.5
#  "Fourth tier" - improvements: -0.91 meV to -0.17 meV
#     hydro 3 d 16.8
#     hydro 5 g 18
#     hydro 4 p 4.5
#     hydro 3 s 2.1
#  Further basis functions that fell out of the optimization - < -0.09 meV
#     hydro 4 p 10.4
#     hydro 4 d 17.6
#     hydro 4 s 11.2

# Additional basis functions for atoms with a core hole

     hydro 2 p 16.0
     hydro 2 p 13.0
     hydro 2 p 6.0
     hydro 2 s 15.0
     hydro 1 s 17.0
```

```
     hydro 1 s 10.0
```

## Sulfur

```
# core-hole
  species        S
#     global species definitions
    nucleus             16
    mass                32.065
#
    l_hartree           6
#
    cut_pot             4.0          2.0  1.0
    basis_dep_cutoff    1e-4
#
    radial_base         44 7.0
    radial_multiplier   2
    angular_grids       specified
      division   0.4665  110
      division   0.5810  194
      division   0.7139  302
      division   0.8274  434
#      division   0.9105  590
#      division   1.0975  770
#      division   1.2028  974
#      outer_grid  974
      outer_grid  434

#     valence basis states
    valence      3  s   2.
    valence      3  p   4.
#     ion occupancy
    ion_occ      3  s   1.
    ion_occ      3  p   3.

#  "First tier" - improvements: -652.81 meV to -45.53 meV
     ionic 3 d auto
     hydro 2 p 1.8
     hydro 4 f 7
     ionic 3 s auto
#  "Second tier" - improvements: -30.20 meV to -1.74 meV
     hydro 4 d 6.2
     hydro 5 g 10.8
     hydro 4 p 4.9
     hydro 5 f 10
     hydro 1 s 0.8
#  "Third tier" - improvements: -1.04 meV to -0.20 meV
     hydro 3 d 3.9
     hydro 3 d 2.7
     hydro 5 g 12
     hydro 4 p 10.4
     hydro 5 f 12.4
     hydro 2 s 1.9
#  "Fourth tier" - improvements: -0.35 meV to -0.06 meV
#     hydro 4 d 10.4
#     hydro 4 p 7.2
#     hydro 4 d 10
#     hydro 5 g 19.2
#     hydro 4 s 12

# Additional basis functions for atoms with a core hole
```

```
     hydro 2 p 17.0
     hydro 2 p 14.0
     hydro 2 p 7.0
     hydro 2 s 16.0
     hydro 1 s 18.0
     hydro 1 s 11.0
```

## Chlorine

```
# core-hole
  species        Cl
#     global species definitions
    nucleus             17
    mass                35.453
#
    l_hartree           6
#
    cut_pot             4.0          2.0  1.0
    basis_dep_cutoff    1e-4
#
    radial_base         45 7.0
    radial_multiplier   2
    angular_grids       specified
      division   0.4412  110
      division   0.5489  194
      division   0.6734  302
      division   0.7794  434
#      division   0.9402  590
#      division   1.0779  770
#      division   1.1792  974
#      outer_grid  974
      outer_grid  434

#     valence basis states
    valence      3  s   2.
    valence      3  p   5.
#     ion occupancy
    ion_occ      3  s   1.
    ion_occ      3  p   4.

#  "First tier" - improvements: -429.57 meV to -15.03 meV
     ionic 3 d auto
     hydro 2 p 1.9
     hydro 4 f 7.4
     ionic 3 s auto
     hydro 5 g 10.4
#  "Second tier" - improvements: -7.84 meV to -0.48 meV
     hydro 3 d 3.3
     hydro 5 f 9.8
     hydro 1 s 0.75
     hydro 5 g 11.2
     hydro 4 p 10.4
#  "Third tier" - improvements: -1.00 meV to -0.12 meV
     hydro 4 d 12.8
     hydro 4 f 4.6
     hydro 4 d 10.8
     hydro 2 s 1.8
     hydro 3 p 3
#  Further functions that fell out - improvements: -0.10 meV and below
#     hydro 5 f 14.4
```

```
#     hydro 4 s 12.8
#     hydro 3 d 11.6
#     hydro 4 s 4.1

# Additional basis functions for atoms with a core hole

     hydro 3 d  8.0
     hydro 3 p  8.0
     hydro 3 s 14.0
     hydro 2 p 15.0
     hydro 2 p 11.5
     hydro 2 p  9.0
     hydro 2 s 18.0
     hydro 2 s 16.0
     hydro 1 s 19.0
     hydro 1 s 12.0
```

## Standard numerical basis sets

These are the FHI-aims "tight" default basis sets with all Tier 1 and 2 basis functions enabled (Blum et al., Comput. Phys. Commun. 180, 2175 (2009)) that are only reproduced here for completeness. Given in FHI-aims format, together with a definition of other numerical parameters. These basis sets were used in the molecular calculations for all other atoms, except for the one whose core electron is removed.

## Hydrogen

```
################################################################################
#
#  FHI-aims code project
# Volker Blum, Fritz Haber Institute Berlin, 2009
#
#  Suggested "tight" defaults for H atom (to be pasted into control.in file)
#
################################################################################
  species        H
#     global species definitions
    nucleus             1
    mass                1.00794
#
    l_hartree           6
#
    cut_pot             4.0  2.0  1.0
    basis_dep_cutoff    1e-4
#
    radial_base         24 7.0
    radial_multiplier   2
    angular_grids       specified
      division   0.1930   50
      division   0.3175  110
      division   0.4293  194
      division   0.5066  302
      division   0.5626  434
#      division   0.5922  590
#      division   0.6227  974
#      division   0.6868 1202
#      outer_grid  770
      outer_grid  434
################################################################################
#
#  Definition of "minimal" basis
#
```

```
################################################################################
#     valence basis states
    valence      1  s   1.
#     ion occupancy
    ion_occ      1  s   0.5
################################################################################
#
#  Suggested additional basis functions. For production calculations,
#  uncomment them one after another (the most important basis functions are
#  listed first).
#
#  Basis constructed for dimers: 0.5 A, 0.7 A, 1.0 A, 1.5 A, 2.5 A
#
################################################################################
#  "First tier" - improvements: -1014.90 meV to -62.69 meV
     hydro 2 s 2.1
     hydro 2 p 3.5
#  "Second tier" - improvements: -12.89 meV to -1.83 meV
     hydro 1 s 0.85
     hydro 2 p 3.7
     hydro 2 s 1.2
     hydro 3 d 7
#  "Third tier" - improvements: -0.25 meV to -0.12 meV
#     hydro 4 f 11.2
#     hydro 3 p 4.8
#     hydro 4 d 9
#     hydro 3 s 3.2
################################################################################
#
# For methods that use the localized form of the "resolution of identity" for
# the two-electron Coulomb operator (RI_method LVL), particularly Hartree-Fock and
# hybrid density functional calculations, the highest accuracy can be obtained by
# uncommenting the line beginning with "for_aux"  below, thus adding an extra g radial
# function to the construction of the product basis set for the expansion.
# See Ref. New J. Phys. 17, 093020 (2015) for more information, particularly Figs. 1 and 6.
#
################################################################################
#
# for_aux hydro 5 g 6.0
```

## Boron

```
################################################################################
#
#  FHI-aims code project
# Volker Blum, Fritz Haber Institute Berlin, 2009
#
#  Suggested "tight" defaults for B atom (to be pasted into control.in file)
#
################################################################################
  species        B
#     global species definitions
    nucleus             5
    mass                10.811
#
    l_hartree           6
#
    cut_pot             4.0  2.0  1.0
    basis_dep_cutoff    1e-4
#
    radial_base         32 7.0
```

```
    radial_multiplier   2
    angular_grids       specified
      division   0.3742  110
      division   0.5197  194
      division   0.5753  302
      division   0.7664  434
#      division   0.8392  770
#      division   1.6522  974
#      outer_grid   974
      outer_grid  434
################################################################################
#
#  Definition of "minimal" basis
#
################################################################################
#     valence basis states
    valence      2  s   2.
    valence      2  p   1.
#     ion occupancy
    ion_occ      2  s   1.
################################################################################
#
#  Suggested additional basis functions. For production calculations,
#  uncomment them one after another (the most important basis functions are
#  listed first).
#
#  Constructed for dimers: 1.25 A, 1.625 A, 2.5 A, 3.5 A
#
################################################################################
#  "First tier" - improvements: -710.52 meV to -92.39 meV
     hydro 2 p 1.4
     hydro 3 d 4.8
     hydro 2 s 4
#  "Second tier" - improvements: -33.88 meV to -2.20 meV
     hydro 4 f 7.8
     hydro 3 p 4.2
     hydro 3 s 3.3
     hydro 5 g 11.2
     hydro 3 d 5.4
#  "Third tier" - improvements: -1.28 meV to -0.36 meV
#     hydro 2 p 4.7
#     hydro 2 s 8.4
#     hydro 4 d 5.8
#  "Fourth tier" - improvements: -0.25 meV to -0.12 meV
#     hydro 3 p 2.2
#     hydro 3 s 3
#     hydro 4 f 9.8
#     hydro 5 g 12.8
#     hydro 4 d 10
#  Further functions
#     hydro 4 f 14
#     hydro 3 p 12.4
################################################################################
#
# For methods that use the localized form of the "resolution of identity" for
# the two-electron Coulomb operator (RI_method LVL), particularly Hartree-Fock and
# hybrid density functional calculations, the highest accuracy can be obtained by
# uncommenting the line beginning with "for_aux"  below, thus adding an extra g radial
# function to the construction of the product basis set for the expansion.
# See Ref. New J. Phys. 17, 093020 (2015) for more information, particularly Figs. 1 and 6.
#
```

```
################################################################################
#
# for_aux hydro 5 g 6.0
```

## Carbon

```
################################################################################
#
#  FHI-aims code project
# Volker Blum, Fritz Haber Institute Berlin, 2009
#
#  Suggested "tight" defaults for C atom (to be pasted into control.in file)
#
################################################################################
  species        C
#     global species definitions
    nucleus             6
    mass                12.0107
#
    l_hartree           6
#
    cut_pot             4.0  2.0  1.0
    basis_dep_cutoff    1e-4
#
    radial_base         34 7.0
    radial_multiplier   2
    angular_grids specified
      division   0.2187   50
      division   0.4416  110
      division   0.6335  194
      division   0.7727  302
      division   0.8772  434
#      division   0.9334  590
#      division   0.9924  770
#      division   1.0230  974
#      division   1.5020 1202
#     outer_grid  974
      outer_grid  434
################################################################################
#
#  Definition of "minimal" basis
#
################################################################################
#     valence basis states
    valence      2  s   2.
    valence      2  p   2.
#     ion occupancy
    ion_occ      2  s   1.
    ion_occ      2  p   1.
################################################################################
#
#  Suggested additional basis functions. For production calculations,
#  uncomment them one after another (the most important basis functions are
#  listed first).
#
#  Constructed for dimers: 1.0 A, 1.25 A, 1.5 A, 2.0 A, 3.0 A
#
################################################################################
#  "First tier" - improvements: -1214.57 meV to -155.61 meV
     hydro 2 p 1.7
     hydro 3 d 6
```

```
     hydro 2 s 4.9
#  "Second tier" - improvements: -67.75 meV to -5.23 meV
     hydro 4 f 9.8
     hydro 3 p 5.2
     hydro 3 s 4.3
     hydro 5 g 14.4
     hydro 3 d 6.2
#  "Third tier" - improvements: -2.43 meV to -0.60 meV
#     hydro 2 p 5.6
#     hydro 2 s 1.4
#     hydro 3 d 4.9
#     hydro 4 f 11.2
#  "Fourth tier" - improvements: -0.39 meV to -0.18 meV
#     hydro 2 p 2.1
#     hydro 5 g 16.4
#     hydro 4 d 13.2
#     hydro 3 s 13.6
#     hydro 4 f 17.6
#  Further basis functions - improvements: -0.08 meV and below
#     hydro 3 s 2
#     hydro 3 p 6
#     hydro 4 d 20
################################################################################
#
# For methods that use the localized form of the "resolution of identity" for
# the two-electron Coulomb operator (RI_method LVL), particularly Hartree-Fock and
# hybrid density functional calculations, the highest accuracy can be obtained by
# uncommenting the line beginning with "for_aux"  below, thus adding an extra g radial
# function to the construction of the product basis set for the expansion.
# See Ref. New J. Phys. 17, 093020 (2015) for more information, particularly Figs. 1 and 6.
#
################################################################################
#
# for_aux hydro 5 g 6.0
```

## Nitrogen

```
################################################################################
#
#  FHI-aims code project
# Volker Blum, Fritz Haber Institute Berlin, 2009
#
#  Suggested "tight" defaults for N atom (to be pasted into control.in file)
#
################################################################################
  species        N
#     global species definitions
    nucleus             7
    mass                14.0067
#
    l_hartree           6
#
    cut_pot             4.0  2.0  1.0
    basis_dep_cutoff    1e-4
#
    radial_base         35 7.0
    radial_multiplier   2
    angular_grids       specified
      division   0.1841   50
      division   0.3514  110
      division   0.5126  194
```

```
      division   0.6292  302
      division   0.6939  434
#      division   0.7396  590
#      division   0.7632  770
#      division   0.8122  974
#      division   1.1604 1202
#      outer_grid  974
      outer_grid  434
################################################################################
#
#  Definition of "minimal" basis
#
################################################################################
#     valence basis states
    valence      2  s   2.
    valence      2  p   3.
#     ion occupancy
    ion_occ      2  s   1.
    ion_occ      2  p   2.
################################################################################
#
#  Suggested additional basis functions. For production calculations,
#  uncomment them one after another (the most important basis functions are
#  listed first).
#
#  Constructed for dimers: 1.0 A, 1.1 A, 1.5 A, 2.0 A, 3.0 A
#
################################################################################
#  "First tier" - improvements: -1193.42 meV to -220.60 meV
     hydro 2 p 1.8
     hydro 3 d 6.8
     hydro 3 s 5.8
#  "Second tier" - improvements: -80.21 meV to -6.86 meV
     hydro 4 f 10.8
     hydro 3 p 5.8
     hydro 1 s 0.8
     hydro 5 g 16
     hydro 3 d 4.9
#  "Third tier" - improvements: -4.29 meV to -0.53 meV
#     hydro 3 s 16
#     ionic 2 p auto
#     hydro 3 d 6.6
#     hydro 4 f 11.6
#  "Fourth tier" - improvements: -0.75 meV to -0.25 meV
#     hydro 2 p 4.5
#     hydro 2 s 2.4
#     hydro 5 g 14.4
#     hydro 4 d 14.4
#     hydro 4 f 16.8
# Further basis functions - -0.21 meV and below
#     hydro 3 p 14.8
#     hydro 3 s 4.4
#     hydro 3 d 19.6
#     hydro 5 g 12.8
################################################################################
#
# For methods that use the localized form of the "resolution of identity" for
# the two-electron Coulomb operator (RI_method LVL), particularly Hartree-Fock and
# hybrid density functional calculations, the highest accuracy can be obtained by
# uncommenting the line beginning with "for_aux"  below, thus adding an extra g radial
# function to the construction of the product basis set for the expansion.
```

```
# See Ref. New J. Phys. 17, 093020 (2015) for more information, particularly Figs. 1 and 6.
#
################################################################################
#
# for_aux hydro 5 g 6.0
```

## Oxygen

```
################################################################################
#
#  FHI-aims code project
# Volker Blum, Fritz Haber Institute Berlin, 2009
#
#  Suggested "tight" defaults for O atom (to be pasted into control.in file)
#
################################################################################
  species        O
#     global species definitions
    nucleus             8
    mass                15.9994
#
    l_hartree           6
#
    cut_pot             4.0  2.0  1.0
    basis_dep_cutoff    1e-4
#
    radial_base         36 7.0
    radial_multiplier   2
     angular_grids specified
      division   0.1817   50
      division   0.3417  110
      division   0.4949  194
      division   0.6251  302
      division   0.8014  434
#      division   0.8507  590
#      division   0.8762  770
#      division   0.9023  974
#      division   1.2339 1202
#      outer_grid 974
      outer_grid  434
################################################################################
#
#  Definition of "minimal" basis
#
################################################################################
#     valence basis states
    valence      2  s   2.
    valence      2  p   4.
#     ion occupancy
    ion_occ      2  s   1.
    ion_occ      2  p   3.
################################################################################
#
#  Suggested additional basis functions. For production calculations,
#  uncomment them one after another (the most important basis functions are
#  listed first).
#
#  Constructed for dimers: 1.0 A, 1.208 A, 1.5 A, 2.0 A, 3.0 A
#
################################################################################
#  "First tier" - improvements: -699.05 meV to -159.38 meV
```

```
     hydro 2 p 1.8
     hydro 3 d 7.6
     hydro 3 s 6.4
#  "Second tier" - improvements: -49.91 meV to -5.39 meV
     hydro 4 f 11.6
     hydro 3 p 6.2
     hydro 3 d 5.6
     hydro 5 g 17.6
     hydro 1 s 0.75
#  "Third tier" - improvements: -2.83 meV to -0.50 meV
#     ionic 2 p auto
#     hydro 4 f 10.8
#     hydro 4 d 4.7
#     hydro 2 s 6.8
#  "Fourth tier" - improvements: -0.40 meV to -0.12 meV
#     hydro 3 p 5
#     hydro 3 s 3.3
#     hydro 5 g 15.6
#     hydro 4 f 17.6
#     hydro 4 d 14
# Further basis functions - -0.08 meV and below
#     hydro 3 s 2.1
#     hydro 4 d 11.6
#     hydro 3 p 16
#     hydro 2 s 17.2
################################################################################
#
# For methods that use the localized form of the "resolution of identity" for
# the two-electron Coulomb operator (RI_method LVL), particularly Hartree-Fock and
# hybrid density functional calculations, the highest accuracy can be obtained by
# uncommenting the line beginning with "for_aux"  below, thus adding an extra g radial
# function to the construction of the product basis set for the expansion.
# See Ref. New J. Phys. 17, 093020 (2015) for more information, particularly Figs. 1 and 6.
#
################################################################################
#
# for_aux hydro 5 g 6.0
```

## Fluorine

```
################################################################################
#
#  FHI-aims code project
# Volker Blum, Fritz Haber Institute Berlin, 2009
#
#  Suggested "tight" defaults for F atom (to be pasted into control.in file)
#
################################################################################
  species        F
#     global species definitions
    nucleus             9
    mass                18.9984032
#
    l_hartree           6
#
    cut_pot             4.0  2.0  1.0
    basis_dep_cutoff    1e-4
#
    radial_base         37 7.0
    radial_multiplier   2
    angular_grids specified
```

```
      division   0.4014  110
      division   0.5291  194
      division   0.6019  302
      division   0.6814  434
#      division   0.7989  590
#      division   0.8965  770
#      division   1.3427  974
#      outer_grid   974
      outer_grid  434
################################################################################
#
#  Definition of "minimal" basis
#
################################################################################
#     valence basis states
    valence      2  s   2.
    valence      2  p   5.
#     ion occupancy
    ion_occ      2  s   1.
    ion_occ      2  p   4.
################################################################################
#
#  Suggested additional basis functions. For production calculations,
#  uncomment them one after another (the most important basis functions are
#  listed first).
#
#  Constructed for dimers: 1.2 A, 1.418 A, 1.75 A, 2.25 A, 3.25 A
#
################################################################################
#  "First tier" - improvements: -149.44 meV to -45.88 meV
     hydro 2 p 1.7
     hydro 3 d 7.4
     hydro 3 s 6.8
#  "Second tier" - improvements: -12.96 meV to -1.56 meV
     hydro 4 f 11.2
     ionic 2 p auto
     hydro 1 s 0.75
     hydro 4 d 8.8
     hydro 5 g 16.8
#  "Third tier" - improvements: -0.58 meV to -0.05 meV
#     hydro 3 p 6.2
#     hydro 3 s 3.2
#     hydro 4 f 9.6
#     hydro 3 s 19.6
#     hydro 4 d 8.6
#     hydro 5 g 14.4
# Further basis functions: -0.05 meV and below
#     hydro 3 p 4.2
################################################################################
#
# For methods that use the localized form of the "resolution of identity" for
# the two-electron Coulomb operator (RI_method LVL), particularly Hartree-Fock and
# hybrid density functional calculations, the highest accuracy can be obtained by
# uncommenting the line beginning with "for_aux"  below, thus adding an extra g radial
# function to the construction of the product basis set for the expansion.
# See Ref. New J. Phys. 17, 093020 (2015) for more information, particularly Figs. 1 and 6.
#
################################################################################
#
# for_aux hydro 5 g 6.0
```

## Silicon

```
################################################################################
#
#  FHI-aims code project
#  Volker Blum, Fritz Haber Institute Berlin, 2009
#
#  Suggested "tight" defaults for Si atom (to be pasted into control.in file)
#
#  Revised Jan 04, 2011, following tests (SiC) done by Lydia Nemec:
#     d and g functions of tier 2 now enabled by default.
#
################################################################################
  species        Si
#     global species definitions
    nucleus             14
    mass                28.0855
#
    l_hartree           6
#
    cut_pot             4.0          2.0  1.0
    basis_dep_cutoff    1e-4
#
    radial_base         42 7.0
    radial_multiplier   2
    angular_grids       specified
      division   0.4121   50
      division   0.7665  110
      division   1.0603  194
      division   1.2846  302
      division   1.4125  434
#      division   1.4810  590
#      division   1.5529  770
#      division   1.6284  974
#      division   2.6016 1202
#      outer_grid   974
      outer_grid  434
################################################################################
#
#  Definition of "minimal" basis
#
################################################################################
#     valence basis states
    valence      3  s   2.
    valence      3  p   2.
#     ion occupancy
    ion_occ      3  s   1.
    ion_occ      3  p   1.
################################################################################
#
#  Suggested additional basis functions. For production calculations,
#  uncomment them one after another (the most important basis functions are
#  listed first).
#
#  Constructed for dimers: 1.75 A, 2.0 A, 2.25 A, 2.75 A, 3.75 A
#
################################################################################
#  "First tier" - improvements: -571.96 meV to -37.03 meV
     hydro 3 d 4.2
     hydro 2 p 1.4
     hydro 4 f 6.2
```

```
     ionic 3 s auto
#  "Second tier" - improvements: -16.76 meV to -3.03 meV
     hydro 3 d 9
     hydro 5 g 9.4
     hydro 4 p 4
     hydro 1 s 0.65
#  "Third tier" - improvements: -3.89 meV to -0.60 meV
#     ionic 3 d auto
#     hydro 3 s 2.6
#     hydro 4 f 8.4
#     hydro 3 d 3.4
#     hydro 3 p 7.8
#  "Fourth tier" - improvements: -0.33 meV to -0.11 meV
#     hydro 2 p 1.6
#     hydro 5 g 10.8
#     hydro 5 f 11.2
#     hydro 3 d 1
#     hydro 4 s 4.5
#  Further basis functions that fell out of the optimization - noise
#  level... < -0.08 meV
#     hydro 4 d 6.6
#     hydro 5 g 16.4
#     hydro 4 d 9
################################################################################
#
# For methods that use the localized form of the "resolution of identity" for
# the two-electron Coulomb operator (RI_method LVL), particularly Hartree-Fock and
# hybrid density functional calculations, the highest accuracy can be obtained by
# uncommenting the line beginning with "for_aux"  below, thus adding an extra g radial
# function to the construction of the product basis set for the expansion.
# See Ref. New J. Phys. 17, 093020 (2015) for more information, particularly Figs. 1 and 6.
#
################################################################################
#
# for_aux hydro 5 g 6.0
```

## Phosphorus

```
################################################################################
#
#  FHI-aims code project
# Volker Blum, Fritz Haber Institute Berlin, 2010
#
#  Suggested "tight" defaults for P atom (to be pasted into control.in file)
#
#  Revised Jan 04, 2011, following tests (SiC) done by Lydia Nemec:
#     d function of tier 2 now enabled by default.
#
################################################################################
  species        P
#     global species definitions
    nucleus             15
    mass                30.973762
#
    l_hartree           6
#
    cut_pot             4.0          2.0  1.0
    basis_dep_cutoff    1e-4
#
    radial_base         43 7.0
    radial_multiplier   2
```

```
    angular_grids       specified
      division   0.2995   50
      division   0.5998  110
      division   0.9240  194
      division   1.0921  302
      division   1.2863  434
#      division   1.3165  590
#      division   1.4113  770
#      division   1.5128  974
#      division   2.4980 1202
      outer_grid  434
################################################################################
#
#  Definition of "minimal" basis
#
################################################################################
#     valence basis states
    valence      3  s   2.
    valence      3  p   3.
#     ion occupancy
    ion_occ      3  s   1.
    ion_occ      3  p   2.
################################################################################
#
#  Suggested additional basis functions. For production calculations,
#  uncomment them one after another (the most important basis functions are
#  listed first).
#
#  Constructed for dimers: 1.625 A, 1.875 A, 2.5 A, 3.25 A, 4.0 A
#
################################################################################
#  "First tier" - improvements: -726.20 meV to -35.91 meV
     ionic 3 d auto
     ionic 3 p auto
     hydro 4 f 6.2
     hydro 5 g 8.6
     ionic 3 s auto
#  "Second tier" - improvements: -16.02 meV to -1.71 meV
     hydro 4 d 6.2
     hydro 4 p 9.2
     hydro 5 f 9.8
     hydro 1 s 0.7
     hydro 5 g 13.2
#  "Third tier" - improvements: -1.82 meV to -0.20 meV
#     hydro 3 p 2.5
#     hydro 4 d 6.4
#     hydro 5 f 11.2
#     hydro 2 s 1.5
#  "Fourth tier" - improvements: -0.91 meV to -0.17 meV
#     hydro 3 d 16.8
#     hydro 5 g 18
#     hydro 4 p 4.5
#     hydro 3 s 2.1
#  Further basis functions that fell out of the optimization - < -0.09 meV
#     hydro 4 p 10.4
#     hydro 4 d 17.6
#     hydro 4 s 11.2
################################################################################
#
# For methods that use the localized form of the "resolution of identity" for
# the two-electron Coulomb operator (RI_method LVL), particularly Hartree-Fock and
```

```
# hybrid density functional calculations, the highest accuracy can be obtained by
# uncommenting the line beginning with "for_aux"  below, thus adding an extra g radial
# function to the construction of the product basis set for the expansion.
# See Ref. New J. Phys. 17, 093020 (2015) for more information, particularly Figs. 1 and 6.
#
################################################################################
#
# for_aux hydro 5 g 6.0
```

## Sulfur

```
################################################################################
#
#  FHI-aims code project
# Volker Blum, Fritz Haber Institute Berlin, 2009
#
#  Suggested "tight" defaults for S atom (to be pasted into control.in file)
#
#  Revised Jan 04, 2011, following tests (SiC) done by Lydia Nemec:
#     d and g functions of tier 2 now enabled by default.
#
################################################################################
  species        S
#     global species definitions
    nucleus             16
    mass                32.065
#
    l_hartree           6
#
    cut_pot             4.0          2.0  1.0
    basis_dep_cutoff    1e-4
#
    radial_base         44 7.0
    radial_multiplier   2
    angular_grids       specified
      division   0.4665  110
      division   0.5810  194
      division   0.7139  302
      division   0.8274  434
#      division   0.9105  590
#      division   1.0975  770
#      division   1.2028  974
#      outer_grid  974
      outer_grid  434
################################################################################
#
#  Definition of "minimal" basis
#
################################################################################
#     valence basis states
    valence      3  s   2.
    valence      3  p   4.
#     ion occupancy
    ion_occ      3  s   1.
    ion_occ      3  p   3.
################################################################################
#
#  Suggested additional basis functions. For production calculations,
#  uncomment them one after another (the most important basis functions are
#  listed first).
#
```

```
#  Constructed for dimers: 1.6 A, 1.9 A, 2.5 A, 3.25 A, 4.0 A
#
################################################################################
#  "First tier" - improvements: -652.81 meV to -45.53 meV
     ionic 3 d auto
     hydro 2 p 1.8
     hydro 4 f 7
     ionic 3 s auto
#  "Second tier" - improvements: -30.20 meV to -1.74 meV
     hydro 4 d 6.2
     hydro 5 g 10.8
     hydro 4 p 4.9
     hydro 5 f 10
     hydro 1 s 0.8
#  "Third tier" - improvements: -1.04 meV to -0.20 meV
#     hydro 3 d 3.9
#     hydro 3 d 2.7
#     hydro 5 g 12
#     hydro 4 p 10.4
#     hydro 5 f 12.4
#     hydro 2 s 1.9
#  "Fourth tier" - improvements: -0.35 meV to -0.06 meV
#     hydro 4 d 10.4
#     hydro 4 p 7.2
#     hydro 4 d 10
#     hydro 5 g 19.2
#     hydro 4 s 12

################################################################################
#
# For methods that use the localized form of the "resolution of identity" for
# the two-electron Coulomb operator (RI_method LVL), particularly Hartree-Fock and
# hybrid density functional calculations, the highest accuracy can be obtained by
# uncommenting the line beginning with "for_aux"  below, thus adding an extra g radial
# function to the construction of the product basis set for the expansion.
# See Ref. New J. Phys. 17, 093020 (2015) for more information, particularly Figs. 1 and 6.
#
################################################################################
#
# for_aux hydro 5 g 6.0
```

## Chlorine

```
################################################################################
#
#  FHI-aims code project
# Volker Blum, Fritz Haber Institute Berlin, 2009
#
#  Suggested "tight" defaults for Cl atom (to be pasted into control.in file)
#
#  Revised Jan 04, 2011, following tests (SiC) done by Lydia Nemec:
#     d function of tier 2 now enabled by default.
#
################################################################################
  species        Cl
#     global species definitions
    nucleus             17
    mass                35.453
#
    l_hartree           6
#
```

```
    cut_pot             4.0          2.0  1.0
    basis_dep_cutoff    1e-4
#
    radial_base         45 7.0
    radial_multiplier   2
    angular_grids       specified
      division   0.4412  110
      division   0.5489  194
      division   0.6734  302
      division   0.7794  434
#      division   0.9402  590
#      division   1.0779  770
#      division   1.1792  974
#      outer_grid  974
      outer_grid  434
################################################################################
#
#  Definition of "minimal" basis
#
################################################################################
#     valence basis states
    valence      3  s   2.
    valence      3  p   5.
#     ion occupancy
    ion_occ      3  s   1.
    ion_occ      3  p   4.
################################################################################
#
#  Suggested additional basis functions. For production calculations,
#  uncomment them one after another (the most important basis functions are
#  listed first).
#
#  Constructed for dimers: 1.65 A, 2.0 A, 2.5 A, 3.25 A, 4.0 A
#
################################################################################
#  "First tier" - improvements: -429.57 meV to -15.03 meV
     ionic 3 d auto
     hydro 2 p 1.9
     hydro 4 f 7.4
     ionic 3 s auto
     hydro 5 g 10.4
#  "Second tier" - improvements: -7.84 meV to -0.48 meV
     hydro 3 d 3.3
     hydro 5 f 9.8
     hydro 1 s 0.75
     hydro 5 g 11.2
     hydro 4 p 10.4
#  "Third tier" - improvements: -1.00 meV to -0.12 meV
#     hydro 4 d 12.8
#     hydro 4 f 4.6
#     hydro 4 d 10.8
#     hydro 2 s 1.8
#     hydro 3 p 3
#  Further functions that fell out - improvements: -0.10 meV and below
#     hydro 5 f 14.4
#     hydro 4 s 12.8
#     hydro 3 d 11.6
#     hydro 4 s 4.1
################################################################################
#
# For methods that use the localized form of the "resolution of identity" for
```

```
# the two-electron Coulomb operator (RI_method LVL), particularly Hartree-Fock and
# hybrid density functional calculations, the highest accuracy can be obtained by
# uncommenting the line beginning with "for_aux"  below, thus adding an extra g radial
# function to the construction of the product basis set for the expansion.
# See Ref. New J. Phys. 17, 093020 (2015) for more information, particularly Figs. 1 and 6.
#
################################################################################
#
# for_aux hydro 5 g 6.0
```

## u-pcJ-3 basis sets

Given in FHI-aims format. These large uncontracted gaussian basis sets have been constructed by uncontracting the pcJ-3 basis sets from F. Jensen, Theor. Chem. Acc. 126, 371 (2010). These have only been used to check that the numerical basis sets with additional core functions are suitable for the prediction of accurate core electron binding energies.

## Boron

```
# u-pcJ-3
  species        B
#     global species definitions
    nucleus             5
    mass                10.811
#
    l_hartree           8
#
    cut_pot             4.0  2.0  1.0
    basis_dep_cutoff    0.d0
#
    radial_base         32 7.0
    radial_multiplier   6
    angular_grids       specified
      division   0.3742  110
      division   0.5197  194
      division   0.5753  302
      division   0.7664  434
#      division   0.8392  770
#      division   1.6522  974
#      outer_grid   974
      outer_grid   590
################################################################################
#
#  Definition of "minimal" basis
#
################################################################################
#     valence basis states
    valence      2  s   2.
    valence      2  p   1.
#     ion occupancy
    ion_occ      2  s   1.

    include_min_basis   .false.
    pure_gauss          .true.

gaussian 0 1  0.179421E+08
gaussian 0 1  0.717685E+06
gaussian 0 1  0.574148E+05
gaussian 0 1  0.860153E+04
gaussian 0 1  0.195779E+04
gaussian 0 1  0.554611E+03
gaussian 0 1  0.181051E+03
```

```
gaussian 0 1  0.654909E+02
gaussian 0 1  0.255994E+02
gaussian 0 1  0.105323E+02
gaussian 0 1  0.444648E+01
gaussian 0 1  0.188320E+01
gaussian 0 1  0.698312E+00
gaussian 0 1  0.343100E+00
gaussian 0 1  0.142760E+00
gaussian 0 1  0.581574E-01
gaussian 1 1  0.585723E+03
gaussian 1 1  0.901112E+02
gaussian 1 1  0.211653E+02
gaussian 1 1  0.656183E+01
gaussian 1 1  0.256465E+01
gaussian 1 1  0.105104E+01
gaussian 1 1  0.451929E+00
gaussian 1 1  0.194682E+00
gaussian 1 1  0.832120E-01
gaussian 1 1  0.332973E-01
gaussian 2 1  0.2200000000E+02
gaussian 2 1  0.4000000000E+01
gaussian 2 1  0.1050000000E+01
gaussian 2 1  0.4000000000E+00
gaussian 2 1  0.1500000000E+00
gaussian 3 1  0.4200000000E+01
gaussian 3 1  0.1200000000E+01
gaussian 3 1  0.5200000000E+00
gaussian 4 1  0.1300000000E+01
```

## Carbon

```
# u-pcJ-3
  species        C
#     global species definitions
    nucleus             6
    mass                12.0107
#
    l_hartree           8
#
    cut_pot             4.0  2.0  1.0
    basis_dep_cutoff    0.d0
#
    radial_base         34 7.0
    radial_multiplier   6
    angular_grids specified
      division   0.4031  110
      division   0.5191  194
      division   0.6263  302
      division   0.8150  434
      division   0.8501  590
#     division   0.9238  770
#     division   1.6076  974
#     outer_grid  974
     outer_grid 590
################################################################################
#
#  Definition of "minimal" basis
#
################################################################################
#     valence basis states
    valence      2  s   2.
```

```
    valence      2  p   2.
#     ion occupancy
    ion_occ      2  s   1.
    ion_occ      2  p   1.

    include_min_basis   .false.
    pure_gauss          .true.

gaussian 0 1  0.272316E+08
gaussian 0 1  0.108927E+07
gaussian 0 1  0.871412E+05
gaussian 0 1  0.130520E+05
gaussian 0 1  0.297061E+04
gaussian 0 1  0.841460E+03
gaussian 0 1  0.274589E+03
gaussian 0 1  0.992150E+02
gaussian 0 1  0.386940E+02
gaussian 0 1  0.159109E+02
gaussian 0 1  0.676677E+01
gaussian 0 1  0.289837E+01
gaussian 0 1  0.112459E+01
gaussian 0 1  0.514464E+00
gaussian 0 1  0.211760E+00
gaussian 0 1  0.850172E-01
gaussian 1 1  0.963557E+03
gaussian 1 1  0.148240E+03
gaussian 1 1  0.349117E+02
gaussian 1 1  0.108936E+02
gaussian 1 1  0.419336E+01
gaussian 1 1  0.171343E+01
gaussian 1 1  0.735662E+00
gaussian 1 1  0.316374E+00
gaussian 1 1  0.132416E+00
gaussian 1 1  0.519006E-01
gaussian 2 1  0.2860000000E+02
gaussian 2 1  0.5200000000E+01
gaussian 2 1  0.1350000000E+01
gaussian 2 1  0.5200000000E+00
gaussian 2 1  0.2000000000E+00
gaussian 3 1  0.5250000000E+01
gaussian 3 1  0.1500000000E+01
gaussian 3 1  0.6500000000E+00
gaussian 4 1  0.1400000000E+01
```

## Nitrogen

```
# u-pcJ-3
  species        N
#     global species definitions
    nucleus             7
    mass                14.0067
#
    l_hartree           8
#
    cut_pot             4.0  2.0  1.0
    basis_dep_cutoff    0.d0
#
    radial_base         35 7.0
    radial_multiplier   6
    angular_grids       specified
      division   0.3806  110
```

```
      division   0.5126  194
      division   0.5309  302
      division   0.7632  434
#      division   0.7874  770
#      division   3.0496  974
#      outer_grid  974
      outer_grid  590
################################################################################
#
#  Definition of "minimal" basis
#
################################################################################
#     valence basis states
    valence      2  s   2.
    valence      2  p   3.
#     ion occupancy
    ion_occ      2  s   1.
    ion_occ      2  p   2.

    include_min_basis   .false.
    pure_gauss          .true.

gaussian 0 1  0.389206E+08
gaussian 0 1  0.155682E+07
gaussian 0 1  0.124546E+06
gaussian 0 1  0.186556E+05
gaussian 0 1  0.424506E+04
gaussian 0 1  0.120210E+04
gaussian 0 1  0.392142E+03
gaussian 0 1  0.141580E+03
gaussian 0 1  0.551359E+02
gaussian 0 1  0.226432E+02
gaussian 0 1  0.965655E+01
gaussian 0 1  0.416854E+01
gaussian 0 1  0.166780E+01
gaussian 0 1  0.745736E+00
gaussian 0 1  0.305157E+00
gaussian 0 1  0.120888E+00
gaussian 1 1  0.141886E+04
gaussian 1 1  0.218287E+03
gaussian 1 1  0.514884E+02
gaussian 1 1  0.161303E+02
gaussian 1 1  0.613074E+01
gaussian 1 1  0.250523E+01
gaussian 1 1  0.107298E+01
gaussian 1 1  0.458381E+00
gaussian 1 1  0.189481E+00
gaussian 1 1  0.733589E-01
gaussian 2 1  0.3300000000E+02
gaussian 2 1  0.6000000000E+01
gaussian 2 1  0.1650000000E+01
gaussian 2 1  0.6500000000E+00
gaussian 2 1  0.2500000000E+00
gaussian 3 1  0.6300000000E+01
gaussian 3 1  0.1800000000E+01
gaussian 3 1  0.7700000000E+00
gaussian 4 1  0.1500000000E+01
```

## Oxygen

```
# u-pcJ-3
```

```
  species        O
#     global species definitions
    nucleus             8
    mass                15.9994
#
    l_hartree           8
#
    cut_pot             4.0  2.0  1.0
    basis_dep_cutoff    0.d0
#
    radial_base         36 7.0
    radial_multiplier   6
     angular_grids specified
      division   0.4087  110
      division   0.5181  194
      division   0.6184  302
      division   0.7315  434
      division   0.7934  590
#      division   0.9656  770
#      division   1.4041  974
#      outer_grid 974
      outer_grid 590
################################################################################
#
#  Definition of "minimal" basis
#
################################################################################
#     valence basis states
    valence      2  s   2.
    valence      2  p   4.
#     ion occupancy
    ion_occ      2  s   1.
    ion_occ      2  p   3.

    include_min_basis   .false.
    pure_gauss          .true.

gaussian 0 1  0.512593E+08
gaussian 0 1  0.205037E+07
gaussian 0 1  0.164030E+06
gaussian 0 1  0.245674E+05
gaussian 0 1  0.559105E+04
gaussian 0 1  0.158362E+04
gaussian 0 1  0.516670E+03
gaussian 0 1  0.186555E+03
gaussian 0 1  0.726960E+02
gaussian 0 1  0.299924E+02
gaussian 0 1  0.128992E+02
gaussian 0 1  0.561355E+01
gaussian 0 1  0.229864E+01
gaussian 0 1  0.999797E+00
gaussian 0 1  0.407461E+00
gaussian 0 1  0.159225E+00
gaussian 1 1  0.176812E+04
gaussian 1 1  0.272018E+03
gaussian 1 1  0.642425E+02
gaussian 1 1  0.202494E+02
gaussian 1 1  0.764384E+01
gaussian 1 1  0.312320E+01
gaussian 1 1  0.132510E+01
gaussian 1 1  0.555508E+00
```

```
gaussian 1 1  0.222286E+00
gaussian 1 1  0.840097E-01
gaussian 2 1  0.3850000000E+02
gaussian 2 1  0.7000000000E+01
gaussian 2 1  0.2000000000E+01
gaussian 2 1  0.8000000000E+00
gaussian 2 1  0.3000000000E+00
gaussian 3 1  0.7350000000E+01
gaussian 3 1  0.2100000000E+01
gaussian 3 1  0.9000000000E+00
gaussian 4 1  0.1600000000E+01
```

## Fluorine

```
# u-pcJ-3
  species        F
#     global species definitions
    nucleus             9
    mass                18.9984032
#
    l_hartree           8
#
    cut_pot             4.0  2.0  1.0
    basis_dep_cutoff    0.d0
#
    radial_base         37 7.0
    radial_multiplier   6
    angular_grids specified
      division   0.4014  110
      division   0.5291  194
      division   0.6019  302
      division   0.6814  434
      division   0.7989  590
#      division   0.8965  770
#      division   1.3427  974
#      outer_grid   974
      outer_grid   590
################################################################################
#
#  Definition of "minimal" basis
#
################################################################################
#     valence basis states
    valence      2  s   2.
    valence      2  p   5.
#     ion occupancy
    ion_occ      2  s   1.
    ion_occ      2  p   4.

    include_min_basis   .false.
    pure_gauss          .true.

gaussian 0 1  0.673933E+08
gaussian 0 1  0.269573E+07
gaussian 0 1  0.215659E+06
gaussian 0 1  0.322991E+05
gaussian 0 1  0.735044E+04
gaussian 0 1  0.208182E+04
gaussian 0 1  0.679087E+03
gaussian 0 1  0.245100E+03
gaussian 0 1  0.954615E+02
```

```
gaussian 0 1  0.394224E+02
gaussian 0 1  0.170182E+02
gaussian 0 1  0.745246E+01
gaussian 0 1  0.313290E+01
gaussian 0 1  0.133946E+01
gaussian 0 1  0.542183E+00
gaussian 0 1  0.209037E+00
gaussian 1 1  0.228290E+04
gaussian 1 1  0.351216E+03
gaussian 1 1  0.829778E+02
gaussian 1 1  0.262671E+02
gaussian 1 1  0.993065E+01
gaussian 1 1  0.406700E+01
gaussian 1 1  0.172462E+01
gaussian 1 1  0.719760E+00
gaussian 1 1  0.286244E+00
gaussian 1 1  0.107890E+00
gaussian 2 1  0.4620000000E+02
gaussian 2 1  0.8400000000E+01
gaussian 2 1  0.2600000000E+01
gaussian 2 1  0.1000000000E+01
gaussian 2 1  0.3500000000E+00
gaussian 3 1  0.9100000000E+01
gaussian 3 1  0.2600000000E+01
gaussian 3 1  0.1050000000E+01
gaussian 4 1  0.1700000000E+01
```

## Silicon

```
# u-pcJ-3
  species        Si
#     global species definitions
    nucleus             14
    mass                28.0855
#
    l_hartree           8
#
    cut_pot             4.0          2.0  1.0
    basis_dep_cutoff    0.d0
#
    radial_base         42 7.0
    radial_multiplier   6
    angular_grids       specified
      division   0.5546  110
      division   0.6662  194
      division   0.7933  302
      division   0.9076  434
      division   1.0349  590
#      division   1.1770  770
#      division   2.4695  974
#      outer_grid   974
      outer_grid 590
################################################################################
#
#  Definition of "minimal" basis
#
################################################################################
#     valence basis states
    valence      3  s   2.
    valence      3  p   2.
#     ion occupancy
```

```
    ion_occ      3  s   1.
    ion_occ      3  p   1.

    include_min_basis   .false.
    pure_gauss          .true.

gaussian 0 1  0.274202E+09
gaussian 0 1  0.109681E+08
gaussian 0 1  0.877445E+06
gaussian 0 1  0.131448E+06
gaussian 0 1  0.299289E+05
gaussian 0 1  0.848016E+04
gaussian 0 1  0.276723E+04
gaussian 0 1  0.999396E+03
gaussian 0 1  0.390144E+03
gaussian 0 1  0.161910E+03
gaussian 0 1  0.703042E+02
gaussian 0 1  0.315787E+02
gaussian 0 1  0.144804E+02
gaussian 0 1  0.583828E+01
gaussian 0 1  0.259465E+01
gaussian 0 1  0.112498E+01
gaussian 0 1  0.353562E+00
gaussian 0 1  0.161600E+00
gaussian 0 1  0.672611E-01
gaussian 1 1  0.149703E+05
gaussian 1 1  0.230312E+04
gaussian 1 1  0.545845E+03
gaussian 1 1  0.177054E+03
gaussian 1 1  0.663775E+02
gaussian 1 1  0.276011E+02
gaussian 1 1  0.123430E+02
gaussian 1 1  0.568939E+01
gaussian 1 1  0.264060E+01
gaussian 1 1  0.120944E+01
gaussian 1 1  0.520126E+00
gaussian 1 1  0.232558E+00
gaussian 1 1  0.981411E-01
gaussian 1 1  0.383603E-01
gaussian 2 1  0.9990000000E+02
gaussian 2 1  0.6660000000E+01
gaussian 2 1  0.1750000000E+01
gaussian 2 1  0.5200000000E+00
gaussian 2 1  0.1900000000E+00
gaussian 3 1  0.2300000000E+02
gaussian 3 1  0.1150000000E+01
gaussian 3 1  0.3800000000E+00
gaussian 4 1  0.6500000000E+00
```

## Phosphorus

```
# u-pcJ-3
  species        P
#     global species definitions
    nucleus             15
    mass                30.973762
#
    l_hartree           8
#
    cut_pot             4.0          2.0  1.0
    basis_dep_cutoff    0.d0
```

```
#
    radial_base         43 7.0
    radial_multiplier   6
    angular_grids       specified
      division   0.5238  110
      division   0.6544  194
      division   0.7277  302
      division   0.8489  434
      division   0.9855  590
#      division   1.0863  770
#      division   2.6016  974
#      outer_grid  974
      outer_grid  590
################################################################################
#
#  Definition of "minimal" basis
#
################################################################################
#     valence basis states
    valence      3  s   2.
    valence      3  p   3.
#     ion occupancy
    ion_occ      3  s   1.
    ion_occ      3  p   2.

    include_min_basis   .false.
    pure_gauss          .true.

gaussian 0 1  0.332403E+09
gaussian 0 1  0.132961E+08
gaussian 0 1  0.106369E+07
gaussian 0 1  0.160001E+06
gaussian 0 1  0.365133E+05
gaussian 0 1  0.103592E+05
gaussian 0 1  0.338283E+04
gaussian 0 1  0.122229E+04
gaussian 0 1  0.477305E+03
gaussian 0 1  0.198087E+03
gaussian 0 1  0.859940E+02
gaussian 0 1  0.386272E+02
gaussian 0 1  0.176880E+02
gaussian 0 1  0.725513E+01
gaussian 0 1  0.326989E+01
gaussian 0 1  0.143127E+01
gaussian 0 1  0.470467E+00
gaussian 0 1  0.212895E+00
gaussian 0 1  0.877424E-01
gaussian 1 1  0.179542E+05
gaussian 1 1  0.276218E+04
gaussian 1 1  0.654784E+03
gaussian 1 1  0.212581E+03
gaussian 1 1  0.798946E+02
gaussian 1 1  0.333660E+02
gaussian 1 1  0.149865E+02
gaussian 1 1  0.696804E+01
gaussian 1 1  0.328178E+01
gaussian 1 1  0.152471E+01
gaussian 1 1  0.669237E+00
gaussian 1 1  0.299291E+00
gaussian 1 1  0.128110E+00
gaussian 1 1  0.509917E-01
```

```
gaussian 2 1  0.1156500000E+03
gaussian 2 1  0.7710000000E+01
gaussian 2 1  0.2030000000E+01
gaussian 2 1  0.6000000000E+00
gaussian 2 1  0.2200000000E+00
gaussian 3 1  0.2680000000E+02
gaussian 3 1  0.1340000000E+01
gaussian 3 1  0.4500000000E+00
gaussian 4 1  0.7200000000E+00
```

## Sulfur

```
# u-pcJ-3
  species        S
#     global species definitions
    nucleus             16
    mass                32.065
#
    l_hartree           8
#
    cut_pot             4.0          2.0  1.0
    basis_dep_cutoff    0.d0
#
    radial_base         44 7.0
    radial_multiplier   6
    angular_grids       specified
      division   0.4665  110
      division   0.5810  194
      division   0.7139  302
      division   0.8274  434
      division   0.9105  590
#      division   1.0975  770
#      division   1.2028  974
#      outer_grid  974
      outer_grid  590
################################################################################
#
#  Definition of "minimal" basis
#
################################################################################
#     valence basis states
    valence      3  s   2.
    valence      3  p   4.
#     ion occupancy
    ion_occ      3  s   1.
    ion_occ      3  p   3.

    include_min_basis   .false.
    pure_gauss          .true.

gaussian 0 1  0.390761E+09
gaussian 0 1  0.156305E+08
gaussian 0 1  0.125044E+07
gaussian 0 1  0.188077E+06
gaussian 0 1  0.429181E+05
gaussian 0 1  0.121790E+05
gaussian 0 1  0.397874E+04
gaussian 0 1  0.143814E+04
gaussian 0 1  0.561672E+03
gaussian 0 1  0.233113E+03
gaussian 0 1  0.101218E+03
```

```
gaussian 0 1  0.454926E+02
gaussian 0 1  0.208467E+02
gaussian 0 1  0.864916E+01
gaussian 0 1  0.394558E+01
gaussian 0 1  0.174718E+01
gaussian 0 1  0.599527E+00
gaussian 0 1  0.271272E+00
gaussian 0 1  0.110799E+00
gaussian 1 1  0.213577E+05
gaussian 1 1  0.328580E+04
gaussian 1 1  0.778928E+03
gaussian 1 1  0.252759E+03
gaussian 1 1  0.950996E+02
gaussian 1 1  0.398205E+02
gaussian 1 1  0.179253E+02
gaussian 1 1  0.836991E+01
gaussian 1 1  0.396547E+01
gaussian 1 1  0.185395E+01
gaussian 1 1  0.819709E+00
gaussian 1 1  0.361168E+00
gaussian 1 1  0.150974E+00
gaussian 1 1  0.596196E-01
gaussian 2 1  0.1314000000E+03
gaussian 2 1  0.8760000000E+01
gaussian 2 1  0.2300000000E+01
gaussian 2 1  0.6800000000E+00
gaussian 2 1  0.2500000000E+00
gaussian 3 1  0.3060000000E+02
gaussian 3 1  0.1530000000E+01
gaussian 3 1  0.5100000000E+00
gaussian 4 1  0.7900000000E+00
```

## Chlorine

```
# u-pcJ-3
  species        Cl
#     global species definitions
    nucleus             17
    mass                35.453
#
    l_hartree           8
#
    cut_pot             4.0          2.0  1.0
    basis_dep_cutoff    0.d0
#
    radial_base         45 7.0
    radial_multiplier   6
    angular_grids       specified
      division   0.4412  110
      division   0.5489  194
      division   0.6734  302
      division   0.7794  434
      division   0.9402  590
#      division   1.0779  770
#      division   1.1792  974
#      outer_grid  974
      outer_grid  590
################################################################################
#
#  Definition of "minimal" basis
#
```

```
################################################################################
#     valence basis states
    valence      3  s   2.
    valence      3  p   5.
#     ion occupancy
    ion_occ      3  s   1.
    ion_occ      3  p   4.

    include_min_basis   .false.
    pure_gauss          .true.

gaussian 0 1  0.456590E+09
gaussian 0 1  0.182636E+08
gaussian 0 1  0.146109E+07
gaussian 0 1  0.219593E+06
gaussian 0 1  0.500849E+05
gaussian 0 1  0.142058E+05
gaussian 0 1  0.463895E+04
gaussian 0 1  0.167635E+04
gaussian 0 1  0.654515E+03
gaussian 0 1  0.271526E+03
gaussian 0 1  0.117867E+03
gaussian 0 1  0.529838E+02
gaussian 0 1  0.242916E+02
gaussian 0 1  0.101841E+02
gaussian 0 1  0.469284E+01
gaussian 0 1  0.209736E+01
gaussian 0 1  0.748674E+00
gaussian 0 1  0.336135E+00
gaussian 0 1  0.135729E+00
gaussian 1 1  0.249969E+05
gaussian 1 1  0.384568E+04
gaussian 1 1  0.911226E+03
gaussian 1 1  0.295641E+03
gaussian 1 1  0.111403E+03
gaussian 1 1  0.467674E+02
gaussian 1 1  0.211061E+02
gaussian 1 1  0.990577E+01
gaussian 1 1  0.473468E+01
gaussian 1 1  0.223643E+01
gaussian 1 1  0.100711E+01
gaussian 1 1  0.443689E+00
gaussian 1 1  0.184880E+00
gaussian 1 1  0.732679E-01
gaussian 2 1  0.1471500000E+03
gaussian 2 1  0.9810000000E+01
gaussian 2 1  0.2580000000E+01
gaussian 2 1  0.7600000000E+00
gaussian 2 1  0.2800000000E+00
gaussian 3 1  0.3440000000E+02
gaussian 3 1  0.1720000000E+01
gaussian 3 1  0.5700000000E+00
gaussian 4 1  0.8600000000E+00
```

## A comparison of the results obtained using different basis sets

Supplementary Table 2: Calculated core electron binding energies using different basis sets

| Core level | Calculated core electron binding energy (eV) | | |
|---|---|---|---|
| | FHI-aims numerical | u-pcJ-3 | Difference |
| $B_2H_6$ B 1s | 196.401 | 196.403 | -0.002 |
| $CH_4$ C 1s | 290.782 | 290.773 | 0.009 |
| $NH_3$ N 1s | 405.707 | 405.677 | 0.030 |
| $H_2O$ O 1s | 539.884 | 539.874 | 0.010 |
| HF F 1s | 694.280 | 694.302 | -0.022 |
| $SiH_4$ Si 2p | 107.069 | 107.047 | 0.022 |
| $PH_3$ P $2p_{3/2}$ | 137.020 | 136.968 | 0.052 |
| H2S S $2p_{3/2}$ | 170.305 | 170.241 | 0.064 |
| HCl Cl $2p_{3/2}$ | 207.264 | 207.187 | 0.077 |

# The geometries of the clusters used for calculating core electron binding energies of adsorbates and solids

## CO on $Cu_{163}$

165
Atoms

| | | | |
|---|---|---|---|
| Cu3 | -0.00076782 | 1.474235439 | -6.200495248 |
| Cu3 | 2.545149151 | 1.474235467 | -6.200493764 |
| Cu3 | -2.543667365 | 5.873670262 | -6.197916157 |
| Cu3 | 2.545101369 | -2.940335734 | -6.197916157 |
| Cu3 | -0.000719597 | -2.940336988 | -6.197915002 |
| Cu3 | 5.088049137 | 5.873669008 | -6.197915002 |
| Cu3 | -6.355764015 | -0.73414428 | -6.19549722 |
| Cu3 | 3.821773454 | -0.73414428 | -6.19549722 |
| Cu3 | -1.27739006 | -0.734146579 | -6.19549586 |
| Cu3 | 5.090004079 | -2.934328807 | -6.192248842 |
| Cu3 | 0.001235345 | 5.879677189 | -6.192248842 |
| Cu3 | -5.08753339 | -2.934328807 | -6.192248842 |
| Cu3 | 2.543147909 | 5.879678025 | -6.19224692 |
| Cu3 | -2.545620825 | -2.934327971 | -6.19224692 |
| Cu3 | -5.088513101 | 1.46824686 | -6.191489688 |
| Cu3 | 5.089024368 | 1.46824686 | -6.191489688 |
| Cu3 | -2.544640443 | 1.468246621 | -6.19148871 |
| Cu3 | 7.632897026 | 1.468246621 | -6.19148871 |
| Cu3 | 1.272192467 | 3.674079874 | -6.191457308 |
| Cu3 | -3.816576267 | -5.139926122 | -6.191457308 |
| Cu3 | 1.27218847 | -0.733890811 | -6.19009126 |
| Cu3 | 3.814189291 | 3.673362406 | -6.187744895 |
| Cu3 | -1.274579443 | -5.14064359 | -6.187744895 |
| Cu3 | -1.269806257 | 3.673362705 | -6.187744129 |
| Cu3 | 3.818962477 | -5.140643291 | -6.187744129 |
| Cu3 | -3.816577554 | 3.671531878 | -6.186370546 |
| Cu3 | 6.360959915 | 3.671531878 | -6.186370546 |
| Cu3 | 1.27219118 | -5.142474118 | -6.186370546 |
| Cu3 | 6.360963031 | -0.73268129 | -6.184284541 |
| Cu3 | -3.816574438 | -0.73268129 | -6.184284541 |
| Cu3 | -2.541409846 | 7.353507977 | -4.143768435 |
| Cu3 | 2.547358888 | -1.460498019 | -4.143768435 |
| Cu3 | -7.630178581 | -1.460498019 | -4.143768435 |
| Cu3 | 5.085792068 | 7.353509451 | -4.14376721 |
| Cu3 | -0.002976666 | -1.460496545 | -4.14376721 |
| Cu3 | 1.272193963 | 0.743933182 | -4.143074109 |
| Cu3 | 6.360957732 | 0.748674192 | -4.13895892 |
| Cu3 | -3.816579737 | 0.748674192 | -4.13895892 |
| Cu3 | 6.360959649 | -3.662887444 | -4.137295009 |
| Cu3 | 1.272190914 | 5.151118552 | -4.137295009 |
| Cu3 | -3.81657782 | -3.662887444 | -4.137295009 |
| Cu3 | -5.088419047 | 2.946129847 | -4.135817361 |
| Cu3 | 0.000349688 | -5.867876149 | -4.135817361 |
| Cu3 | 5.089118422 | 2.946129847 | -4.135817361 |
| Cu3 | 2.54403344 | -5.867875988 | -4.13581552 |
| Cu3 | -2.544735294 | 2.946130008 | -4.13581552 |
| Cu3 | 7.632802175 | 2.946130008 | -4.13581552 |
| Cu3 | 3.816571672 | -3.662919142 | -4.135333055 |
| Cu3 | -1.272197062 | 5.151086854 | -4.135333055 |
| Cu3 | -6.360965797 | -3.662919142 | -4.135333055 |

| | | | |
|---|---|---|---|
| Cu3 | 3.816579636 | 5.151086786 | -4.135331277 |
| Cu3 | -1.272189098 | -3.66291921 | -4.135331277 |
| Cu3 | -1.262524489 | 0.739230832 | -4.134979682 |
| Cu3 | 8.91501298 | 0.739230832 | -4.134979682 |
| Cu3 | -6.370630625 | 0.739230943 | -4.134979397 |
| Cu3 | 3.806906844 | 0.739230943 | -4.134979397 |
| Cu3 | 1.272190603 | -3.655951223 | -4.134871447 |
| Cu3 | -3.816578131 | 5.158054773 | -4.134871447 |
| Cu3 | 6.360959337 | 5.158054773 | -4.134871447 |
| Cu3 | 5.088668987 | -5.870314183 | -4.134841384 |
| Cu3 | -5.088868481 | -5.870314183 | -4.134841384 |
| Cu3 | -9.9747e-05 | 2.943691813 | -4.134841384 |
| Cu3 | 2.54448289 | 2.94369293 | -4.134839724 |
| Cu3 | -2.544285844 | -5.870313066 | -4.134839724 |
| Cu3 | 0.000868176 | 7.353822172 | -4.130198752 |
| Cu3 | -5.087900559 | -1.460183824 | -4.130198752 |
| Cu3 | 5.08963691 | -1.460183824 | -4.130198752 |
| Cu3 | 7.632282864 | -1.460185026 | -4.130196163 |
| Cu3 | 2.543514129 | 7.35382097 | -4.130196163 |
| Cu3 | -2.545254605 | -1.460185026 | -4.130196163 |
| Cu1 | 2.540099795 | 8.810470115 | -2.103757197 |
| Cu1 | 7.62886853 | -0.003535881 | -2.103757197 |
| Cu1 | -2.548668939 | -0.003535881 | -2.103757197 |
| Cu1 | 5.09305431 | -0.003536166 | -2.103755725 |
| Cu1 | -5.084483159 | -0.003536166 | -2.103755725 |
| Cu1 | 0.004285576 | 8.81046983 | -2.103755725 |
| Cu1 | 2.544015698 | 4.395139172 | -2.10240081 |
| Cu1 | -2.544753036 | -4.418866824 | -2.10240081 |
| Cu1 | 7.632784432 | -4.418866824 | -2.10240081 |
| Cu1 | 0.000367056 | 4.395137273 | -2.10239911 |
| Cu1 | 5.08913579 | -4.418868723 | -2.10239911 |
| Cu1 | -5.088401678 | -4.418868723 | -2.10239911 |
| Cu1 | 3.822007649 | 2.193902917 | -2.101546773 |
| Cu1 | -1.266761085 | -6.620103079 | -2.101546773 |
| Cu1 | -6.35552982 | 2.193902917 | -2.101546773 |
| Cu1 | -6.366393865 | -6.620104248 | -2.101545105 |
| Cu1 | 8.899912338 | 2.193901748 | -2.101545105 |
| Cu1 | 3.811143603 | -6.620104248 | -2.101545105 |
| Cu1 | -1.277625131 | 2.193901748 | -2.101545105 |
| Cu1 | 6.360959833 | -6.630848021 | -2.098206209 |
| Cu1 | -3.816577635 | -6.630848021 | -2.098206209 |
| Cu1 | 1.272191099 | 2.183157975 | -2.098206209 |
| Cu1 | -1.278097524 | 6.606737565 | -2.096000559 |
| Cu1 | 3.81067121 | -2.207268431 | -2.096000559 |
| Cu1 | -6.366866259 | -2.207268431 | -2.096000559 |
| Cu1 | 8.911248271 | -2.207269466 | -2.095999255 |
| Cu1 | 3.822479536 | 6.60673653 | -2.095999255 |
| Cu1 | -1.266289198 | -2.207269466 | -2.095999255 |
| Cu1 | -2.543867882 | 4.401585419 | -2.095385949 |
| Cu1 | -7.632636616 | -4.412420577 | -2.095385949 |
| Cu1 | 7.633669587 | 4.401585419 | -2.095385949 |
| Cu1 | 2.544900852 | -4.412420577 | -2.095385949 |
| Cu1 | -5.089286233 | 4.401586061 | -2.095385193 |
| Cu1 | 5.088251236 | 4.401586061 | -2.095385193 |
| Cu1 | -0.000517498 | -4.412419935 | -2.095385193 |
| Cu1 | 6.360962257 | 2.199102483 | -2.095286265 |
| Cu1 | -3.816575212 | 2.199102483 | -2.095286265 |
| Cu1 | 1.272193522 | -6.614903513 | -2.095286265 |
| Cu1 | 6.360957401 | -2.212284627 | -2.092067316 |
| Cu1 | 1.272188666 | 6.601721369 | -2.092067316 |
| Cu1 | -3.816580068 | -2.212284627 | -2.092067316 |

| | | | |
|---|---|---|---|
| Cu1 | -8.905344457 | -2.200228316 | -2.081376213 |
| Cu1 | -3.816575722 | 6.61377768 | -2.081376213 |
| Cu1 | 6.360961746 | 6.61377768 | -2.081376213 |
| Cu1 | 1.272193012 | -2.200228316 | -2.081376213 |
| Cu1 | 2.537643637 | -0.015559919 | -2.079535438 |
| Cu1 | -2.551125097 | 8.798446077 | -2.079535438 |
| Cu1 | -7.639893832 | -0.015559919 | -2.079535438 |
| Cu1 | 10.184275645 | -0.015559225 | -2.079532636 |
| Cu1 | 0.006738176 | -0.015559225 | -2.079532636 |
| Cu1 | 5.09550691 | 8.798446771 | -2.079532636 |
| Cu2 | 2.561402914 | 1.495443514 | -0.052506729 |
| Cu2 | -0.017012938 | 1.495444311 | -0.052503112 |
| Cu1 | 10.160524531 | 1.495444311 | -0.052503112 |
| Cu1 | -6.331310791 | -0.737847117 | -0.051704229 |
| Cu1 | -1.242542056 | 8.076158879 | -0.051704229 |
| Cu2 | 3.846226678 | -0.737847117 | -0.051704229 |
| Cu1 | 8.875699028 | -0.737846824 | -0.051701969 |
| Cu1 | 3.786930293 | 8.076159172 | -0.051701969 |
| Cu2 | -1.301838441 | -0.737846824 | -0.051701969 |
| Cu1 | 5.069047651 | 5.847756011 | -0.051584695 |
| Cu2 | -0.019721083 | -2.966249985 | -0.051584695 |
| Cu1 | 7.652878313 | 5.847756214 | -0.051584641 |
| Cu1 | -7.61342789 | -2.966249782 | -0.051584641 |
| Cu2 | 2.564109579 | -2.966249782 | -0.051584641 |
| Cu1 | -2.524659155 | 5.847756214 | -0.051584641 |
| Cu1 | -3.81657838 | -5.139855037 | -0.044951761 |
| Cu1 | 6.360959088 | -5.139855037 | -0.044951761 |
| Cu2 | 1.272190354 | 3.674150959 | -0.044951761 |
| Cu1 | 1.272192855 | -5.144660052 | -0.043240001 |
| Cu1 | -3.816575879 | 3.669345944 | -0.043240001 |
| Cu1 | 6.36096159 | 3.669345944 | -0.043240001 |
| Cu2 | -2.551927403 | -2.943024773 | -0.041364601 |
| Cu2 | 2.536841331 | 5.870981223 | -0.041364601 |
| Cu1 | 7.625610066 | -2.943024773 | -0.041364601 |
| Cu2 | 0.007544579 | 5.87098077 | -0.041360513 |
| Cu1 | -5.081224156 | -2.943025226 | -0.041360513 |
| Cu2 | 5.096313313 | -2.943025226 | -0.041360513 |
| Cu1 | -5.082300635 | 1.468921528 | -0.040405588 |
| Cu2 | 5.095236834 | 1.468921528 | -0.040405588 |
| Cu1 | 7.626687138 | 1.468921204 | -0.040403011 |
| Cu2 | -2.550850331 | 1.468921204 | -0.040403011 |
| Cu2 | 3.82740592 | 3.669956505 | -0.035710543 |
| Cu1 | -1.261362814 | -5.144049491 | -0.035710543 |
| Cu1 | 3.805745196 | -5.144049508 | -0.035709792 |
| Cu2 | -1.283023538 | 3.669956488 | -0.035709792 |
| Cu1 | -6.371792272 | -5.144049508 | -0.035709792 |
| Cu1 | 8.894513931 | 3.669956488 | -0.035709792 |
| Cu2 | -3.81656756 | -0.735562798 | -0.035174086 |
| Cu2 | 6.360969909 | -0.735562798 | -0.035174086 |
| Cu1 | 1.272201174 | 8.078443198 | -0.035174086 |
| Cu2 | 1.272192 | -0.7345 | 0.011352187 |
| Cu1 | 6.360960734 | 8.079505996 | 0.011352187 |
| C | 1.272192 | -0.7345 | 1.846487463 |
| O | 1.272192 | -0.7345 | 3.000741735 |

## HCOO on $Cu_{163}$

167
Atoms

| | | | |
|---|---|---|---|
| Cu3 | -2.545078338 | 5.879089464 | -6.195325005 |
| Cu3 | 2.543690396 | -2.934916532 | -6.195325005 |

| | | | |
|---|---|---|---|
| Cu3 | 3.815455671 | 3.677497125 | -6.194751822 |
| Cu3 | -1.273313063 | -5.136508871 | -6.194751822 |
| Cu3 | 5.091170874 | 5.879871429 | -6.194241786 |
| Cu3 | 0.00240214 | -2.934134567 | -6.194241786 |
| Cu3 | -3.815787761 | -5.133510896 | -6.194126189 |
| Cu3 | 1.272980973 | 3.6804951 | -6.194126189 |
| Cu3 | -0.001363334 | 1.473058884 | -6.192750266 |
| Cu3 | 1.27168362 | -0.733596551 | -6.192316714 |
| Cu3 | 3.818092412 | -0.731071601 | -6.191467041 |
| Cu3 | -6.359445057 | -0.731071601 | -6.191467041 |
| Cu3 | 2.543717915 | 1.474192028 | -6.190870071 |
| Cu3 | -1.272273341 | -0.730555246 | -6.190263783 |
| Cu3 | 5.089110821 | -2.932898477 | -6.185615295 |
| Cu3 | -5.088426648 | -2.932898477 | -6.185615295 |
| Cu3 | 0.000342087 | 5.881107519 | -6.185615295 |
| Cu3 | 5.088425904 | 1.471720718 | -6.185422044 |
| Cu3 | -5.089111565 | 1.471720718 | -6.185422044 |
| Cu3 | -1.271066491 | 3.674962106 | -6.18214923 |
| Cu3 | 3.817702243 | -5.13904389 | -6.18214923 |
| Cu3 | 2.543251384 | 5.877963054 | -6.178734385 |
| Cu3 | -2.54551735 | -2.936042942 | -6.178734385 |
| Cu3 | -3.816455361 | -0.731648146 | -6.17808946 |
| Cu3 | 6.361082108 | -0.731648146 | -6.17808946 |
| Cu3 | -2.541420339 | 1.46964257 | -6.173196446 |
| Cu3 | 7.63611713 | 1.46964257 | -6.173196446 |
| Cu3 | 1.271195587 | -5.140183163 | -6.17163236 |
| Cu3 | 6.359964322 | 3.673822833 | -6.17163236 |
| Cu3 | -3.817573147 | 3.673822833 | -6.17163236 |
| Cu3 | 2.543151027 | 2.943496329 | -4.141605487 |
| Cu3 | -2.545617707 | -5.870509667 | -4.141605487 |
| Cu3 | 3.814522359 | -3.664979665 | -4.140820864 |
| Cu3 | -6.36301511 | -3.664979665 | -4.140820864 |
| Cu3 | -1.274246375 | 5.149026331 | -4.140820864 |
| Cu3 | 0.000894593 | -1.463677328 | -4.140003277 |
| Cu3 | 5.089663327 | 7.350328668 | -4.140003277 |
| Cu3 | 1.27281876 | 0.738632788 | -4.137649309 |
| Cu3 | -5.078448821 | -5.874041622 | -4.136713412 |
| Cu3 | 5.099088647 | -5.874041622 | -4.136713412 |
| Cu3 | 0.010319913 | 2.939964374 | -4.136713412 |
| Cu3 | 3.818970033 | 5.149321811 | -4.135932121 |
| Cu3 | -1.269798701 | -3.664684185 | -4.135932121 |
| Cu3 | 2.543775553 | -1.455623999 | -4.135232888 |
| Cu3 | -2.544993181 | 7.358381997 | -4.135232888 |
| Cu3 | -7.633761916 | -1.455623999 | -4.135232888 |
| Cu3 | 1.272828341 | 5.149561809 | -4.13438665 |
| Cu3 | 6.361597076 | -3.664444187 | -4.13438665 |
| Cu3 | -3.815940393 | -3.664444187 | -4.13438665 |
| Cu3 | -6.370074972 | 0.738600437 | -4.132877355 |
| Cu3 | 3.807462497 | 0.738600437 | -4.132877355 |
| Cu3 | 5.08677444 | -1.460734681 | -4.132344027 |
| Cu3 | -5.090763029 | -1.460734681 | -4.132344027 |
| Cu3 | -0.001994294 | 7.353271315 | -4.132344027 |
| Cu3 | -2.542504053 | -1.460003672 | -4.132284186 |
| Cu3 | 2.546264681 | 7.354002324 | -4.132284186 |
| Cu3 | 7.635033416 | -1.460003672 | -4.132284186 |
| Cu3 | -3.818286144 | 5.160291905 | -4.131619676 |
| Cu3 | 6.359251324 | 5.160291905 | -4.131619676 |
| Cu3 | 1.27048259 | -3.653714091 | -4.131619676 |
| Cu3 | 7.633990129 | 2.947291175 | -4.131422271 |
| Cu3 | -2.54354734 | 2.947291175 | -4.131422271 |
| Cu3 | 2.545221394 | -5.866714821 | -4.131422271 |

| | | | |
|---|---|---|---|
| Cu3 | -3.819612498 | 0.745604321 | -4.131130205 |
| Cu3 | 6.357924971 | 0.745604321 | -4.131130205 |
| Cu3 | -1.262648106 | 0.735372341 | -4.129725374 |
| Cu3 | 8.914889363 | 0.735372341 | -4.129725374 |
| Cu3 | 5.074283991 | 2.938464811 | -4.128076383 |
| Cu3 | -0.014484743 | -5.875541185 | -4.128076383 |
| Cu3 | -5.103253478 | 2.938464811 | -4.128076383 |
| Cu1 | -0.002691627 | 4.395200889 | -2.113712137 |
| Cu1 | -5.091460361 | -4.418805107 | -2.113712137 |
| Cu1 | 5.086077107 | -4.418805107 | -2.113712137 |
| Cu1 | -2.543530563 | -4.421305788 | -2.113475199 |
| Cu1 | 2.545238171 | 4.392700208 | -2.113475199 |
| Cu1 | 7.634006905 | -4.421305788 | -2.113475199 |
| Cu1 | 3.816715848 | -6.617358608 | -2.108178287 |
| Cu1 | 8.905484583 | 2.196647388 | -2.108178287 |
| Cu1 | -6.36082162 | -6.617358608 | -2.108178287 |
| Cu1 | -1.272052886 | 2.196647388 | -2.108178287 |
| Cu1 | 5.092277192 | 4.401107251 | -2.108143921 |
| Cu1 | -5.085260277 | 4.401107251 | -2.108143921 |
| Cu1 | 0.003508458 | -4.412898745 | -2.108143921 |
| Cu1 | 3.81602503 | -2.211528949 | -2.107816801 |
| Cu1 | -1.272743704 | 6.602477047 | -2.107816801 |
| Cu1 | -6.361512439 | -2.211528949 | -2.107816801 |
| Cu1 | -0.001875393 | 8.812057139 | -2.103839683 |
| Cu1 | 5.086893341 | -0.001948857 | -2.103839683 |
| Cu1 | -5.090644128 | -0.001948857 | -2.103839683 |
| Cu1 | 3.818207728 | 6.604565442 | -2.102407603 |
| Cu1 | -1.270561006 | -2.209440554 | -2.102407603 |
| Cu1 | 8.906976463 | -2.209440554 | -2.102407603 |
| Cu1 | 2.543761679 | 8.811550622 | -2.101996566 |
| Cu1 | -2.545007055 | -0.002455374 | -2.101996566 |
| Cu1 | 7.632530414 | -0.002455374 | -2.101996566 |
| Cu1 | 1.271555669 | -6.610009833 | -2.101478889 |
| Cu1 | 6.360324404 | 2.203996163 | -2.101478889 |
| Cu1 | -3.817213065 | 2.203996163 | -2.101478889 |
| Cu1 | 2.543880343 | -4.409936521 | -2.099145071 |
| Cu1 | -7.633657125 | -4.409936521 | -2.099145071 |
| Cu1 | -2.544888391 | 4.404069475 | -2.099145071 |
| Cu1 | 7.632649078 | 4.404069475 | -2.099145071 |
| Cu1 | 6.363299637 | -2.209450886 | -2.098047564 |
| Cu1 | -3.814237832 | -2.209450886 | -2.098047564 |
| Cu1 | 1.274530902 | 6.60455511 | -2.098047564 |
| Cu1 | 1.284171769 | 2.181477848 | -2.087733184 |
| Cu1 | -3.804596965 | -6.632528148 | -2.087733184 |
| Cu1 | 6.372940503 | -6.632528148 | -2.087733184 |
| Cu1 | 10.190808966 | -0.018769667 | -2.080367679 |
| Cu1 | 0.013271497 | -0.018769667 | -2.080367679 |
| Cu1 | 5.102040231 | 8.795236329 | -2.080367679 |
| Cu1 | 3.803510525 | 2.184102556 | -2.076924374 |
| Cu1 | -1.285258209 | -6.62990344 | -2.076924374 |
| Cu1 | -6.374026944 | 2.184102556 | -2.076924374 |
| Cu1 | -8.90542614 | -2.193843601 | -2.075123797 |
| Cu1 | 1.272111329 | -2.193843601 | -2.075123797 |
| Cu1 | -3.816657405 | 6.620162395 | -2.075123797 |
| Cu1 | 6.360880063 | 6.620162395 | -2.075123797 |
| Cu1 | 2.536041139 | -0.006805613 | -2.061433683 |
| Cu1 | -7.64149633 | -0.006805613 | -2.061433683 |
| Cu1 | -2.552727595 | 8.807200383 | -2.061433683 |
| Cu2 | -0.033899519 | 1.482245121 | -0.080681359 |
| Cu1 | 10.14363795 | 1.482245121 | -0.080681359 |
| Cu1 | -6.324215964 | -0.761058937 | -0.078208043 |

| | | | |
|---|---|---|---|
| Cu1 | -1.235447229 | 8.052947059 | -0.078208043 |
| Cu2 | 3.853321505 | -0.761058937 | -0.078208043 |
| Cu1 | -3.829485734 | -5.124184142 | -0.074246607 |
| Cu1 | 6.348051734 | -5.124184142 | -0.074246607 |
| Cu2 | 1.259283 | 3.689821854 | -0.074246607 |
| Cu1 | -1.251539116 | -5.120682336 | -0.068145599 |
| Cu2 | 3.837229618 | 3.69332366 | -0.068145599 |
| Cu1 | 7.650631748 | 5.852642912 | -0.068127812 |
| Cu1 | -7.615674455 | -2.961363084 | -0.068127812 |
| Cu2 | 2.561863014 | -2.961363084 | -0.068127812 |
| Cu1 | -2.52690572 | 5.852642912 | -0.068127812 |
| Cu1 | 5.063517177 | 5.845602389 | -0.06364488 |
| Cu2 | -0.025251557 | -2.968403607 | -0.06364488 |
| Cu1 | 3.787385305 | 8.068250968 | -0.061826563 |
| Cu1 | 8.87615404 | -0.745755028 | -0.061826563 |
| Cu2 | -1.301383429 | -0.745755028 | -0.061826563 |
| Cu1 | -5.059830825 | 1.464295569 | -0.058811468 |
| Cu2 | 5.117706644 | 1.464295569 | -0.058811468 |
| Cu1 | -6.371029999 | -5.148566522 | -0.045460367 |
| Cu2 | -1.282261265 | 3.665439474 | -0.045460367 |
| Cu1 | 3.806507469 | -5.148566522 | -0.045460367 |
| Cu1 | 8.895276204 | 3.665439474 | -0.045460367 |
| Cu2 | 5.099779122 | -2.942585023 | -0.04486358 |
| Cu1 | -5.077758347 | -2.942585023 | -0.04486358 |
| Cu2 | 0.011010388 | 5.871420973 | -0.04486358 |
| Cu1 | 1.275692052 | -5.144229025 | -0.044797914 |
| Cu1 | -3.813076682 | 3.669776971 | -0.044797914 |
| Cu1 | 6.364460787 | 3.669776971 | -0.044797914 |
| Cu2 | -2.548888336 | -2.945791599 | -0.044386542 |
| Cu2 | 2.539880398 | 5.868214397 | -0.044386542 |
| Cu1 | 7.628649133 | -2.945791599 | -0.044386542 |
| Cu2 | -2.546287574 | 1.466640482 | -0.040479623 |
| Cu1 | 7.631249895 | 1.466640482 | -0.040479623 |
| Cu2 | 6.363470758 | -0.738670814 | -0.039481306 |
| Cu1 | 1.274702023 | 8.075335182 | -0.039481306 |
| Cu2 | -3.814066711 | -0.738670814 | -0.039481306 |
| Cu2 | 2.559333233 | 1.493775322 | 0.012662949 |
| Cu2 | 1.252382524 | -0.766316693 | 0.025121599 |
| Cu1 | 6.341151258 | 8.047689303 | 0.025121599 |
| O | 2.502626686 | 1.354286273 | 2.006144426 |
| O | 1.34739253 | -0.608226786 | 2.019466141 |
| C | 1.928226272 | 0.374695495 | 2.568253774 |
| H | 1.933786843 | 0.378366457 | 3.679952026 |

## OH on $Cu_{163}$

165
Atoms

| | | | |
|---|---|---|---|
| Cu3 | 0.002364551 | -2.933851651 | -6.198299543 |
| Cu3 | 5.091133285 | 5.880154345 | -6.198299543 |
| Cu3 | 2.541883835 | -2.934694671 | -6.197373164 |
| Cu3 | -2.546884899 | 5.879311325 | -6.197373164 |
| Cu3 | -1.274350357 | -0.72837303 | -6.195601018 |
| Cu3 | -0.000792618 | 1.470712464 | -6.194778764 |
| Cu3 | 3.814746956 | -5.138288034 | -6.19437073 |
| Cu3 | -1.274021778 | 3.675717962 | -6.19437073 |
| Cu3 | 3.81960667 | -0.728298203 | -6.193758402 |
| Cu3 | -6.357930799 | -0.728298203 | -6.193758402 |
| Cu3 | 1.27223033 | 3.680379379 | -6.192869038 |
| Cu3 | -3.816538404 | -5.133626617 | -6.192869038 |
| Cu3 | 3.818580322 | 3.675797171 | -6.192521041 |

| | | | |
|---|---|---|---|
| Cu3 | -1.270188412 | -5.138208825 | -6.192521041 |
| Cu3 | 1.271426505 | -0.734660909 | -6.192199763 |
| Cu3 | 2.544040466 | 1.471173042 | -6.191918481 |
| Cu3 | 2.546349674 | 5.879976584 | -6.183196891 |
| Cu3 | -2.54241906 | -2.934029412 | -6.183196891 |
| Cu3 | 5.086941594 | -2.933461382 | -6.18263106 |
| Cu3 | -0.00182714 | 5.880544614 | -6.18263106 |
| Cu3 | -5.090595875 | -2.933461382 | -6.18263106 |
| Cu3 | 7.637410817 | 1.472729483 | -6.179285229 |
| Cu3 | -2.540126652 | 1.472729483 | -6.179285229 |
| Cu3 | -5.09168458 | 1.473559184 | -6.179214935 |
| Cu3 | 5.085852889 | 1.473559184 | -6.179214935 |
| Cu3 | -3.816554566 | -0.733464143 | -6.174816204 |
| Cu3 | 6.360982903 | -0.733464143 | -6.174816204 |
| Cu3 | 1.272042102 | -5.143078447 | -6.164112032 |
| Cu3 | 6.360810837 | 3.670927549 | -6.164112032 |
| Cu3 | -3.816726632 | 3.670927549 | -6.164112032 |
| Cu3 | 0.004481723 | 2.941363101 | -4.140334168 |
| Cu3 | 5.093250457 | -5.872642895 | -4.140334168 |
| Cu3 | -5.084287011 | -5.872642895 | -4.140334168 |
| Cu3 | -1.270049842 | -3.666029366 | -4.140193787 |
| Cu3 | 3.818718892 | 5.14797663 | -4.140193787 |
| Cu3 | 2.539588686 | 2.941258996 | -4.138734897 |
| Cu3 | -2.549180048 | -5.872747 | -4.138734897 |
| Cu3 | -1.274002693 | 5.148610125 | -4.138544285 |
| Cu3 | 3.814766041 | -3.665395871 | -4.138544285 |
| Cu3 | -6.362771428 | -3.665395871 | -4.138544285 |
| Cu3 | -2.543256295 | 7.355115335 | -4.137198616 |
| Cu3 | -7.63202503 | -1.458890661 | -4.137198616 |
| Cu3 | 2.545512439 | -1.458890661 | -4.137198616 |
| Cu3 | -0.00198405 | -1.458735772 | -4.136296019 |
| Cu3 | 5.086784684 | 7.355270224 | -4.136296019 |
| Cu3 | 6.36157013 | -3.665866906 | -4.136099292 |
| Cu3 | 1.272801395 | 5.14813909 | -4.136099292 |
| Cu3 | -3.815967339 | -3.665866906 | -4.136099292 |
| Cu3 | 1.271499925 | 0.738951047 | -4.135723383 |
| Cu3 | 7.635279237 | -1.462164052 | -4.131443438 |
| Cu3 | 2.546510502 | 7.351841944 | -4.131443438 |
| Cu3 | -2.542258232 | -1.462164052 | -4.131443438 |
| Cu3 | 6.360124484 | 5.160504503 | -4.130624436 |
| Cu3 | -3.817412984 | 5.160504503 | -4.130624436 |
| Cu3 | 1.27135575 | -3.653501493 | -4.130624436 |
| Cu3 | 5.087573025 | -1.461762326 | -4.129719541 |
| Cu3 | -0.001195709 | 7.35224367 | -4.129719541 |
| Cu3 | -5.089964444 | -1.461762326 | -4.129719541 |
| Cu3 | -1.266599514 | 0.737330212 | -4.129567905 |
| Cu3 | 8.910937955 | 0.737330212 | -4.129567905 |
| Cu3 | 3.811140976 | 0.738344712 | -4.12945254 |
| Cu3 | -6.366396493 | 0.738344712 | -4.12945254 |
| Cu3 | -3.815626623 | 0.744289607 | -4.129184725 |
| Cu3 | 6.361910846 | 0.744289607 | -4.129184725 |
| Cu3 | -2.528730914 | 2.938791313 | -4.124971227 |
| Cu3 | 2.56003782 | -5.875214683 | -4.124971227 |
| Cu3 | 7.648806555 | 2.938791313 | -4.124971227 |
| Cu3 | 5.073632166 | 2.939341576 | -4.122819254 |
| Cu3 | -5.103905303 | 2.939341576 | -4.122819254 |
| Cu3 | -0.015136568 | -5.87466442 | -4.122819254 |
| Cu1 | -0.005565057 | 4.391049082 | -2.116116184 |
| Cu1 | 5.083203677 | -4.422956914 | -2.116116184 |
| Cu1 | -5.094333791 | -4.422956914 | -2.116116184 |
| Cu1 | 2.549988909 | 4.391190711 | -2.116085934 |

| | | | |
|---|---|---|---|
| Cu1 | -2.538779825 | -4.422815285 | -2.116085934 |
| Cu1 | 7.638757643 | -4.422815285 | -2.116085934 |
| Cu1 | 8.906774762 | -2.212877723 | -2.106056892 |
| Cu1 | 3.818006027 | 6.601128273 | -2.106056892 |
| Cu1 | -1.270762707 | -2.212877723 | -2.106056892 |
| Cu1 | 6.362069168 | 2.206924584 | -2.105619057 |
| Cu1 | 1.273300433 | -6.607081412 | -2.105619057 |
| Cu1 | -3.815468301 | 2.206924584 | -2.105619057 |
| Cu1 | 3.815423683 | -2.211177049 | -2.104433007 |
| Cu1 | -6.362113786 | -2.211177049 | -2.104433007 |
| Cu1 | -1.273345051 | 6.602828947 | -2.104433007 |
| Cu1 | 2.540791086 | -4.411626465 | -2.103970655 |
| Cu1 | 7.629559821 | 4.402379531 | -2.103970655 |
| Cu1 | -2.547977648 | 4.402379531 | -2.103970655 |
| Cu1 | -7.636746382 | -4.411626465 | -2.103970655 |
| Cu1 | 0.00401763 | -4.410624445 | -2.10274045 |
| Cu1 | -5.084751105 | 4.403381551 | -2.10274045 |
| Cu1 | 5.092786364 | 4.403381551 | -2.10274045 |
| Cu1 | 2.545885325 | 8.811895889 | -2.098356043 |
| Cu1 | 7.63465406 | -0.002110107 | -2.098356043 |
| Cu1 | -2.542883409 | -0.002110107 | -2.098356043 |
| Cu1 | 5.087472918 | -0.001272708 | -2.097511521 |
| Cu1 | -0.001295816 | 8.812733288 | -2.097511521 |
| Cu1 | -5.090064551 | -0.001272708 | -2.097511521 |
| Cu1 | -3.816702753 | -2.211528855 | -2.093259554 |
| Cu1 | 6.360834716 | -2.211528855 | -2.093259554 |
| Cu1 | 1.272065981 | 6.602477141 | -2.093259554 |
| Cu1 | 6.360630386 | -6.634929658 | -2.077006739 |
| Cu1 | 1.271861652 | 2.179076338 | -2.077006739 |
| Cu1 | -3.816907082 | -6.634929658 | -2.077006739 |
| Cu1 | 8.918948629 | 2.187214257 | -2.07284501 |
| Cu1 | -6.347357574 | -6.626791739 | -2.07284501 |
| Cu1 | -1.25858884 | 2.187214257 | -2.07284501 |
| Cu1 | 3.830179894 | -6.626791739 | -2.07284501 |
| Cu1 | -6.373428946 | 2.188584512 | -2.072030899 |
| Cu1 | 3.804108523 | 2.188584512 | -2.072030899 |
| Cu1 | -1.284660211 | -6.625421484 | -2.072030899 |
| Cu1 | 5.099739548 | 8.811006936 | -2.071686346 |
| Cu1 | 10.188508283 | -0.00299906 | -2.071686346 |
| Cu1 | 0.010970814 | -0.00299906 | -2.071686346 |
| Cu1 | 1.272365056 | -2.197083841 | -2.070247326 |
| Cu1 | -8.905172413 | -2.197083841 | -2.070247326 |
| Cu1 | -3.816403678 | 6.616922155 | -2.070247326 |
| Cu1 | 6.36113379 | 6.616922155 | -2.070247326 |
| Cu1 | 2.534185383 | -0.002385281 | -2.069860811 |
| Cu1 | -2.554583351 | 8.811620715 | -2.069860811 |
| Cu1 | -7.643352086 | -0.002385281 | -2.069860811 |
| Cu2 | 1.271379404 | 3.705641693 | -0.086674796 |
| Cu1 | -3.81738933 | -5.108364303 | -0.086674796 |
| Cu1 | 6.360148138 | -5.108364303 | -0.086674796 |
| Cu1 | 8.865321149 | -0.766469477 | -0.067103258 |
| Cu2 | -1.31221632 | -0.766469477 | -0.067103258 |
| Cu1 | 3.776552414 | 8.047536519 | -0.067103258 |
| Cu1 | -1.235382046 | 8.051530032 | -0.066736252 |
| Cu1 | -6.324150781 | -0.762475964 | -0.066736252 |
| Cu2 | 3.853386688 | -0.762475964 | -0.066736252 |
| Cu1 | 7.65671697 | 5.849382954 | -0.047404966 |
| Cu1 | -2.520820498 | 5.849382954 | -0.047404966 |
| Cu1 | -7.609589233 | -2.964623042 | -0.047404966 |
| Cu2 | 2.567948236 | -2.964623042 | -0.047404966 |
| Cu2 | 3.84139885 | 3.692384343 | -0.04658767 |

| | | | |
|---|---|---|---|
| Cu1 | -1.247369884 | -5.121621653 | -0.04658767 |
| Cu1 | 5.064097657 | 5.847230877 | -0.046456672 |
| Cu2 | -0.024671077 | -2.966775119 | -0.046456672 |
| Cu2 | -1.296016833 | 3.689767757 | -0.046345535 |
| Cu1 | -6.384785567 | -5.124238239 | -0.046345535 |
| Cu1 | 3.792751901 | -5.124238239 | -0.046345535 |
| Cu1 | 8.881520636 | 3.689767757 | -0.046345535 |
| Cu2 | 5.120030545 | 1.470378658 | -0.044849099 |
| Cu1 | -5.057506924 | 1.470378658 | -0.044849099 |
| Cu1 | 7.604374613 | 1.469320568 | -0.043883536 |
| Cu2 | -2.573162856 | 1.469320568 | -0.043883536 |
| Cu2 | -3.816503072 | -0.739215716 | -0.038837577 |
| Cu1 | 1.272265662 | 8.07479028 | -0.038837577 |
| Cu2 | 6.361034397 | -0.739215716 | -0.038837577 |
| Cu1 | -3.814885677 | 3.674213915 | -0.038351665 |
| Cu1 | 6.362651792 | 3.674213915 | -0.038351665 |
| Cu1 | 1.273883057 | -5.139792081 | -0.038351665 |
| Cu2 | -2.554368288 | -2.945402298 | -0.038061463 |
| Cu2 | 2.534400446 | 5.868603698 | -0.038061463 |
| Cu1 | 7.623169181 | -2.945402298 | -0.038061463 |
| Cu2 | 0.010548797 | 5.870526948 | -0.038002168 |
| Cu2 | 5.099317531 | -2.943479048 | -0.038002168 |
| Cu1 | -5.078219938 | -2.943479048 | -0.038002168 |
| Cu2 | 2.652308082 | 1.520032235 | 0.010373088 |
| Cu2 | 1.273684853 | -0.847874459 | 0.010844196 |
| Cu1 | 6.362453587 | 7.966131537 | 0.010844196 |
| Cu1 | 10.074818679 | 1.517148608 | 0.012081334 |
| Cu2 | -0.10271879 | 1.517148608 | 0.012081334 |
| O | 1.276327077 | 0.745851606 | 1.268212748 |
| H | 1.283862321 | 0.750185879 | 2.248537114 |

## $H_2O$ layer on $Cu_{42}$

51

Atoms

| | | | |
|---|---|---|---|
| Cu1 | -1.299343473 | 0.688297277 | -4.224279948 |
| Cu1 | 2.516689645 | 2.899120874 | -4.223487537 |
| Cu1 | 1.232152905 | 0.687531419 | -4.220756946 |
| Cu1 | 3.787646415 | 0.700573956 | -4.21998939 |
| Cu1 | -0.030117846 | 2.900360981 | -4.212624691 |
| Cu1 | 2.505091081 | -1.517656633 | -4.206799217 |
| Cu1 | 1.246309463 | -3.714158588 | -4.205527275 |
| Cu1 | -2.559404367 | -1.510996678 | -4.199875132 |
| Cu1 | -0.021327293 | -1.521499495 | -4.199463054 |
| Cu1 | -1.29904096 | -3.706571977 | -4.197770384 |
| Cu1 | -1.308711545 | 2.139446214 | -2.202907659 |
| Cu1 | 1.252213796 | 2.145627632 | -2.201042378 |
| Cu1 | 2.517222422 | -0.048344387 | -2.200729964 |
| Cu1 | 5.069290686 | -0.042170779 | -2.194138528 |
| Cu1 | -3.848524519 | -2.251665519 | -2.183838789 |
| Cu1 | 2.506472207 | 4.351756845 | -2.181783382 |
| Cu1 | -2.582296527 | -4.462249151 | -2.181783382 |
| Cu1 | -0.042517824 | -0.071682338 | -2.173663283 |
| Cu1 | 3.792166071 | 2.144303782 | -2.169316451 |
| Cu1 | -0.028822769 | 4.350028793 | -2.167289027 |
| Cu1 | 3.785205478 | -2.262838896 | -2.164776534 |
| Cu1 | -0.021697783 | -4.455329444 | -2.155099 |
| Cu1 | -2.563849644 | -0.063231718 | -2.151871779 |
| Cu1 | 2.52457256 | -4.453178766 | -2.150130125 |
| Cu1 | 1.24801565 | -2.278282404 | -2.122003689 |
| Cu1 | -1.294142978 | -2.259100002 | -2.113865582 |

| | | | |
|---|---|---|---|
| Cu2 | -0.021590178 | 1.437056315 | -0.18555525 |
| Cu2 | 3.793931896 | -0.762430755 | -0.178356118 |
| Cu2 | 3.769473878 | 3.597953188 | -0.167931277 |
| Cu2 | -1.319294856 | -5.216052808 | -0.167931277 |
| Cu2 | 1.266094951 | -0.748563958 | -0.164956049 |
| Cu2 | 1.265408258 | -5.230501428 | -0.136422555 |
| Cu2 | -2.600307976 | 1.435127998 | -0.129159093 |
| Cu2 | -2.608583597 | -3.007343824 | -0.126974014 |
| Cu2 | -3.867315168 | -0.789070787 | -0.118435568 |
| Cu2 | -1.282385972 | 3.598641069 | -0.109047717 |
| Cu2 | 2.520747289 | 1.418386774 | -0.090896252 |
| Cu2 | 1.237543875 | 3.61563664 | -0.088154425 |
| Cu2 | 5.061784281 | 1.410153049 | -0.082658267 |
| Cu2 | -0.032840318 | -3.021869508 | -0.054260032 |
| Cu2 | 2.545077807 | -2.988238475 | -0.053884002 |
| Cu2 | -1.308342884 | -0.755611564 | -0.051373324 |
| O | -0.027327062 | -2.961408965 | 2.117991089 |
| H | 0.754204959 | 1.692051747 | 2.13615115 |
| O1 | -1.232992998 | -0.595385992 | 2.163122686 |
| H | -0.445865273 | -2.064669443 | 2.317761618 |
| H | 0.949433639 | -2.913230621 | 2.347522647 |
| H | -2.173005802 | -0.500244909 | 2.435263242 |
| H | -0.729800096 | 0.282249275 | 2.441496044 |
| H | -0.525298925 | 2.339685565 | 2.830780105 |
| O | 0.069990395 | 1.510267151 | 2.831015146 |

## $H_2O$ layer on $Cu_{88}$

106
Atoms

| | | | |
|---|---|---|---|
| O | -0.21309684 | -2.9080808 | 2.9582285 |
| O | 1.3702311 | 3.7619994 | 2.9066158 |
| H | 0.77494179 | 4.5914178 | 2.9063808 |
| O | 5.3932614 | 1.5389801 | 2.8704632 |
| H | 0.31324803 | -2.0901607 | 2.7190321 |
| H | 4.5263366 | 0.17765818 | 2.5493874 |
| H | 0.57044062 | 2.5339815 | 2.5170967 |
| H | 4.8739872 | 2.3035264 | 2.5149796 |
| H | -0.87276509 | 1.7514874 | 2.5108639 |
| H | 4.5205991 | -1.4335534 | 2.4994446 |
| H | 2.2496744 | -0.66149836 | 2.4231233 |
| H | 0.85437544 | 0.18706282 | 2.3933623 |
| O | 3.9684818 | -0.64339094 | 2.3029024 |
| H | -0.91847428 | -2.9514921 | 2.2642285 |
| O1 | 0.067247715 | 1.6563463 | 2.2387234 |
| H | 6.146552 | 1.500709 | 2.2190795 |
| H | 2.0544457 | 3.943784 | 2.2117518 |
| O | 1.2729137 | -0.70967671 | 2.1935918 |
| Cu2 | -0.008102171 | 1.4961207 | 0.024227366 |
| Cu2 | -6.332219 | -0.73650622 | 0.021716688 |
| Cu2 | 3.8453185 | -0.73650622 | 0.021716688 |
| Cu2 | 1.2674004 | -0.77013725 | 0.021340658 |
| Cu2 | 1.2732562 | -5.1521207 | -0.007057577 |
| Cu2 | -3.8155125 | 3.6618853 | -0.007057577 |
| Cu2 | 6.362025 | 3.6618853 | -0.007057577 |
| Cu2 | -2.5509841 | -2.9466371 | -0.012553735 |
| Cu2 | 2.5377846 | 5.8673689 | -0.012553735 |
| Cu2 | 3.820988 | 3.670119 | -0.015295562 |
| Cu2 | -1.2677807 | -5.143887 | -0.015295562 |
| Cu2 | -5.070914 | -2.9636327 | -0.033447027 |
| Cu2 | 0.017854766 | 5.8503733 | -0.033447027 |

| | | | |
|---|---|---|---|
| Cu2 | 5.1066235 | -2.9636327 | -0.033447027 |
| Cu2 | -2.5670745 | 1.4626615 | -0.042834878 |
| Cu2 | 7.610463 | 1.4626615 | -0.042834878 |
| Cu2 | -3.8005442 | -0.73955976 | -0.042970929 |
| Cu2 | 6.3769933 | -0.73955976 | -0.042970929 |
| Cu2 | -1.3083429 | -0.75561156 | -0.051373324 |
| Cu2 | -1.3000673 | 3.6868603 | -0.053558403 |
| Cu2 | 3.7887014 | -5.1271457 | -0.053558403 |
| Cu2 | -2.5231197 | 5.8352368 | -0.060821865 |
| Cu2 | 2.565649 | -2.9787692 | -0.060821865 |
| Cu2 | 2.5663357 | 1.5031683 | -0.089355359 |
| Cu2 | -0.019054143 | -2.9643205 | -0.092330587 |
| Cu2 | 5.0697146 | 5.8496855 | -0.092330587 |
| Cu2 | 5.0941726 | 1.4893015 | -0.10275543 |
| Cu2 | -5.0833649 | 1.4893015 | -0.10275543 |
| Cu2 | 1.2786505 | 3.6887886 | -0.10995456 |
| Cu2 | -3.8101182 | -5.1252174 | -0.10995456 |
| Cu1 | 0.006097735 | -0.007367742 | -2.0382649 |
| Cu1 | 2.5482564 | -0.026550144 | -2.046403 |
| Cu1 | -1.2639554 | 6.6125595 | -2.0745294 |
| Cu1 | 3.8248133 | -2.2014465 | -2.0745294 |
| Cu1 | -1.2636089 | 2.1885005 | -2.0762711 |
| Cu1 | 1.2785429 | -2.2035972 | -2.0794983 |
| Cu1 | -5.0920913 | -0.011106636 | -2.0891758 |
| Cu1 | 5.0854462 | -0.011106636 | -2.0891758 |
| Cu1 | -3.8173508 | -2.2122449 | -2.0916883 |
| Cu1 | 6.3601867 | -2.2122449 | -2.0916883 |
| Cu1 | 1.2714179 | 6.6017611 | -2.0916883 |
| Cu1 | 5.0924068 | 4.396036 | -2.0937158 |
| Cu1 | 0.003638066 | -4.41797 | -2.0937158 |
| Cu1 | 1.2577229 | 2.1800499 | -2.0980626 |
| Cu1 | -2.5527554 | 4.4041106 | -2.1025998 |
| Cu1 | 2.5360133 | -4.4098954 | -2.1025998 |
| Cu1 | 3.8067129 | 6.6034891 | -2.1061827 |
| Cu1 | -1.2820558 | -2.2105169 | -2.1061827 |
| Cu1 | -2.5482838 | 6.6741e-05 | -2.1082381 |
| Cu1 | 7.6292537 | 6.6741e-05 | -2.1082381 |
| Cu1 | 6.3695314 | 2.2095615 | -2.1185378 |
| Cu1 | -3.8080061 | 2.2095615 | -2.1185378 |
| Cu1 | 3.8174631 | 2.2033879 | -2.1251293 |
| Cu1 | -2.5363142 | -4.4166461 | -2.1254417 |
| Cu1 | 2.5524545 | 4.3973599 | -2.1254417 |
| Cu1 | -0.008470832 | 4.3911785 | -2.127307 |
| Cu1 | 5.0802979 | -4.4228275 | -2.127307 |
| Cu1 | 0.001199753 | -1.4548397 | -4.1221697 |
| Cu1 | 1.2789134 | 0.73023277 | -4.1238624 |
| Cu1 | -1.2591637 | 0.74073558 | -4.1242744 |
| Cu1 | 2.5465502 | -1.4624263 | -4.1299266 |
| Cu1 | 3.8053318 | 0.73407563 | -4.1311985 |
| Cu1 | 3.8186656 | -3.6550199 | -4.1312901 |
| Cu1 | -1.2701031 | 5.1589861 | -4.1312901 |
| Cu1 | 5.0883345 | -1.4592031 | -4.1336507 |
| Cu1 | -2.5466409 | -1.460365 | -4.1337052 |
| Cu1 | -2.5298387 | 2.9441776 | -4.1361324 |
| Cu1 | 1.2701228 | 5.1520932 | -4.137024 |
| Cu1 | 6.3531772 | 0.74530413 | -4.1370902 |
| Cu1 | -3.8243603 | 0.74530413 | -4.1370902 |
| Cu1 | 1.2720984 | -3.6542549 | -4.1397182 |
| Cu1 | 5.0878871 | 2.9523062 | -4.1443887 |
| Cu1 | 2.5323936 | 2.9392637 | -4.1451563 |
| Cu1 | 3.8169303 | 5.1508531 | -4.1478868 |

| | | | |
|---|---|---|---|
| Cu1 | -1.2718384 | -3.6631529 | -4.1478868 |
| Cu1 | 0.00089724 | 2.9400295 | -4.1486793 |
| Cu1 | -1.2698003 | -0.73066546 | -6.1809111 |
| Cu1 | -2.5395705 | 1.4693615 | -6.181616 |
| Cu1 | 5.0834333 | 1.4728463 | -6.1863838 |
| Cu1 | 3.8129855 | 3.678651 | -6.1882022 |
| Cu1 | 1.271877 | -0.73361753 | -6.1902918 |
| Cu1 | 0.002254778 | 1.4704062 | -6.1908016 |
| Cu1 | 3.8143664 | -0.73183611 | -6.1939976 |
| Cu1 | 0.001202717 | -2.9289915 | -6.197116 |
| Cu1 | 2.5418408 | 1.4724854 | -6.197573 |
| Cu1 | 2.5416578 | -2.9328591 | -6.1983888 |
| Cu1 | 1.2711131 | 3.6823332 | -6.2001023 |
| Cu1 | -1.2683739 | 3.6775691 | -6.2022893 |

## $H_2O$ layer on $Cu_{163}$

181
Atoms

| | | | |
|---|---|---|---|
| Cu3 | -1.26837394 | 3.677569142 | -6.202289324 |
| Cu3 | 3.820394794 | -5.136436854 | -6.202289324 |
| Cu3 | -3.817655672 | -5.131672751 | -6.20010234 |
| Cu3 | 1.271113062 | 3.682333245 | -6.20010234 |
| Cu3 | 2.541657784 | -2.932859075 | -6.198388798 |
| Cu3 | -2.54711095 | 5.881146921 | -6.198388798 |
| Cu3 | 2.541840815 | 1.472485394 | -6.197573003 |
| Cu3 | 0.001202717 | -2.928991481 | -6.197116037 |
| Cu3 | 5.089971451 | 5.885014515 | -6.197116037 |
| Cu3 | 2.545447212 | 5.880904409 | -6.194067378 |
| Cu3 | -2.543321522 | -2.933101587 | -6.194067378 |
| Cu3 | 3.814366431 | -0.731836107 | -6.19399757 |
| Cu3 | -6.363171038 | -0.731836107 | -6.19399757 |
| Cu3 | 0.002254778 | 1.470406214 | -6.190801576 |
| Cu3 | 1.271876986 | -0.733617527 | -6.190291787 |
| Cu3 | 5.088939976 | -2.936144575 | -6.19008283 |
| Cu3 | 0.000171242 | 5.877861421 | -6.19008283 |
| Cu3 | -5.088597493 | -2.936144575 | -6.19008283 |
| Cu3 | -1.275783251 | -5.135354993 | -6.18820218 |
| Cu3 | 3.812985483 | 3.678651003 | -6.18820218 |
| Cu3 | 5.083433286 | 1.472846342 | -6.186383812 |
| Cu3 | -5.094104183 | 1.472846342 | -6.186383812 |
| Cu3 | 6.360466959 | -0.732629808 | -6.184141269 |
| Cu3 | -3.81707051 | -0.732629808 | -6.184141269 |
| Cu3 | -3.81539076 | 3.675261867 | -6.183102071 |
| Cu3 | 1.273377974 | -5.138744129 | -6.183102071 |
| Cu3 | 6.362146709 | 3.675261867 | -6.183102071 |
| Cu3 | 7.637966929 | 1.469361518 | -6.181615973 |
| Cu3 | -2.53957054 | 1.469361518 | -6.181615973 |
| Cu3 | -1.269800275 | -0.730665457 | -6.180911135 |
| Cu3 | 0.00089724 | 2.940029537 | -4.148679258 |
| Cu3 | -5.087871494 | -5.873976459 | -4.148679258 |
| Cu3 | 5.089665974 | -5.873976459 | -4.148679258 |
| Cu3 | 3.816930358 | 5.150853134 | -4.147886847 |
| Cu3 | -1.271838376 | -3.663152862 | -4.147886847 |
| Cu3 | -2.556375116 | -5.874742317 | -4.145156256 |
| Cu3 | 2.532393618 | 2.939263679 | -4.145156256 |
| Cu3 | 5.087887128 | 2.952306216 | -4.1443887 |
| Cu3 | -0.000881606 | -5.86169978 | -4.1443887 |
| Cu3 | -5.089650341 | 2.952306216 | -4.1443887 |
| Cu3 | 1.272098394 | -3.654254877 | -4.139718228 |
| Cu3 | -3.81667034 | 5.159751119 | -4.139718228 |

| | | | |
|---|---|---|---|
| Cu3 | 6.360867128 | 5.159751119 | -4.139718228 |
| Cu3 | -3.824360312 | 0.745304129 | -4.137090168 |
| Cu3 | 6.353177157 | 0.745304129 | -4.137090168 |
| Cu3 | -3.818645867 | -3.661912755 | -4.137024001 |
| Cu3 | 6.358891602 | -3.661912755 | -4.137024001 |
| Cu3 | 1.270122867 | 5.152093241 | -4.137024001 |
| Cu3 | 2.558930053 | -5.869828391 | -4.136132377 |
| Cu3 | 7.647698788 | 2.944177605 | -4.136132377 |
| Cu3 | -2.529838681 | 2.944177605 | -4.136132377 |
| Cu3 | 2.542127832 | 7.353641031 | -4.133705157 |
| Cu3 | 7.630896567 | -1.460364965 | -4.133705157 |
| Cu3 | -2.546640902 | -1.460364965 | -4.133705157 |
| Cu3 | -0.000434242 | 7.354802866 | -4.133650707 |
| Cu3 | 5.088334492 | -1.45920313 | -4.133650707 |
| Cu3 | -5.089202977 | -1.45920313 | -4.133650707 |
| Cu3 | -1.270103139 | 5.158986116 | -4.131290097 |
| Cu3 | 3.818665595 | -3.65501988 | -4.131290097 |
| Cu3 | -6.358871874 | -3.65501988 | -4.131290097 |
| Cu3 | 3.805331794 | 0.734075627 | -4.131198527 |
| Cu3 | -6.372205675 | 0.734075627 | -4.131198527 |
| Cu3 | -2.542218558 | 7.351579668 | -4.129926585 |
| Cu3 | 2.546550176 | -1.462426328 | -4.129926585 |
| Cu3 | -7.630987293 | -1.462426328 | -4.129926585 |
| Cu3 | -1.259163654 | 0.740735582 | -4.124274442 |
| Cu3 | 8.918373815 | 0.740735582 | -4.124274442 |
| Cu3 | 1.27891342 | 0.730232765 | -4.123862364 |
| Cu3 | 0.001199753 | -1.454839717 | -4.122169694 |
| Cu3 | 5.089968487 | 7.359166279 | -4.122169694 |
| Cu1 | -5.097239566 | -4.422827522 | -2.127306969 |
| Cu1 | 5.080297902 | -4.422827522 | -2.127306969 |
| Cu1 | -0.008470832 | 4.391178474 | -2.127306969 |
| Cu1 | 2.552454509 | 4.397359892 | -2.125441688 |
| Cu1 | -2.536314225 | -4.416646104 | -2.125441688 |
| Cu1 | 7.641223243 | -4.416646104 | -2.125441688 |
| Cu1 | 3.817463135 | 2.203387873 | -2.125129274 |
| Cu1 | -6.360074334 | 2.203387873 | -2.125129274 |
| Cu1 | -1.271305599 | -6.610618123 | -2.125129274 |
| Cu1 | 1.280762664 | -6.604444515 | -2.118537838 |
| Cu1 | 6.369531399 | 2.209561481 | -2.118537838 |
| Cu1 | -3.80800607 | 2.209561481 | -2.118537838 |
| Cu1 | 2.540484928 | 8.814072737 | -2.108238099 |
| Cu1 | -2.548283806 | 6.6741e-05 | -2.108238099 |
| Cu1 | 7.629253663 | 6.6741e-05 | -2.108238099 |
| Cu1 | -1.282055814 | -2.210516891 | -2.106182692 |
| Cu1 | 3.80671292 | 6.603489105 | -2.106182692 |
| Cu1 | 8.895481655 | -2.210516891 | -2.106182692 |
| Cu1 | -2.552755413 | 4.40411062 | -2.102599789 |
| Cu1 | -7.641524147 | -4.409895376 | -2.102599789 |
| Cu1 | 2.536013321 | -4.409895376 | -2.102599789 |
| Cu1 | 7.624782056 | 4.40411062 | -2.102599789 |
| Cu1 | -3.831045845 | -6.633956074 | -2.098062593 |
| Cu1 | 1.257722889 | 2.180049922 | -2.098062593 |
| Cu1 | 6.346491623 | -6.633956074 | -2.098062593 |
| Cu1 | 0.00363805 | -4.417969954 | -2.093715761 |
| Cu1 | -5.085130685 | 4.396036042 | -2.093715761 |
| Cu1 | 5.092406784 | 4.396036042 | -2.093715761 |
| Cu1 | 1.271417944 | 6.601761053 | -2.091688337 |
| Cu1 | 6.360186679 | -2.212244943 | -2.091688337 |
| Cu1 | -3.81735079 | -2.212244943 | -2.091688337 |
| Cu1 | -0.003322543 | 8.80289936 | -2.089175844 |
| Cu1 | -5.092091278 | -0.011106636 | -2.089175844 |

| | | | |
|---|---|---|---|
| Cu1 | 5.085446191 | -0.011106636 | -2.089175844 |
| Cu1 | 1.27854293 | -2.203597184 | -2.07949831 |
| Cu1 | -8.898994539 | -2.203597184 | -2.07949831 |
| Cu1 | 6.367311664 | 6.610408812 | -2.07949831 |
| Cu1 | -3.810225804 | 6.610408812 | -2.07949831 |
| Cu1 | -6.352377665 | -6.625505454 | -2.076271089 |
| Cu1 | 3.825159803 | -6.625505454 | -2.076271089 |
| Cu1 | 8.913928538 | 2.188500542 | -2.076271089 |
| Cu1 | -1.263608931 | 2.188500542 | -2.076271089 |
| Cu1 | 3.824813273 | -2.201446506 | -2.074529435 |
| Cu1 | -6.352724196 | -2.201446506 | -2.074529435 |
| Cu1 | -1.263955461 | 6.61255949 | -2.074529435 |
| Cu1 | 2.548256363 | -0.026550144 | -2.046402999 |
| Cu1 | -2.540512371 | 8.787455852 | -2.046402999 |
| Cu1 | -7.629281106 | -0.026550144 | -2.046402999 |
| Cu1 | 10.183635204 | -0.007367742 | -2.038264892 |
| Cu1 | 5.094866469 | 8.806638254 | -2.038264892 |
| Cu1 | 0.006097735 | -0.007367742 | -2.038264892 |
| Cu1 | 6.367419269 | -5.125217421 | -0.10995456 |
| Cu1 | -3.810118199 | -5.125217421 | -0.10995456 |
| Cu2 | 1.278650535 | 3.688788575 | -0.10995456 |
| Cu1 | -5.08336486 | 1.489301505 | -0.102755428 |
| Cu2 | 5.094172609 | 1.489301505 | -0.102755428 |
| Cu1 | 5.069714591 | 5.849685448 | -0.092330587 |
| Cu2 | -0.019054143 | -2.964320548 | -0.092330587 |
| Cu2 | 2.566335664 | 1.503168302 | -0.089355359 |
| Cu1 | -7.611888498 | -2.978769168 | -0.060821865 |
| Cu1 | -2.523119763 | 5.835236828 | -0.060821865 |
| Cu1 | 7.654417705 | 5.835236828 | -0.060821865 |
| Cu2 | 2.565648971 | -2.978769168 | -0.060821865 |
| Cu1 | -6.388835997 | -5.127145738 | -0.053558403 |
| Cu1 | 3.788701471 | -5.127145738 | -0.053558403 |
| Cu1 | 8.877470206 | 3.686860258 | -0.053558403 |
| Cu2 | -1.300067263 | 3.686860258 | -0.053558403 |
| Cu1 | 8.869194585 | -0.755611564 | -0.051373324 |
| Cu2 | -1.308342884 | -0.755611564 | -0.051373324 |
| Cu1 | 3.78042585 | 8.058394432 | -0.051373324 |
| Cu2 | 6.376993287 | -0.739559765 | -0.042970929 |
| Cu1 | 1.288224552 | 8.074446231 | -0.042970929 |
| Cu2 | -3.800544182 | -0.739559765 | -0.042970929 |
| Cu1 | 7.610463014 | 1.462661473 | -0.042834878 |
| Cu2 | -2.567074455 | 1.462661473 | -0.042834878 |
| Cu1 | -5.070913994 | -2.963632667 | -0.033447027 |
| Cu2 | 0.017854741 | 5.850373329 | -0.033447027 |
| Cu2 | 5.106623475 | -2.963632667 | -0.033447027 |
| Cu1 | -1.267780732 | -5.143886962 | -0.015295562 |
| Cu2 | 3.820988002 | 3.670119034 | -0.015295562 |
| Cu2 | -2.550984146 | -2.946637096 | -0.012553735 |
| Cu1 | 7.626553323 | -2.946637096 | -0.012553735 |
| Cu2 | 2.537784588 | 5.8673689 | -0.012553735 |
| Cu1 | -3.815512475 | 3.661885309 | -0.007057577 |
| Cu1 | 6.362024994 | 3.661885309 | -0.007057577 |
| Cu1 | 1.273256259 | -5.152120687 | -0.007057577 |
| Cu1 | 6.356169129 | 8.043868748 | 0.021340658 |
| Cu2 | 1.267400395 | -0.770137248 | 0.021340658 |
| Cu1 | -6.332218949 | -0.736506215 | 0.021716688 |
| Cu1 | -1.243450214 | 8.077499781 | 0.021716688 |
| Cu2 | 3.84531852 | -0.736506215 | 0.021716688 |
| Cu1 | 10.169435298 | 1.496120696 | 0.024227366 |
| Cu2 | -0.008102171 | 1.496120696 | 0.024227366 |
| O | 1.272913651 | -0.709676705 | 2.193591779 |

| | | | |
|---|---|---|---|
| H | 2.054445672 | 3.943784007 | 2.21175184 |
| H | 6.14655201 | 1.500709033 | 2.21907952 |
| O1 | 0.067247715 | 1.656346268 | 2.238723376 |
| H | -0.91847428 | -2.951492146 | 2.264228538 |
| O | 3.968481841 | -0.643390944 | 2.302902383 |
| H | 0.85437544 | 0.187062817 | 2.393362308 |
| H | 2.249674352 | -0.661498361 | 2.423123337 |
| H | 4.520599128 | -1.433553363 | 2.49944461 |
| H | -0.872765089 | 1.751487351 | 2.510863932 |
| H | 4.873987228 | 2.303526432 | 2.514979609 |
| H | 0.570440617 | 2.533981535 | 2.517096734 |
| H | 4.526336606 | 0.177658185 | 2.549387373 |
| H | 0.313248026 | -2.090160687 | 2.719032089 |
| O | 5.393261367 | 1.538980102 | 2.870463157 |
| H | 0.774941788 | 4.591417825 | 2.906380795 |
| O | 1.370231108 | 3.761999411 | 2.906615836 |
| O | -0.213096839 | -2.908080758 | 2.958228458 |

## $H_2O$ layer on $Cu_{292}$

310
Atoms

| | | | |
|---|---|---|---|
| Cu3 | 3.820394794 | -5.136436854 | -6.202289324 |
| Cu3 | 8.909163529 | 3.677569142 | -6.202289324 |
| Cu3 | -6.357142674 | -5.136436854 | -6.202289324 |
| Cu3 | -1.26837394 | 3.677569142 | -6.202289324 |
| Cu3 | 6.359881796 | -5.131672751 | -6.20010234 |
| Cu3 | -3.817655672 | -5.131672751 | -6.20010234 |
| Cu3 | 11.448650531 | 3.682333245 | -6.20010234 |
| Cu3 | 1.271113062 | 3.682333245 | -6.20010234 |
| Cu3 | 2.541657784 | -2.932859075 | -6.198388798 |
| Cu3 | 7.630426518 | 5.881146921 | -6.198388798 |
| Cu3 | -7.635879685 | -2.932859075 | -6.198388798 |
| Cu3 | -2.54711095 | 5.881146921 | -6.198388798 |
| Cu3 | 12.719378284 | 1.472485394 | -6.197573003 |
| Cu3 | 2.541840815 | 1.472485394 | -6.197573003 |
| Cu3 | -7.635696654 | 1.472485394 | -6.197573003 |
| Cu3 | 7.630609549 | 10.28649139 | -6.197573003 |
| Cu3 | -2.546927919 | 10.28649139 | -6.197573003 |
| Cu3 | -2.546927919 | -7.341520602 | -6.197573003 |
| Cu3 | 7.630609549 | -7.341520602 | -6.197573003 |
| Cu3 | 10.178740186 | -2.928991481 | -6.197116037 |
| Cu3 | -5.087566017 | 5.885014515 | -6.197116037 |
| Cu3 | -10.176334752 | -2.928991481 | -6.197116037 |
| Cu3 | 0.001202717 | -2.928991481 | -6.197116037 |
| Cu3 | 5.089971451 | 5.885014515 | -6.197116037 |
| Cu3 | 2.545447212 | 5.880904409 | -6.194067378 |
| Cu3 | 7.634215947 | -2.933101587 | -6.194067378 |
| Cu3 | -2.543321522 | -2.933101587 | -6.194067378 |
| Cu3 | -6.363171038 | -0.731836107 | -6.19399757 |
| Cu3 | 3.814366431 | -0.731836107 | -6.19399757 |
| Cu3 | -1.274402303 | 8.082169889 | -6.19399757 |
| Cu3 | 8.903135165 | 8.082169889 | -6.19399757 |
| Cu3 | -5.086513956 | -7.343599782 | -6.190801576 |
| Cu3 | 10.179792247 | 1.470406214 | -6.190801576 |
| Cu3 | 5.091023512 | 10.28441221 | -6.190801576 |
| Cu3 | 5.091023512 | -7.343599782 | -6.190801576 |
| Cu3 | 0.002254778 | 1.470406214 | -6.190801576 |
| Cu3 | -3.816891748 | 8.080388469 | -6.190291787 |
| Cu3 | 1.271876986 | -0.733617527 | -6.190291787 |
| Cu3 | -8.905660483 | -0.733617527 | -6.190291787 |

| | | | |
|---|---|---|---|
| Cu3 | 11.449414455 | -0.733617527 | -6.190291787 |
| Cu3 | 6.36064572 | 8.080388469 | -6.190291787 |
| Cu3 | 10.17770871 | 5.877861421 | -6.19008283 |
| Cu3 | 0.000171242 | 5.877861421 | -6.19008283 |
| Cu3 | 5.088939976 | -2.936144575 | -6.19008283 |
| Cu3 | -5.088597493 | -2.936144575 | -6.19008283 |
| Cu3 | 8.901754217 | -5.135354993 | -6.18820218 |
| Cu3 | -6.364551986 | 3.678651003 | -6.18820218 |
| Cu3 | -1.275783251 | -5.135354993 | -6.18820218 |
| Cu3 | 3.812985483 | 3.678651003 | -6.18820218 |
| Cu3 | 5.083433286 | 1.472846342 | -6.186383812 |
| Cu3 | -0.005335448 | 10.286852338 | -6.186383812 |
| Cu3 | -0.005335448 | -7.341159654 | -6.186383812 |
| Cu3 | -5.094104183 | 1.472846342 | -6.186383812 |
| Cu3 | 1.271698224 | 8.081376188 | -6.184141269 |
| Cu3 | -3.81707051 | -0.732629808 | -6.184141269 |
| Cu3 | 6.360466959 | -0.732629808 | -6.184141269 |
| Cu3 | 1.273377974 | -5.138744129 | -6.183102071 |
| Cu3 | -3.81539076 | 3.675261867 | -6.183102071 |
| Cu3 | -8.904159494 | -5.138744129 | -6.183102071 |
| Cu3 | 6.362146709 | 3.675261867 | -6.183102071 |
| Cu3 | -7.628339274 | -7.344644478 | -6.181615973 |
| Cu3 | 7.637966929 | 1.469361518 | -6.181615973 |
| Cu3 | 2.549198194 | 10.283367514 | -6.181615973 |
| Cu3 | -2.53957054 | 1.469361518 | -6.181615973 |
| Cu3 | 2.549198194 | -7.344644478 | -6.181615973 |
| Cu3 | -1.269800275 | -0.730665457 | -6.180911135 |
| Cu3 | 8.907737194 | -0.730665457 | -6.180911135 |
| Cu3 | 3.818968459 | 8.083340539 | -6.180911135 |
| Cu3 | 5.089665974 | -5.873976459 | -4.148679258 |
| Cu3 | -5.087871494 | -5.873976459 | -4.148679258 |
| Cu3 | 10.178434709 | 2.940029537 | -4.148679258 |
| Cu3 | 5.089665974 | 11.754035533 | -4.148679258 |
| Cu3 | 0.00089724 | 2.940029537 | -4.148679258 |
| Cu3 | 3.816930358 | 5.150853134 | -4.147886847 |
| Cu3 | -1.271838376 | -3.663152862 | -4.147886847 |
| Cu3 | 8.905699093 | -3.663152862 | -4.147886847 |
| Cu3 | -11.449375845 | -3.663152862 | -4.147886847 |
| Cu3 | -6.36060711 | 5.150853134 | -4.147886847 |
| Cu3 | -7.645143851 | 2.939263679 | -4.145156256 |
| Cu3 | 7.621162352 | 11.753269675 | -4.145156256 |
| Cu3 | 7.621162352 | -5.874742317 | -4.145156256 |
| Cu3 | 2.532393618 | 2.939263679 | -4.145156256 |
| Cu3 | 12.709931087 | 2.939263679 | -4.145156256 |
| Cu3 | -2.556375116 | -5.874742317 | -4.145156256 |
| Cu3 | -2.556375116 | 11.753269675 | -4.145156256 |
| Cu3 | -10.178419075 | -5.86169978 | -4.1443887 |
| Cu3 | 10.176655862 | -5.86169978 | -4.1443887 |
| Cu3 | -0.000881606 | 11.766312212 | -4.1443887 |
| Cu3 | 5.087887128 | 2.952306216 | -4.1443887 |
| Cu3 | -0.000881606 | -5.86169978 | -4.1443887 |
| Cu3 | -5.089650341 | 2.952306216 | -4.1443887 |
| Cu3 | -3.81667034 | 5.159751119 | -4.139718228 |
| Cu3 | 1.272098394 | -3.654254877 | -4.139718228 |
| Cu3 | 6.360867128 | 5.159751119 | -4.139718228 |
| Cu3 | -8.905439075 | -3.654254877 | -4.139718228 |
| Cu3 | 11.449635863 | -3.654254877 | -4.139718228 |
| Cu3 | 1.264408422 | -8.068701867 | -4.137090168 |
| Cu3 | -3.824360312 | 0.745304129 | -4.137090168 |
| Cu3 | 6.353177157 | 0.745304129 | -4.137090168 |
| Cu3 | 1.264408422 | 9.559310125 | -4.137090168 |

| | | | |
|---|---|---|---|
| Cu3 | -8.913129046 | -8.068701867 | -4.137090168 |
| Cu3 | -3.818645867 | -3.661912755 | -4.137024001 |
| Cu3 | 11.447660336 | 5.152093241 | -4.137024001 |
| Cu3 | 6.358891602 | -3.661912755 | -4.137024001 |
| Cu3 | 1.270122867 | 5.152093241 | -4.137024001 |
| Cu3 | 7.647698788 | 2.944177605 | -4.136132377 |
| Cu3 | 2.558930053 | 11.758183601 | -4.136132377 |
| Cu3 | -7.618607415 | -5.869828391 | -4.136132377 |
| Cu3 | 2.558930053 | -5.869828391 | -4.136132377 |
| Cu3 | -2.529838681 | 2.944177605 | -4.136132377 |
| Cu3 | -2.546640902 | -1.460364965 | -4.133705157 |
| Cu3 | 2.542127832 | 7.353641031 | -4.133705157 |
| Cu3 | 7.630896567 | -1.460364965 | -4.133705157 |
| Cu3 | 5.088334492 | -1.45920313 | -4.133650707 |
| Cu3 | -5.089202977 | -1.45920313 | -4.133650707 |
| Cu3 | -0.000434242 | 7.354802866 | -4.133650707 |
| Cu3 | 10.177103226 | 7.354802866 | -4.133650707 |
| Cu3 | 8.907434329 | 5.158986116 | -4.131290097 |
| Cu3 | -6.358871874 | -3.65501988 | -4.131290097 |
| Cu3 | 3.818665595 | -3.65501988 | -4.131290097 |
| Cu3 | -1.270103139 | 5.158986116 | -4.131290097 |
| Cu3 | -1.28343694 | 9.548081623 | -4.131198527 |
| Cu3 | 3.805331794 | 0.734075627 | -4.131198527 |
| Cu3 | 8.894100528 | -8.079930369 | -4.131198527 |
| Cu3 | -6.372205675 | 0.734075627 | -4.131198527 |
| Cu3 | 13.982869263 | 0.734075627 | -4.131198527 |
| Cu3 | -1.28343694 | -8.079930369 | -4.131198527 |
| Cu3 | 8.894100528 | 9.548081623 | -4.131198527 |
| Cu3 | 2.546550176 | -1.462426328 | -4.129926585 |
| Cu3 | -7.630987293 | -1.462426328 | -4.129926585 |
| Cu3 | 7.63531891 | 7.351579668 | -4.129926585 |
| Cu3 | 12.724087645 | -1.462426328 | -4.129926585 |
| Cu3 | -2.542218558 | 7.351579668 | -4.129926585 |
| Cu3 | -1.259163654 | 0.740735582 | -4.124274442 |
| Cu3 | 3.82960508 | 9.554741578 | -4.124274442 |
| Cu3 | -6.347932388 | -8.073270414 | -4.124274442 |
| Cu3 | 8.918373815 | 0.740735582 | -4.124274442 |
| Cu3 | 3.82960508 | -8.073270414 | -4.124274442 |
| Cu3 | 6.367682154 | 9.544238761 | -4.123862364 |
| Cu3 | -3.809855314 | -8.083773231 | -4.123862364 |
| Cu3 | 6.367682154 | -8.083773231 | -4.123862364 |
| Cu3 | -8.898624049 | 0.730232765 | -4.123862364 |
| Cu3 | -3.809855314 | 9.544238761 | -4.123862364 |
| Cu3 | 11.456450889 | 0.730232765 | -4.123862364 |
| Cu3 | 1.27891342 | 0.730232765 | -4.123862364 |
| Cu3 | -5.087568981 | 7.359166279 | -4.122169694 |
| Cu3 | 10.178737222 | -1.454839717 | -4.122169694 |
| Cu3 | 0.001199753 | -1.454839717 | -4.122169694 |
| Cu3 | -10.176337716 | -1.454839717 | -4.122169694 |
| Cu3 | 5.089968487 | 7.359166279 | -4.122169694 |
| Cu1 | -5.097239566 | -4.422827522 | -2.127306969 |
| Cu1 | 5.080297902 | -4.422827522 | -2.127306969 |
| Cu1 | -0.008470832 | 4.391178474 | -2.127306969 |
| Cu3 | 10.169066637 | 4.391178474 | -2.127306969 |
| Cu1 | 2.552454509 | 4.397359892 | -2.125441688 |
| Cu3 | -7.62508296 | 4.397359892 | -2.125441688 |
| Cu1 | 7.641223243 | -4.416646104 | -2.125441688 |
| Cu1 | -2.536314225 | -4.416646104 | -2.125441688 |
| Cu1 | -1.271305599 | -6.610618123 | -2.125129274 |
| Cu3 | -1.271305599 | 11.017393869 | -2.125129274 |
| Cu3 | 8.906231869 | -6.610618123 | -2.125129274 |

| | | | |
|---|---|---|---|
| Cu1 | -6.360074334 | 2.203387873 | -2.125129274 |
| Cu1 | 3.817463135 | 2.203387873 | -2.125129274 |
| Cu3 | -8.896774804 | -6.604444515 | -2.118537838 |
| Cu1 | 1.280762664 | -6.604444515 | -2.118537838 |
| Cu1 | -3.80800607 | 2.209561481 | -2.118537838 |
| Cu3 | 1.280762664 | 11.023567477 | -2.118537838 |
| Cu1 | 6.369531399 | 2.209561481 | -2.118537838 |
| Cu1 | -2.548283806 | 6.6741e-05 | -2.108238099 |
| Cu1 | 2.540484928 | 8.814072737 | -2.108238099 |
| Cu3 | -7.63705254 | -8.813939255 | -2.108238099 |
| Cu1 | 7.629253663 | 6.6741e-05 | -2.108238099 |
| Cu3 | 2.540484928 | -8.813939255 | -2.108238099 |
| Cu1 | -1.282055814 | -2.210516891 | -2.106182692 |
| Cu1 | 3.80671292 | 6.603489105 | -2.106182692 |
| Cu1 | 8.895481655 | -2.210516891 | -2.106182692 |
| Cu3 | -6.370824548 | 6.603489105 | -2.106182692 |
| Cu3 | -11.459593283 | -2.210516891 | -2.106182692 |
| Cu1 | -7.641524147 | -4.409895376 | -2.102599789 |
| Cu1 | 7.624782056 | 4.40411062 | -2.102599789 |
| Cu1 | -2.552755413 | 4.40411062 | -2.102599789 |
| Cu1 | 2.536013321 | -4.409895376 | -2.102599789 |
| Cu1 | 1.257722889 | 2.180049922 | -2.098062593 |
| Cu3 | 6.346491623 | 10.994055918 | -2.098062593 |
| Cu3 | -3.831045845 | 10.994055918 | -2.098062593 |
| Cu1 | -3.831045845 | -6.633956074 | -2.098062593 |
| Cu3 | -8.91981458 | 2.180049922 | -2.098062593 |
| Cu1 | 6.346491623 | -6.633956074 | -2.098062593 |
| Cu3 | 11.435260358 | 2.180049922 | -2.098062593 |
| Cu3 | -10.173899419 | -4.417969954 | -2.093715761 |
| Cu3 | 10.181175518 | -4.417969954 | -2.093715761 |
| Cu1 | 5.092406784 | 4.396036042 | -2.093715761 |
| Cu1 | 0.00363805 | -4.417969954 | -2.093715761 |
| Cu1 | -5.085130685 | 4.396036042 | -2.093715761 |
| Cu1 | 1.271417944 | 6.601761053 | -2.091688337 |
| Cu1 | 6.360186679 | -2.212244943 | -2.091688337 |
| Cu1 | -3.81735079 | -2.212244943 | -2.091688337 |
| Cu1 | -5.092091278 | -0.011106636 | -2.089175844 |
| Cu1 | -0.003322543 | 8.80289936 | -2.089175844 |
| Cu3 | -0.003322543 | -8.825112632 | -2.089175844 |
| Cu1 | 5.085446191 | -0.011106636 | -2.089175844 |
| Cu1 | 6.367311664 | 6.610408812 | -2.07949831 |
| Cu1 | -8.898994539 | -2.203597184 | -2.07949831 |
| Cu1 | 1.27854293 | -2.203597184 | -2.07949831 |
| Cu3 | 11.456080399 | -2.203597184 | -2.07949831 |
| Cu1 | -3.810225804 | 6.610408812 | -2.07949831 |
| Cu3 | 3.825159803 | 11.002506538 | -2.076271089 |
| Cu1 | -1.263608931 | 2.188500542 | -2.076271089 |
| Cu1 | 8.913928538 | 2.188500542 | -2.076271089 |
| Cu1 | -6.352377665 | -6.625505454 | -2.076271089 |
| Cu1 | 3.825159803 | -6.625505454 | -2.076271089 |
| Cu1 | -6.352724196 | -2.201446506 | -2.074529435 |
| Cu1 | -1.263955461 | 6.61255949 | -2.074529435 |
| Cu1 | 3.824813273 | -2.201446506 | -2.074529435 |
| Cu3 | 8.913582007 | 6.61255949 | -2.074529435 |
| Cu3 | 7.637025097 | -8.84055614 | -2.046402999 |
| Cu3 | 7.637025097 | 8.787455852 | -2.046402999 |
| Cu1 | 2.548256363 | -0.026550144 | -2.046402999 |
| Cu3 | 12.725793832 | -0.026550144 | -2.046402999 |
| Cu3 | -2.540512371 | -8.84055614 | -2.046402999 |
| Cu1 | -7.629281106 | -0.026550144 | -2.046402999 |
| Cu1 | -2.540512371 | 8.787455852 | -2.046402999 |

| | | | |
|---|---|---|---|
| Cu3 | -5.082670999 | -8.821373738 | -2.038264892 |
| Cu1 | 10.183635204 | -0.007367742 | -2.038264892 |
| Cu3 | 5.094866469 | -8.821373738 | -2.038264892 |
| Cu1 | 0.006097735 | -0.007367742 | -2.038264892 |
| Cu3 | -10.171439734 | -0.007367742 | -2.038264892 |
| Cu3 | -5.082670999 | 8.806638254 | -2.038264892 |
| Cu1 | 5.094866469 | 8.806638254 | -2.038264892 |
| Cu1 | -3.810118199 | -5.125217421 | -0.10995456 |
| Cu1 | 6.367419269 | -5.125217421 | -0.10995456 |
| Cu2 | 1.278650535 | 3.688788575 | -0.10995456 |
| Cu3 | 0.005403875 | -7.324704491 | -0.102755428 |
| Cu2 | 5.094172609 | 1.489301505 | -0.102755428 |
| Cu1 | -5.08336486 | 1.489301505 | -0.102755428 |
| Cu3 | 0.005403875 | 10.303307501 | -0.102755428 |
| Cu3 | -5.107822877 | 5.849685448 | -0.092330587 |
| Cu2 | -0.019054143 | -2.964320548 | -0.092330587 |
| Cu1 | 5.069714591 | 5.849685448 | -0.092330587 |
| Cu3 | -10.196591612 | -2.964320548 | -0.092330587 |
| Cu3 | 10.158483326 | -2.964320548 | -0.092330587 |
| Cu3 | -7.611201805 | 1.503168302 | -0.089355359 |
| Cu3 | 7.655104398 | -7.310837694 | -0.089355359 |
| Cu3 | -2.52243307 | -7.310837694 | -0.089355359 |
| Cu3 | -2.52243307 | 10.317174298 | -0.089355359 |
| Cu2 | 2.566335664 | 1.503168302 | -0.089355359 |
| Cu1 | 7.654417705 | 5.835236828 | -0.060821865 |
| Cu2 | 2.565648971 | -2.978769168 | -0.060821865 |
| Cu1 | -7.611888498 | -2.978769168 | -0.060821865 |
| Cu1 | -2.523119763 | 5.835236828 | -0.060821865 |
| Cu2 | -1.300067263 | 3.686860258 | -0.053558403 |
| Cu1 | 8.877470206 | 3.686860258 | -0.053558403 |
| Cu1 | 3.788701471 | -5.127145738 | -0.053558403 |
| Cu1 | -6.388835997 | -5.127145738 | -0.053558403 |
| Cu1 | 3.78042585 | 8.058394432 | -0.051373324 |
| Cu1 | 8.869194585 | -0.755611564 | -0.051373324 |
| Cu2 | -1.308342884 | -0.755611564 | -0.051373324 |
| Cu2 | 6.376993287 | -0.739559765 | -0.042970929 |
| Cu1 | 1.288224552 | 8.074446231 | -0.042970929 |
| Cu2 | -3.800544182 | -0.739559765 | -0.042970929 |
| Cu1 | 7.610463014 | 1.462661473 | -0.042834878 |
| Cu3 | -7.655843189 | -7.351344523 | -0.042834878 |
| Cu3 | 2.521694279 | 10.276667469 | -0.042834878 |
| Cu3 | 2.521694279 | -7.351344523 | -0.042834878 |
| Cu2 | -2.567074455 | 1.462661473 | -0.042834878 |
| Cu2 | 5.106623475 | -2.963632667 | -0.033447027 |
| Cu2 | 0.017854741 | 5.850373329 | -0.033447027 |
| Cu1 | -5.070913994 | -2.963632667 | -0.033447027 |
| Cu3 | 8.909756736 | -5.143886962 | -0.015295562 |
| Cu2 | 3.820988002 | 3.670119034 | -0.015295562 |
| Cu1 | -1.267780732 | -5.143886962 | -0.015295562 |
| Cu3 | -6.356549467 | 3.670119034 | -0.015295562 |
| Cu2 | 2.537784588 | 5.8673689 | -0.012553735 |
| Cu2 | -2.550984146 | -2.946637096 | -0.012553735 |
| Cu1 | 7.626553323 | -2.946637096 | -0.012553735 |
| Cu1 | 1.273256259 | -5.152120687 | -0.007057577 |
| Cu3 | -8.904281209 | -5.152120687 | -0.007057577 |
| Cu1 | -3.815512475 | 3.661885309 | -0.007057577 |
| Cu1 | 6.362024994 | 3.661885309 | -0.007057577 |
| Cu3 | 11.444937864 | -0.770137248 | 0.021340658 |
| Cu3 | -3.821368339 | 8.043868748 | 0.021340658 |
| Cu2 | 1.267400395 | -0.770137248 | 0.021340658 |
| Cu1 | 6.356169129 | 8.043868748 | 0.021340658 |

| | | | |
|---|---|---|---|
| Cu3 | -8.910137074 | -0.770137248 | 0.021340658 |
| Cu2 | 3.84531852 | -0.736506215 | 0.021716688 |
| Cu1 | -1.243450214 | 8.077499781 | 0.021716688 |
| Cu1 | -6.332218949 | -0.736506215 | 0.021716688 |
| Cu3 | 5.080666563 | -7.3178853 | 0.024227366 |
| Cu1 | 10.169435298 | 1.496120696 | 0.024227366 |
| Cu3 | -5.096870905 | -7.3178853 | 0.024227366 |
| Cu2 | -0.008102171 | 1.496120696 | 0.024227366 |
| Cu3 | 5.080666563 | 10.310126692 | 0.024227366 |
| O | 1.272913651 | -0.709676705 | 2.193591779 |
| H | 2.054445672 | 3.943784007 | 2.21175184 |
| H | 6.14655201 | 1.500709033 | 2.21907952 |
| O1 | 0.067247715 | 1.656346268 | 2.238723376 |
| H | -0.91847428 | -2.951492146 | 2.264228538 |
| O | 3.968481841 | -0.643390944 | 2.302902383 |
| H | 0.85437544 | 0.187062817 | 2.393362308 |
| H | 2.249674352 | -0.661498361 | 2.423123337 |
| H | 4.520599128 | -1.433553363 | 2.49944461 |
| H | -0.872765089 | 1.751487351 | 2.510863932 |
| H | 4.873987228 | 2.303526432 | 2.514979609 |
| H | 0.570440617 | 2.533981535 | 2.517096734 |
| H | 4.526336606 | 0.177658185 | 2.549387373 |
| H | 0.313248026 | -2.090160687 | 2.719032089 |
| O | 5.393261367 | 1.538980102 | 2.870463157 |
| H | 0.774941788 | 4.591417825 | 2.906380795 |
| O | 1.370231108 | 3.761999411 | 2.906615836 |
| O | -0.213096839 | -2.908080758 | 2.958228458 |

## $Be_{167}$

167
Atoms

| | | | |
|---|---|---|---|
| Be1 | 0 | -1e-05 | 5e-05 |
| Be2 | 0 | 1.30688 | -1.78005 |
| Be2 | 1.1318 | -0.653455 | -1.78005 |
| Be2 | -1.1318 | -0.653455 | -1.78005 |
| Be2 | 0 | 1.30688 | 1.78015 |
| Be2 | -1.1318 | -0.653455 | 1.78015 |
| Be2 | 1.1318 | -0.653455 | 1.78015 |
| Be2 | -1.1318 | 1.960325 | 5e-05 |
| Be2 | 1.1318 | 1.960325 | 5e-05 |
| Be2 | -2.2636 | -1e-05 | 5e-05 |
| Be2 | 2.2636 | -1e-05 | 5e-05 |
| Be2 | -1.1318 | -1.960345 | 5e-05 |
| Be2 | 1.1318 | -1.960345 | 5e-05 |
| Be | 2.2636 | 1.30688 | -1.78005 |
| Be | -2.2636 | 1.30688 | -1.78005 |
| Be | 0 | -2.61379 | -1.78005 |
| Be | -2.2636 | 1.30688 | 1.78015 |
| Be | 2.2636 | 1.30688 | 1.78015 |
| Be | 0 | -2.61379 | 1.78015 |
| Be | 0 | -1e-05 | -3.56015 |
| Be | 0 | -1e-05 | 3.56025 |
| Be | -1.1318 | 3.267215 | -1.78005 |
| Be | 1.1318 | 3.267215 | -1.78005 |
| Be | 3.3954 | -0.653455 | -1.78005 |
| Be | -3.3954 | -0.653455 | -1.78005 |
| Be | -2.2636 | -2.61379 | -1.78005 |
| Be | 2.2636 | -2.61379 | -1.78005 |
| Be | -1.1318 | 3.267215 | 1.78015 |
| Be | 1.1318 | 3.267215 | 1.78015 |

| | | | |
|---|---|---|---|
| Be | 3.3954 | -0.653455 | 1.78015 |
| Be | -3.3954 | -0.653455 | 1.78015 |
| Be | 2.2636 | -2.61379 | 1.78015 |
| Be | -2.2636 | -2.61379 | 1.78015 |
| Be | 0 | 3.92066 | 5e-05 |
| Be | 3.3954 | 1.960325 | 5e-05 |
| Be | -3.3954 | 1.960325 | 5e-05 |
| Be | 3.3954 | -1.960345 | 5e-05 |
| Be | -3.3954 | -1.960345 | 5e-05 |
| Be | 0 | -3.92068 | 5e-05 |
| Be | -1.1318 | 1.960325 | -3.56015 |
| Be | 1.1318 | 1.960325 | -3.56015 |
| Be | 2.2636 | -1e-05 | -3.56015 |
| Be | -2.2636 | -1e-05 | -3.56015 |
| Be | 1.1318 | -1.960345 | -3.56015 |
| Be | -1.1318 | -1.960345 | -3.56015 |
| Be | 1.1318 | 1.960325 | 3.56025 |
| Be | -1.1318 | 1.960325 | 3.56025 |
| Be | -2.2636 | -1e-05 | 3.56025 |
| Be | 2.2636 | -1e-05 | 3.56025 |
| Be | 1.1318 | -1.960345 | 3.56025 |
| Be | -1.1318 | -1.960345 | 3.56025 |
| Be | 2.2636 | 3.92066 | 5e-05 |
| Be | -2.2636 | 3.92066 | 5e-05 |
| Be | -4.5272 | -1e-05 | 5e-05 |
| Be | 4.5272 | -1e-05 | 5e-05 |
| Be | -2.2636 | -3.92068 | 5e-05 |
| Be | 2.2636 | -3.92068 | 5e-05 |
| Be | -3.3954 | 3.267215 | -1.78005 |
| Be | 3.3954 | 3.267215 | -1.78005 |
| Be | 4.5272 | 1.30688 | -1.78005 |
| Be | -4.5272 | 1.30688 | -1.78005 |
| Be | -1.1318 | -4.574125 | -1.78005 |
| Be | 1.1318 | -4.574125 | -1.78005 |
| Be | 3.3954 | 3.267215 | 1.78015 |
| Be | -3.3954 | 3.267215 | 1.78015 |
| Be | 4.5272 | 1.30688 | 1.78015 |
| Be | -4.5272 | 1.30688 | 1.78015 |
| Be | -1.1318 | -4.574125 | 1.78015 |
| Be | 1.1318 | -4.574125 | 1.78015 |
| Be | 0 | 3.92066 | -3.56015 |
| Be | 3.3954 | 1.960325 | -3.56015 |
| Be | -3.3954 | 1.960325 | -3.56015 |
| Be | 3.3954 | -1.960345 | -3.56015 |
| Be | -3.3954 | -1.960345 | -3.56015 |
| Be | 0 | -3.92068 | -3.56015 |
| Be | 0 | 3.92066 | 3.56025 |
| Be | 3.3954 | 1.960325 | 3.56025 |
| Be | -3.3954 | 1.960325 | 3.56025 |
| Be | -3.3954 | -1.960345 | 3.56025 |
| Be | 3.3954 | -1.960345 | 3.56025 |
| Be | 0 | -3.92068 | 3.56025 |
| Be | 0 | 1.30688 | -5.34025 |
| Be | 1.1318 | -0.653455 | -5.34025 |
| Be | -1.1318 | -0.653455 | -5.34025 |
| Be | 0 | 5.227551 | -1.78005 |
| Be | 4.5272 | -2.61379 | -1.78005 |
| Be | -4.5272 | -2.61379 | -1.78005 |
| Be | 0 | 5.227551 | 1.78015 |
| Be | -4.5272 | -2.61379 | 1.78015 |
| Be | 4.5272 | -2.61379 | 1.78015 |

| | | | |
|---|---|---|---|
| Be | -2.2636 | 3.92066 | -3.56015 |
| Be | 2.2636 | 3.92066 | -3.56015 |
| Be | 4.5272 | -1e-05 | -3.56015 |
| Be | -4.5272 | -1e-05 | -3.56015 |
| Be | -2.2636 | -3.92068 | -3.56015 |
| Be | 2.2636 | -3.92068 | -3.56015 |
| Be | -2.2636 | 3.92066 | 3.56025 |
| Be | 2.2636 | 3.92066 | 3.56025 |
| Be | 4.5272 | -1e-05 | 3.56025 |
| Be | -4.5272 | -1e-05 | 3.56025 |
| Be | 2.2636 | -3.92068 | 3.56025 |
| Be | -2.2636 | -3.92068 | 3.56025 |
| Be | 2.2636 | 1.30688 | -5.34025 |
| Be | -2.2636 | 1.30688 | -5.34025 |
| Be | 0 | -2.61379 | -5.34025 |
| Be | -2.2636 | 5.227551 | -1.78005 |
| Be | 2.2636 | 5.227551 | -1.78005 |
| Be | -5.659 | -0.653455 | -1.78005 |
| Be | 5.659 | -0.653455 | -1.78005 |
| Be | -3.3954 | -4.574125 | -1.78005 |
| Be | 3.3954 | -4.574125 | -1.78005 |
| Be | 2.2636 | 5.227551 | 1.78015 |
| Be | -2.2636 | 5.227551 | 1.78015 |
| Be | 5.659 | -0.653455 | 1.78015 |
| Be | -5.659 | -0.653455 | 1.78015 |
| Be | 3.3954 | -4.574125 | 1.78015 |
| Be | -3.3954 | -4.574125 | 1.78015 |
| Be | -1.1318 | 5.880995 | 5e-05 |
| Be | 1.1318 | 5.880995 | 5e-05 |
| Be | 4.5272 | 3.92066 | 5e-05 |
| Be | -4.5272 | 3.92066 | 5e-05 |
| Be | -5.659 | 1.960325 | 5e-05 |
| Be | 5.659 | 1.960325 | 5e-05 |
| Be | -5.659 | -1.960345 | 5e-05 |
| Be | 5.659 | -1.960345 | 5e-05 |
| Be | 4.5272 | -3.92068 | 5e-05 |
| Be | -4.5272 | -3.92068 | 5e-05 |
| Be | 1.1318 | -5.881015 | 5e-05 |
| Be | -1.1318 | -5.881015 | 5e-05 |
| Be | -1.1318 | 3.267215 | -5.34025 |
| Be | 1.1318 | 3.267215 | -5.34025 |
| Be | -3.3954 | -0.653455 | -5.34025 |
| Be | 3.3954 | -0.653455 | -5.34025 |
| Be | 2.2636 | -2.61379 | -5.34025 |
| Be | -2.2636 | -2.61379 | -5.34025 |
| Be | -5.659 | 3.267215 | -1.78005 |
| Be | 5.659 | 3.267215 | -1.78005 |
| Be | 0 | -6.53446 | -1.78005 |
| Be | 0 | -6.53446 | 1.78015 |
| Be | 3.3954 | 5.880995 | 5e-05 |
| Be | -3.3954 | 5.880995 | 5e-05 |
| Be | -6.7908 | -1e-05 | 5e-05 |
| Be | 6.7908 | -1e-05 | 5e-05 |
| Be | 3.3954 | -5.881015 | 5e-05 |
| Be | -3.3954 | -5.881015 | 5e-05 |
| Be | 4.5272 | 3.92066 | -3.56015 |
| Be | -4.5272 | 3.92066 | -3.56015 |
| Be | 5.659 | 1.960325 | -3.56015 |
| Be | -5.659 | 1.960325 | -3.56015 |
| Be | 1.1318 | -5.881015 | -3.56015 |
| Be | -1.1318 | -5.881015 | -3.56015 |

Be 1.1318 -5.881015 3.56025
Be -1.1318 -5.881015 3.56025
Be 3.3954 3.267215 -5.34025
Be -3.3954 3.267215 -5.34025
Be 4.5272 1.30688 -5.34025
Be -4.5272 1.30688 -5.34025
Be -1.1318 -4.574125 -5.34025
Be 1.1318 -4.574125 -5.34025
Be -4.5272 5.227551 -1.78005
Be 4.5272 5.227551 -1.78005
Be 6.7908 1.30688 -1.78005
Be -6.7908 1.30688 -1.78005
Be 2.2636 -6.53446 -1.78005
Be -2.2636 -6.53446 -1.78005
Be 2.2636 -6.53446 1.78015
Be -2.2636 -6.53446 1.78015

## $Mg_{167}$

167
Atoms
Mg1 0 1.841805 1.273525
Mg2 -1.59505 0.920903 3.820575
Mg2 1.59505 0.920903 3.820575
Mg2 -1.59505 0.920903 -1.273525
Mg2 1.59505 0.920903 -1.273525
Mg2 0 3.68361 -1.273525
Mg2 0 3.68361 3.820575
Mg2 -3.1901 1.841805 1.273525
Mg2 3.1901 1.841805 1.273525
Mg2 1.59505 4.604513 1.273525
Mg2 -1.59505 4.604513 1.273525
Mg2 1.59505 -0.920903 1.273525
Mg2 -1.59505 -0.920903 1.273525
Mg 0 -1.841805 3.820575
Mg 0 -1.841805 -1.273525
Mg 3.1901 3.68361 3.820575
Mg -3.1901 3.68361 3.820575
Mg -3.1901 3.68361 -1.273525
Mg 3.1901 3.68361 -1.273525
Mg 0 1.841805 6.367625
Mg 0 1.841805 -3.820575
Mg 3.1901 -1.841805 -1.273525
Mg 3.1901 -1.841805 3.820575
Mg -3.1901 -1.841805 3.820575
Mg -3.1901 -1.841805 -1.273525
Mg -4.78515 0.920903 -1.273525
Mg 4.78515 0.920903 -1.273525
Mg 4.78515 0.920903 3.820575
Mg -4.78515 0.920903 3.820575
Mg 1.59505 6.446318 3.820575
Mg -1.59505 6.446318 -1.273525
Mg -1.59505 6.446318 3.820575
Mg 1.59505 6.446318 -1.273525
Mg 0 7.36722 1.273525
Mg 0 -3.68361 1.273525
Mg 4.78515 -0.920903 1.273525
Mg 4.78515 4.604513 1.273525
Mg -4.78515 4.604513 1.273525
Mg -4.78515 -0.920903 1.273525
Mg -3.1901 1.841805 -3.820575

| | | | |
|---|---|---|---|
| Mg | 3.1901 | 1.841805 | 6.367625 |
| Mg | -3.1901 | 1.841805 | 6.367625 |
| Mg | 3.1901 | 1.841805 | -3.820575 |
| Mg | -1.59505 | 4.604513 | -3.820575 |
| Mg | 1.59505 | 4.604513 | -3.820575 |
| Mg | -1.59505 | 4.604513 | 6.367625 |
| Mg | 1.59505 | 4.604513 | 6.367625 |
| Mg | 1.59505 | -0.920903 | -3.820575 |
| Mg | -1.59505 | -0.920903 | -3.820575 |
| Mg | -1.59505 | -0.920903 | 6.367625 |
| Mg | 1.59505 | -0.920903 | 6.367625 |
| Mg | 3.1901 | 7.36722 | 1.273525 |
| Mg | -3.1901 | 7.36722 | 1.273525 |
| Mg | -3.1901 | -3.68361 | 1.273525 |
| Mg | 3.1901 | -3.68361 | 1.273525 |
| Mg | 6.3802 | 1.841805 | 1.273525 |
| Mg | -6.3802 | 1.841805 | 1.273525 |
| Mg | -6.3802 | 3.68361 | 3.820575 |
| Mg | -6.3802 | 3.68361 | -1.273525 |
| Mg | 6.3802 | 3.68361 | -1.273525 |
| Mg | 6.3802 | 3.68361 | 3.820575 |
| Mg | 1.59505 | -4.604513 | 3.820575 |
| Mg | -1.59505 | -4.604513 | 3.820575 |
| Mg | -1.59505 | -4.604513 | -1.273525 |
| Mg | 1.59505 | -4.604513 | -1.273525 |
| Mg | -4.78515 | 6.446318 | -1.273525 |
| Mg | 4.78515 | 6.446318 | 3.820575 |
| Mg | -4.78515 | 6.446318 | 3.820575 |
| Mg | 4.78515 | 6.446318 | -1.273525 |
| Mg | 0 | -3.68361 | 6.367625 |
| Mg | 0 | -3.68361 | -3.820575 |
| Mg | 0 | 7.36722 | -3.820575 |
| Mg | 0 | 7.36722 | 6.367625 |
| Mg | 4.78515 | -0.920903 | 6.367625 |
| Mg | -4.78515 | 4.604513 | 6.367625 |
| Mg | 4.78515 | 4.604513 | 6.367625 |
| Mg | 4.78515 | 4.604513 | -3.820575 |
| Mg | -4.78515 | 4.604513 | -3.820575 |
| Mg | -4.78515 | -0.920903 | -3.820575 |
| Mg | -4.78515 | -0.920903 | 6.367625 |
| Mg | 4.78515 | -0.920903 | -3.820575 |
| Mg | 0 | 9.209025 | -1.273525 |
| Mg | 0 | 9.209025 | 3.820575 |
| Mg | -6.3802 | -1.841805 | 3.820575 |
| Mg | 6.3802 | -1.841805 | 3.820575 |
| Mg | -6.3802 | -1.841805 | -1.273525 |
| Mg | 6.3802 | -1.841805 | -1.273525 |
| Mg | 1.59505 | 0.920903 | -6.367625 |
| Mg | -1.59505 | 0.920903 | -6.367625 |
| Mg | 0 | 3.68361 | -6.367625 |
| Mg | 3.1901 | 7.36722 | -3.820575 |
| Mg | -3.1901 | -3.68361 | 6.367625 |
| Mg | -3.1901 | -3.68361 | -3.820575 |
| Mg | 3.1901 | -3.68361 | -3.820575 |
| Mg | -3.1901 | 7.36722 | -3.820575 |
| Mg | 3.1901 | 7.36722 | 6.367625 |
| Mg | 3.1901 | -3.68361 | 6.367625 |
| Mg | -3.1901 | 7.36722 | 6.367625 |
| Mg | 6.3802 | 1.841805 | 6.367625 |
| Mg | -6.3802 | 1.841805 | -3.820575 |
| Mg | 6.3802 | 1.841805 | -3.820575 |

| | | | |
|---|---|---|---|
| Mg | -6.3802 | 1.841805 | 6.367625 |
| Mg | -3.1901 | 9.209025 | -1.273525 |
| Mg | 3.1901 | 9.209025 | -1.273525 |
| Mg | 3.1901 | 9.209025 | 3.820575 |
| Mg | -3.1901 | 9.209025 | 3.820575 |
| Mg | 7.97525 | 0.920903 | -1.273525 |
| Mg | -7.97525 | 0.920903 | 3.820575 |
| Mg | 7.97525 | 0.920903 | 3.820575 |
| Mg | -7.97525 | 0.920903 | -1.273525 |
| Mg | -4.78515 | -4.604513 | -1.273525 |
| Mg | 4.78515 | -4.604513 | -1.273525 |
| Mg | -4.78515 | -4.604513 | 3.820575 |
| Mg | 4.78515 | -4.604513 | 3.820575 |
| Mg | -6.3802 | -3.68361 | 1.273525 |
| Mg | 6.3802 | -3.68361 | 1.273525 |
| Mg | -6.3802 | 7.36722 | 1.273525 |
| Mg | 6.3802 | 7.36722 | 1.273525 |
| Mg | -1.59505 | 10.129928 | 1.273525 |
| Mg | 1.59505 | -6.446318 | 1.273525 |
| Mg | 1.59505 | 10.129928 | 1.273525 |
| Mg | -1.59505 | -6.446318 | 1.273525 |
| Mg | -7.97525 | -0.920903 | 1.273525 |
| Mg | 7.97525 | -0.920903 | 1.273525 |
| Mg | -7.97525 | 4.604513 | 1.273525 |
| Mg | 7.97525 | 4.604513 | 1.273525 |
| Mg | 0 | -1.841805 | -6.367625 |
| Mg | -3.1901 | 3.68361 | -6.367625 |
| Mg | 3.1901 | 3.68361 | -6.367625 |
| Mg | -3.1901 | -1.841805 | -6.367625 |
| Mg | 3.1901 | -1.841805 | -6.367625 |
| Mg | -4.78515 | 0.920903 | -6.367625 |
| Mg | 4.78515 | 0.920903 | -6.367625 |
| Mg | 1.59505 | 6.446318 | -6.367625 |
| Mg | -1.59505 | 6.446318 | -6.367625 |
| Mg | 0 | -7.36722 | -1.273525 |
| Mg | 0 | -7.36722 | 3.820575 |
| Mg | -7.97525 | 6.446318 | -1.273525 |
| Mg | 7.97525 | 6.446318 | -1.273525 |
| Mg | -9.5703 | 1.841805 | 1.273525 |
| Mg | 9.5703 | 1.841805 | 1.273525 |
| Mg | 4.78515 | -6.446318 | 1.273525 |
| Mg | -4.78515 | -6.446318 | 1.273525 |
| Mg | 4.78515 | 10.129928 | 1.273525 |
| Mg | -4.78515 | 10.129928 | 1.273525 |
| Mg | -6.3802 | 7.36722 | -3.820575 |
| Mg | 6.3802 | 7.36722 | -3.820575 |
| Mg | 1.59505 | -6.446318 | 6.367625 |
| Mg | -1.59505 | -6.446318 | 6.367625 |
| Mg | 1.59505 | -6.446318 | -3.820575 |
| Mg | -1.59505 | -6.446318 | -3.820575 |
| Mg | -7.97525 | 4.604513 | -3.820575 |
| Mg | 7.97525 | 4.604513 | -3.820575 |
| Mg | -3.1901 | -7.36722 | 3.820575 |
| Mg | -3.1901 | -7.36722 | -1.273525 |
| Mg | 3.1901 | -7.36722 | -1.273525 |
| Mg | 3.1901 | -7.36722 | 3.820575 |
| Mg | -6.3802 | 9.209025 | -1.273525 |
| Mg | 6.3802 | 9.209025 | -1.273525 |
| Mg | 9.5703 | 3.68361 | -1.273525 |
| Mg | -9.5703 | 3.68361 | -1.273525 |
| Mg | 6.3802 | 3.68361 | -6.367625 |

| | | | |
|---|---|---|---|
| Mg | -6.3802 | 3.68361 | -6.367625 |
| Mg | 1.59505 | -4.604513 | -6.367625 |
| Mg | -1.59505 | -4.604513 | -6.367625 |
| Mg | -4.78515 | 6.446318 | -6.367625 |
| Mg | 4.78515 | 6.446318 | -6.367625 |

## Basis sets used in the cluster calculations

All of these basis sets are variants of the default FHI-aims basis sets (Blum et al., Comput. Phys. Commun. 180, 2175 (2009)). Additional core functions have been added for use with the atoms whose core electron is removed. Given in FHI-aims format, together with a definition of other numerical parameters. For all of the non-metal atoms, the same basis sets were used as in the molecular calculations.

### Be1 – the central Be atom whose core electron is removed

```
  species        Be1
#     global species definitions
    nucleus             4.0
    mass                9.012182
#
    l_hartree           6
#
    cut_pot             4.0  2.0  1.0
    basis_dep_cutoff    1e-4
#
    radial_base         31 7.0
    radial_multiplier   2
    angular_grids       specified
      division   0.4283  110
      division   0.4792  194
      division   0.5061  302
      division   0.7227  434
#      division   0.8724  590
#      division   0.9555  770
#      division   2.9770  974
#      outer_grid   974
      outer_grid  434

#     valence basis states
    valence      2  s   1.999
    valence      2  p   0.001
#     ion occupancy
    ion_occ      2  s   1.

#  "First tier" - improvements: -677.26 meV to -34.75 meV
     ionic 2 p auto
     hydro 3 s 2.9
     hydro 3 d 3.5
#  "Second tier" - improvements: -16.34 meV to -1.26 meV
     hydro 3 p 3.1
     hydro 4 d 4.7
#     hydro 3 p 2.4
     hydro 4 f 7.6
     hydro 2 s 2.9
#  "Third tier" - improvements: -0.27 meV to -0.05 meV
#     hydro 2 p 8.2
#     hydro 5 g 10.8
#     hydro 4 f 7
#     hydro 3 s 2.3
#     hydro 4 d 3.8

# Additional basis functions for atoms with a core hole

    hydro 1 s 5.0
    hydro 1 s 7.0
```

```
    hydro 2 s 6.0
```

## Be2 – nearest neighbours of the atom whose core electron is removed

```
  species        Be2
#     global species definitions
    nucleus             4
    mass                9.012182
#
    l_hartree           6
#
    cut_pot             4.0  2.0  1.0
    basis_dep_cutoff    1e-4
#
    radial_base         31 7.0
    radial_multiplier   2
    angular_grids       specified
      division   0.4283  110
      division   0.4792  194
      division   0.5061  302
      division   0.7227  434
#      division   0.8724  590
#      division   0.9555  770
#      division   2.9770  974
#      outer_grid   974
      outer_grid  434

#     valence basis states
    valence      2  s   2.
#     ion occupancy
    ion_occ      2  s   1.

#  "First tier" - improvements: -677.26 meV to -34.75 meV
     ionic 2 p auto
     hydro 3 s 2.9
     hydro 3 d 3.5
#  "Second tier" - improvements: -16.34 meV to -1.26 meV
     hydro 3 p 3.1
     hydro 4 d 4.7
     hydro 3 p 2.4
#     hydro 4 f 7.6
#     hydro 2 s 2.9
#  "Third tier" - improvements: -0.27 meV to -0.05 meV
#     hydro 2 p 8.2
#     hydro 5 g 10.8
#     hydro 4 f 7
#     hydro 3 s 2.3
#     hydro 4 d 3.8
```

## Be – all other Be atoms

```
  species        Be
#     global species definitions
    nucleus             4
    mass                9.012182
#
    l_hartree           6
#
    cut_pot             4.0  2.0  1.0
    basis_dep_cutoff    1e-4
#
```

```
    radial_base         31 7.0
    radial_multiplier   2
    angular_grids       specified
      division   0.4283  110
      division   0.4792  194
      division   0.5061  302
      division   0.7227  434
#      division   0.8724  590
#      division   0.9555  770
#      division   2.9770  974
#      outer_grid   974
      outer_grid  434

#     valence basis states
    valence      2  s   2.
#     ion occupancy
    ion_occ      2  s   1.

#  "First tier" - improvements: -677.26 meV to -34.75 meV
     ionic 2 p auto
     hydro 3 s 2.9
     hydro 3 d 3.5
#  "Second tier" - improvements: -16.34 meV to -1.26 meV
#     hydro 3 p 3.1
#     hydro 4 d 4.7
#     hydro 3 p 2.4
#     hydro 4 f 7.6
#     hydro 2 s 2.9
#  "Third tier" - improvements: -0.27 meV to -0.05 meV
#     hydro 2 p 8.2
#     hydro 5 g 10.8
#     hydro 4 f 7
#     hydro 3 s 2.3
#     hydro 4 d 3.8
```

## Mg1 – the central Mg atom whose core electron is removed

```
  species        Mg1
#     global species definitions
    nucleus             12.
    mass                24.3050
#
    l_hartree           6
#
    cut_pot             5.5          2.0  1.0
    basis_dep_cutoff    1e-5
#
    radial_base         50 7.5
    radial_multiplier   2
    angular_grids       specified
      division   0.5421   50
      division   0.8500  110
      division   1.0736  194
      division   1.1879  302
      division   1.2806  434
      division   1.4147  590
#      division   1.4867  770
#      division   1.6422  974
#      division   2.6134 1202
#      outer_grid   974
      outer_grid  590
```

```
#     valence basis states
    valence      3  s   2.
    valence      3  p   0.
#     ion occupancy
    ion_occ      2  s   2.
    ion_occ      2  p   6.

#  "First tier" - improvements: -230.76 meV to -21.94 meV
     hydro 2 p 1.5
     ionic 3 d auto
     hydro 3 s 2.4
#  "Second tier" - improvements: -5.43 meV to -1.64 meV
     hydro 4 f 4.3
     hydro 2 p 3.4
     hydro 4 s 11.2
     hydro 3 d 6.2
#  "Third tier" - improvements: -0.92 meV to -0.22 meV
#     hydro 2 s 0.6
#     hydro 3 p 4.8
#     hydro 4 f 7.4
#     hydro 5 g 6.6
#     hydro 2 p 1.6
#     hydro 3 d 1.8
#  "Fourth tier" - improvements: -0.09 meV to -0.05 meV
#     hydro 4 p 0.45
#     hydro 5 g 10.4
#     hydro 2 s 12.4
#     hydro 4 d 1.7

# additional basis functions for atom with a core hole

     hydro 1 s 16.0
     hydro 1 s 14.0
     hydro 1 s 10.0
     hydro 2 s 14.5
     hydro 2 s 12.5
     hydro 2 p 11.5
     hydro 2 p 9.5
     hydro 3 d 8.0
     hydro 3 p 9.0
```

## Mg2 – nearest neighbours of the atom whose core electron is removed

```
  species        Mg2
#     global species definitions
    nucleus             12
    mass                24.3050
#
    l_hartree           6
#
    cut_pot             5.5          2.0  1.0
    basis_dep_cutoff    1e-5
#
    radial_base         50 7.5
    radial_multiplier   2
    angular_grids       specified
      division   0.5421   50
      division   0.8500  110
      division   1.0736  194
      division   1.1879  302
```

```
      division   1.2806  434
      division   1.4147  590
#      division   1.4867  770
#      division   1.6422  974
#      division   2.6134 1202
#      outer_grid   974
      outer_grid  590

#     valence basis states
    valence      3  s   2.
    valence      2  p   6.
#     ion occupancy
    ion_occ      2  s   2.
    ion_occ      2  p   6.

#  "First tier" - improvements: -230.76 meV to -21.94 meV
     hydro 2 p 1.5
     ionic 3 d auto
     hydro 3 s 2.4
#  "Second tier" - improvements: -5.43 meV to -1.64 meV
     hydro 4 f 4.3
     hydro 2 p 3.4
     hydro 4 s 11.2
     hydro 3 d 6.2
#  "Third tier" - improvements: -0.92 meV to -0.22 meV
#     hydro 2 s 0.6
#     hydro 3 p 4.8
#     hydro 4 f 7.4
#     hydro 5 g 6.6
#     hydro 2 p 1.6
#     hydro 3 d 1.8
#  "Fourth tier" - improvements: -0.09 meV to -0.05 meV
#     hydro 4 p 0.45
#     hydro 5 g 10.4
#     hydro 2 s 12.4
#     hydro 4 d 1.7
```

## Mg – all other Mg atoms

```
  species        Mg
#     global species definitions
    nucleus             12
    mass                24.3050
#
    l_hartree           6
#
    cut_pot             5.5          2.0  1.0
    basis_dep_cutoff    1e-5
#
    radial_base         50 7.5
    radial_multiplier   2
    angular_grids       specified
      division   0.5421   50
      division   0.8500  110
      division   1.0736  194
      division   1.1879  302
      division   1.2806  434
      division   1.4147  590
#      division   1.4867  770
#      division   1.6422  974
#      division   2.6134 1202
```

```
#      outer_grid   974
     outer_grid  590

#     valence basis states
    valence      3  s   2.
    valence      2  p   6.
#     ion occupancy
    ion_occ      2  s   2.
    ion_occ      2  p   6.

#  "First tier" - improvements: -230.76 meV to -21.94 meV
     hydro 2 p 1.5
     ionic 3 d auto
     hydro 3 s 2.4
#  "Second tier" - improvements: -5.43 meV to -1.64 meV
#     hydro 4 f 4.3
#     hydro 2 p 3.4
#     hydro 4 s 11.2
#     hydro 3 d 6.2
#  "Third tier" - improvements: -0.92 meV to -0.22 meV
#     hydro 2 s 0.6
#     hydro 3 p 4.8
#     hydro 4 f 7.4
#     hydro 5 g 6.6
#     hydro 2 p 1.6
#     hydro 3 d 1.8
#  "Fourth tier" - improvements: -0.09 meV to -0.05 meV
#     hydro 4 p 0.45
#     hydro 5 g 10.4
#     hydro 2 s 12.4
#     hydro 4 d 1.7
```

## Cu2 – top layer Cu atoms that are in the vicinity of the adsorbate

```
  species        Cu2
#
    nucleus      29
    mass         63.546
#
    l_hartree    6
#
    cut_pot      4.0  2.0  1.0
    basis_dep_cutoff    1e-4
#
    radial_base        53 7.0
    radial_multiplier  2
    angular_grids       specified
      division   0.3478   50
      division   0.6638  110
      division   0.9718  194
      division   1.1992  302
      division   1.5920  434
#      division   1.8557  590
#      division   2.0466  770
#      division   2.0877  974
#      division   2.4589 1202
      outer_grid   434

#     valence basis states
    valence      4  s   1.
    valence      3  p   6.
```

```
    valence      3  d  10.
#     ion occupancy
    ion_occ      4  s   0.
    ion_occ      3  p   6.
    ion_occ      3  d   9.

#  "First tier" - improvements: -211.42 meV to -9.17 meV
     ionic 4 p auto
     hydro 4 f 7.4
     hydro 3 s 2.6
     hydro 3 d 5
     hydro 5 g 10.4
#  "Second tier" - improvements: -2.49 meV to -1.08 meV
     hydro 4 p 5.8
     hydro 3 d 2.7
     hydro 6 h 15.2
     hydro 5 s 10.8
     hydro 4 f 16
#  "Third tier" - improvements: -0.50 meV to -0.21 meV
#     hydro 4 d 6
#     hydro 3 p 2.4
#     hydro 4 f 6.4
#     hydro 3 s 6.8
#     hydro 5 g 11.2
#  "Fourth tier" - improvements: -0.13 meV to -0.05 meV
#     hydro 4 p 7
#     hydro 4 s 4
#     hydro 6 h 14
#     hydro 4 d 8.6
#     hydro 5 f 15.2
```

## Cu1 – “intermediate” Cu atoms that are further from the adsorbate

```
  species        Cu1
#
    nucleus      29
    mass         63.546
#
    l_hartree    4
#
    cut_pot      3.5  1.5  1.0
    basis_dep_cutoff    1e-4
#
    radial_base        53 5.0
    radial_multiplier  1
    angular_grids       specified
      division   0.5231   50
      division   0.8642  110
      division   1.1767  194
      division   1.5041  302
#      division   1.9293  434
#      division   2.0065  590
#      division   2.0466  770
#      division   2.0877  974
#      division   2.4589 1202
      outer_grid   302

#     valence basis states
    valence      4  s   1.
    valence      3  p   6.
    valence      3  d  10.
```

```
#     ion occupancy
    ion_occ      4  s   0.
    ion_occ      3  p   6.
    ion_occ      3  d   9.

#  "First tier" - improvements: -211.42 meV to -9.17 meV
     ionic 4 p auto
     hydro 4 f 7.4
     hydro 3 s 2.6
     hydro 3 d 5
#     hydro 5 g 10.4
#  "Second tier" - improvements: -2.49 meV to -1.08 meV
#     hydro 4 p 5.8
#     hydro 3 d 2.7
#     hydro 6 h 15.2
#     hydro 5 s 10.8
#     hydro 4 f 16
#  "Third tier" - improvements: -0.50 meV to -0.21 meV
#     hydro 4 d 6
#     hydro 3 p 2.4
#     hydro 4 f 6.4
#     hydro 3 s 6.8
#     hydro 5 g 11.2
#  "Fourth tier" - improvements: -0.13 meV to -0.05 meV
#     hydro 4 p 7
#     hydro 4 s 4
#     hydro 6 h 14
#     hydro 4 d 8.6
#     hydro 5 f 15.2
```

## Cu3 – “environmental” Cu atoms that are furthest from the adsorbate

```
  species        Cu3
#
    nucleus      29
    mass         63.546
#
    l_hartree    4
#
    cut_pot      3.4  1.5  1.0
    basis_dep_cutoff    1e-4
#
    radial_base        47 4.9
    radial_multiplier  1
    angular_grids       specified
      division   0.5231   50
      division   0.8642  110
      division   1.1767  194
#      division   1.5041  302
#      division   1.9293  434
#      division   2.0065  590
#      division   2.0466  770
#      division   2.0877  974
#      division   2.4589 1202
      outer_grid   194

#     valence basis states
    valence      4  s   1.
    valence      3  p   6.
    valence      3  d  10.
#     ion occupancy
```

```
    ion_occ      4  s   0.
    ion_occ      3  p   6.
    ion_occ      3  d   9.

#  "First tier" - improvements: -211.42 meV to -9.17 meV
     ionic 4 p auto
#     hydro 4 f 7.4
#     hydro 3 s 2.6
#     hydro 3 d 5
#     hydro 5 g 10.4
#  "Second tier" - improvements: -2.49 meV to -1.08 meV
#     hydro 4 p 5.8
#     hydro 3 d 2.7
#     hydro 6 h 15.2
#     hydro 5 s 10.8
#     hydro 4 f 16
#  "Third tier" - improvements: -0.50 meV to -0.21 meV
#     hydro 4 d 6
#     hydro 3 p 2.4
#     hydro 4 f 6.4
#     hydro 3 s 6.8
#     hydro 5 g 11.2
#  "Fourth tier" - improvements: -0.13 meV to -0.05 meV
#     hydro 4 p 7
#     hydro 4 s 4
#     hydro 6 h 14
#     hydro 4 d 8.6
#     hydro 5 f 15.2
```

## Relaxed lattice parameters of bulk Be and Mg obtained using the SCAN functional and numerical "tight" basis sets

Beryllium: a = b = 2.264, c = 3.560
Magnesium: a = b = 3.190, c = 5.094
